# Supplementary material for: Study of charmonium production using decays to hadronic final states with the LHCb experiment
Source: arXiv:1910.08796 source file (2019-10-19)
Supplement: Supplementary file 1 [file appendix.tex]

\clearpage

\clearpage

\section{Invariant mass spectra before 2D and 3D fits}
\label{sec:notpure}

This section provides fits to the invariant mass spectra without 
using 2D or 3D fits to obtain pure two and three $\phi$ candidates. 
Figures~\ref{fig:ccall}, \ref{fig:twophiall} and~\ref{fig:threephiall} 
show invariant mass spectra for charmonia decays to $\phi \phi$, 
$\Bs \to \phi \phi$ and $\Bs \to \phi \phi \phi$, respectively. 
\begin{figure}[h]
\centering
\protect\protect\includegraphics[width=1\linewidth,height=10.cm]{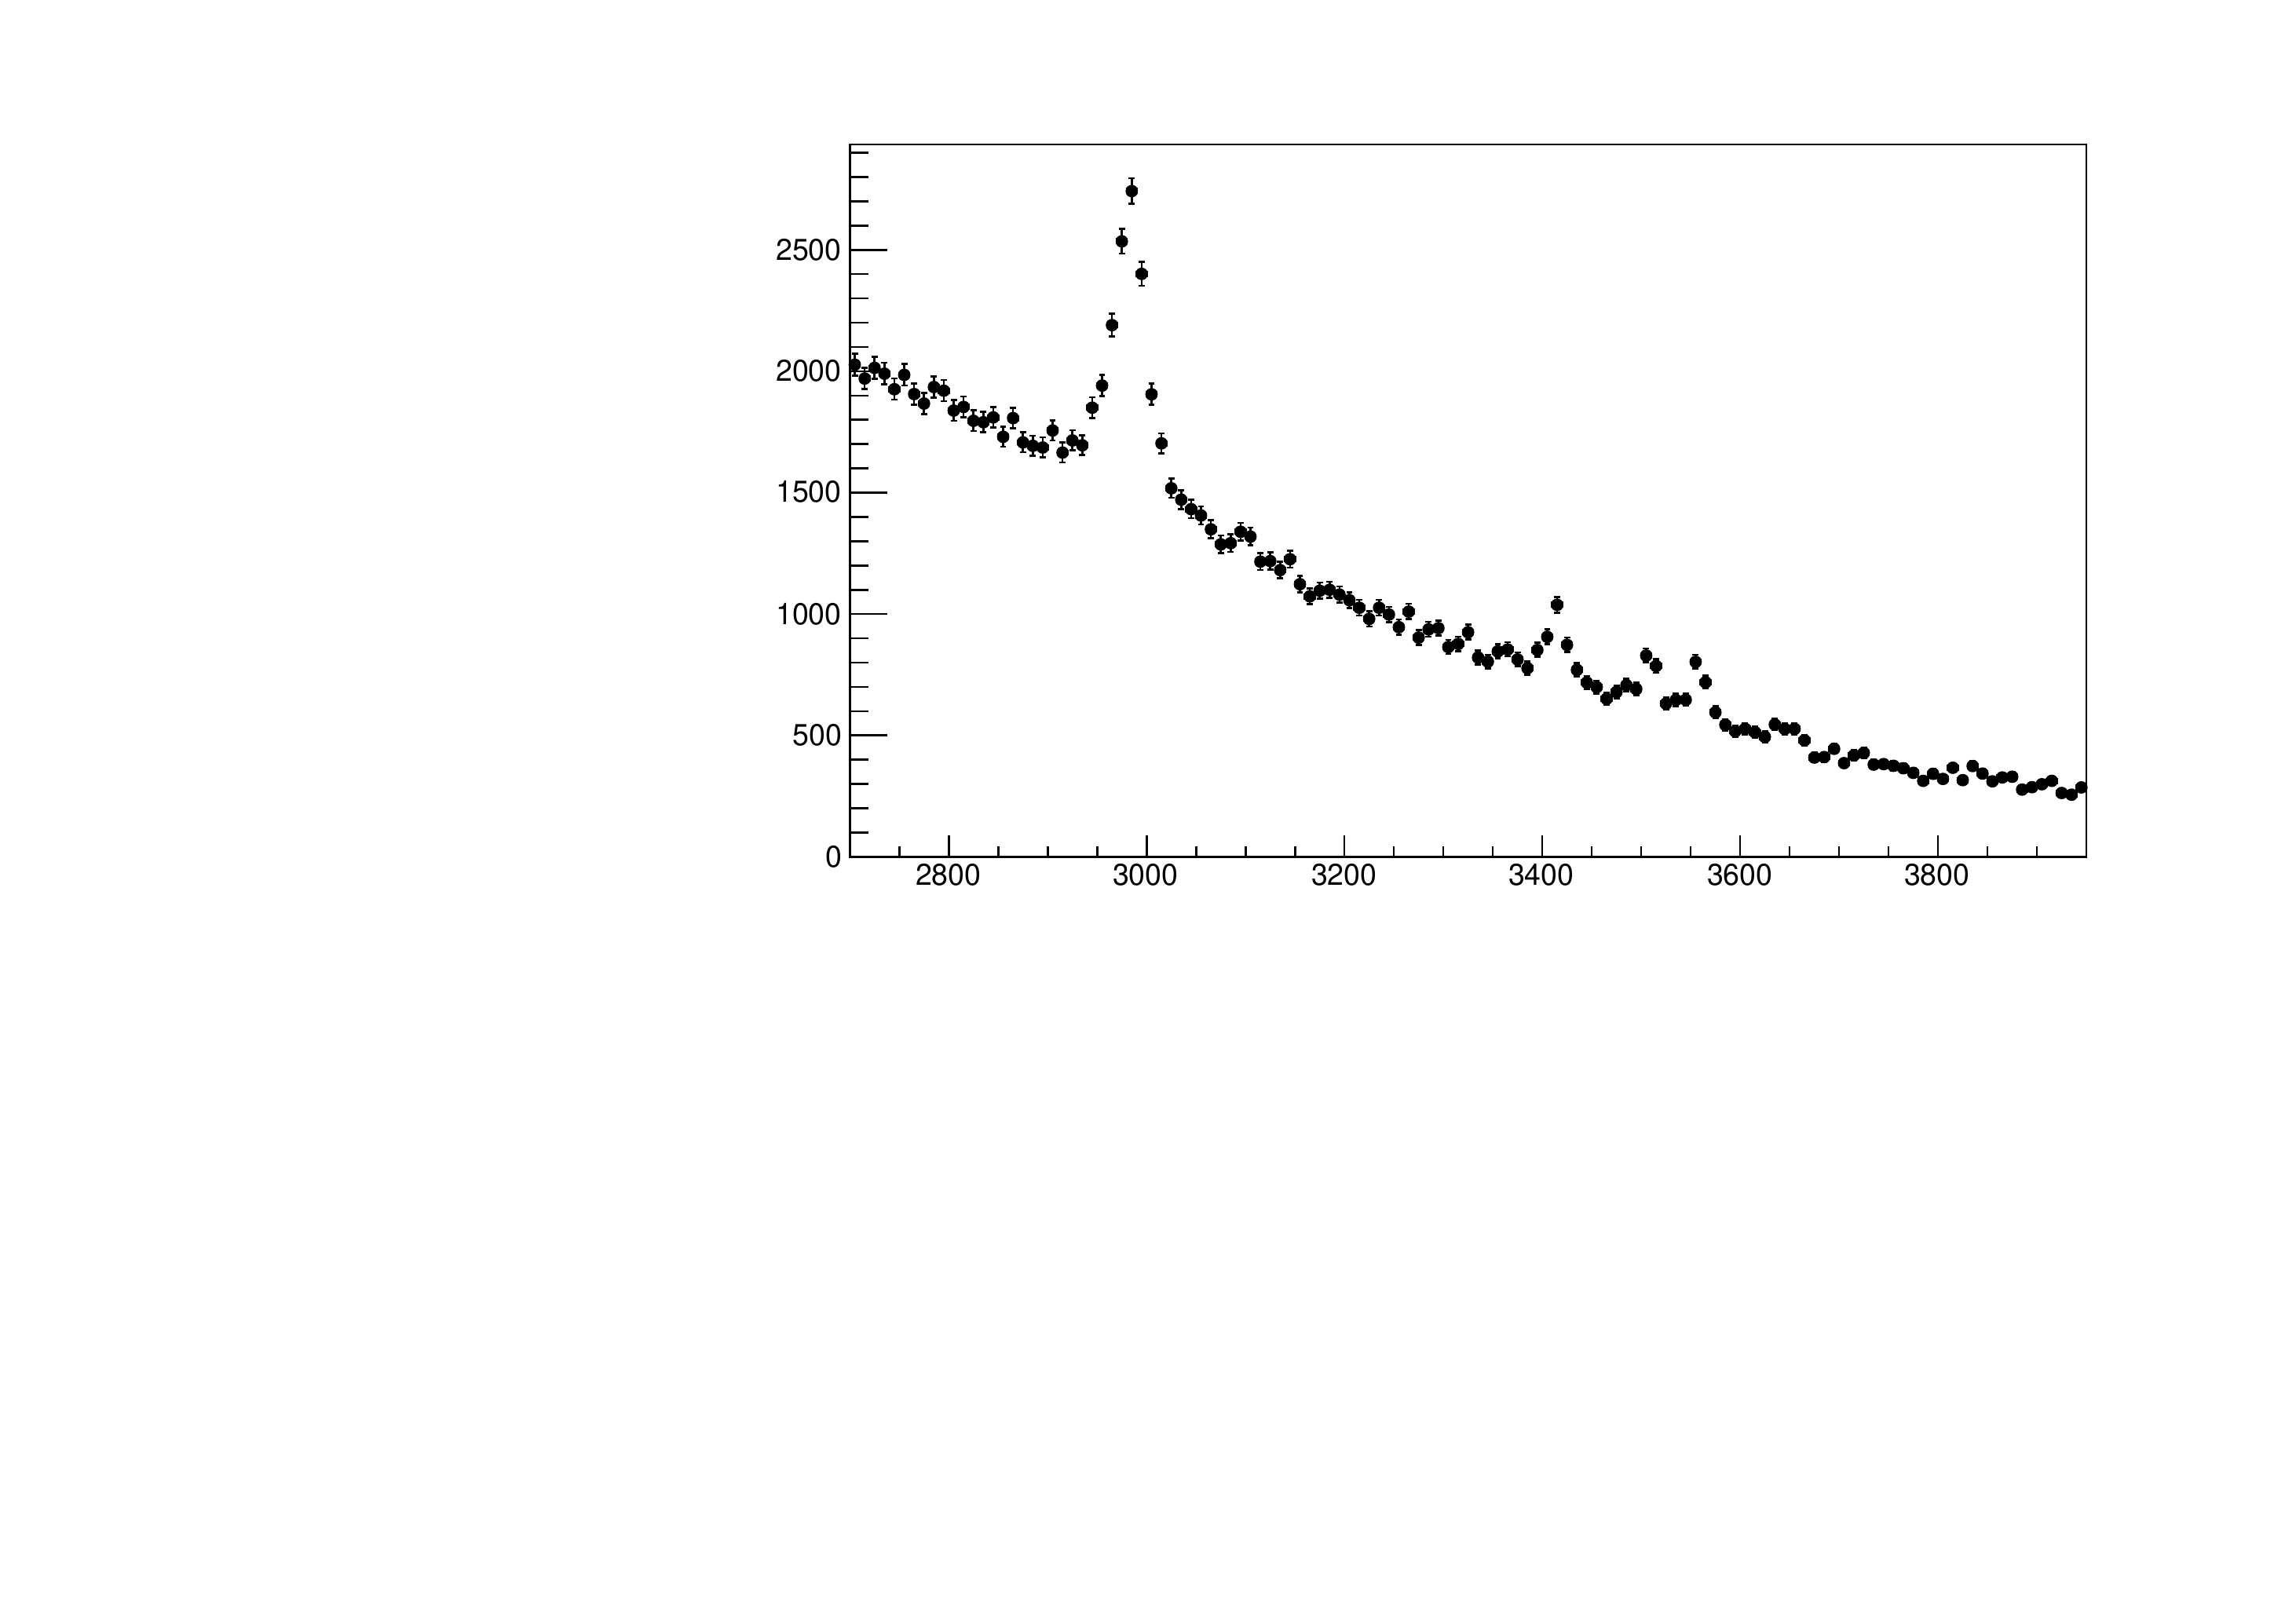}
                \put(-450,160){\rotatebox{90}{{Events/10 \mev}}}
                \put(-75,0) {{\mev}}
                \put(-150,230) {\lhcb preliminary}
                \put(-150,210) {3 fb$^{-1}$}
                \put(-310,220) {$\etac(1S)$}
                \put(-195,115) {\chiczero}
                \put(-170,100) {\chicone}
                \put(-155,95) {\chictwo}
                \put(-130,80) {$\etac(2S)$}
                \put(-240,0) {{$M( \phi \phi )$}}
\caption{Distribution of the $\phi \phi$ invariant mass for combined data sample, 
accumulated at $\sqs = 7 \tev$ and $\sqs = 8 \tev$. 
No 2D fit is performed 
\label{fig:ccall}}
\end{figure}
\begin{figure}[h]
\centering
\protect\protect\includegraphics[width=1\linewidth,height=8.cm]{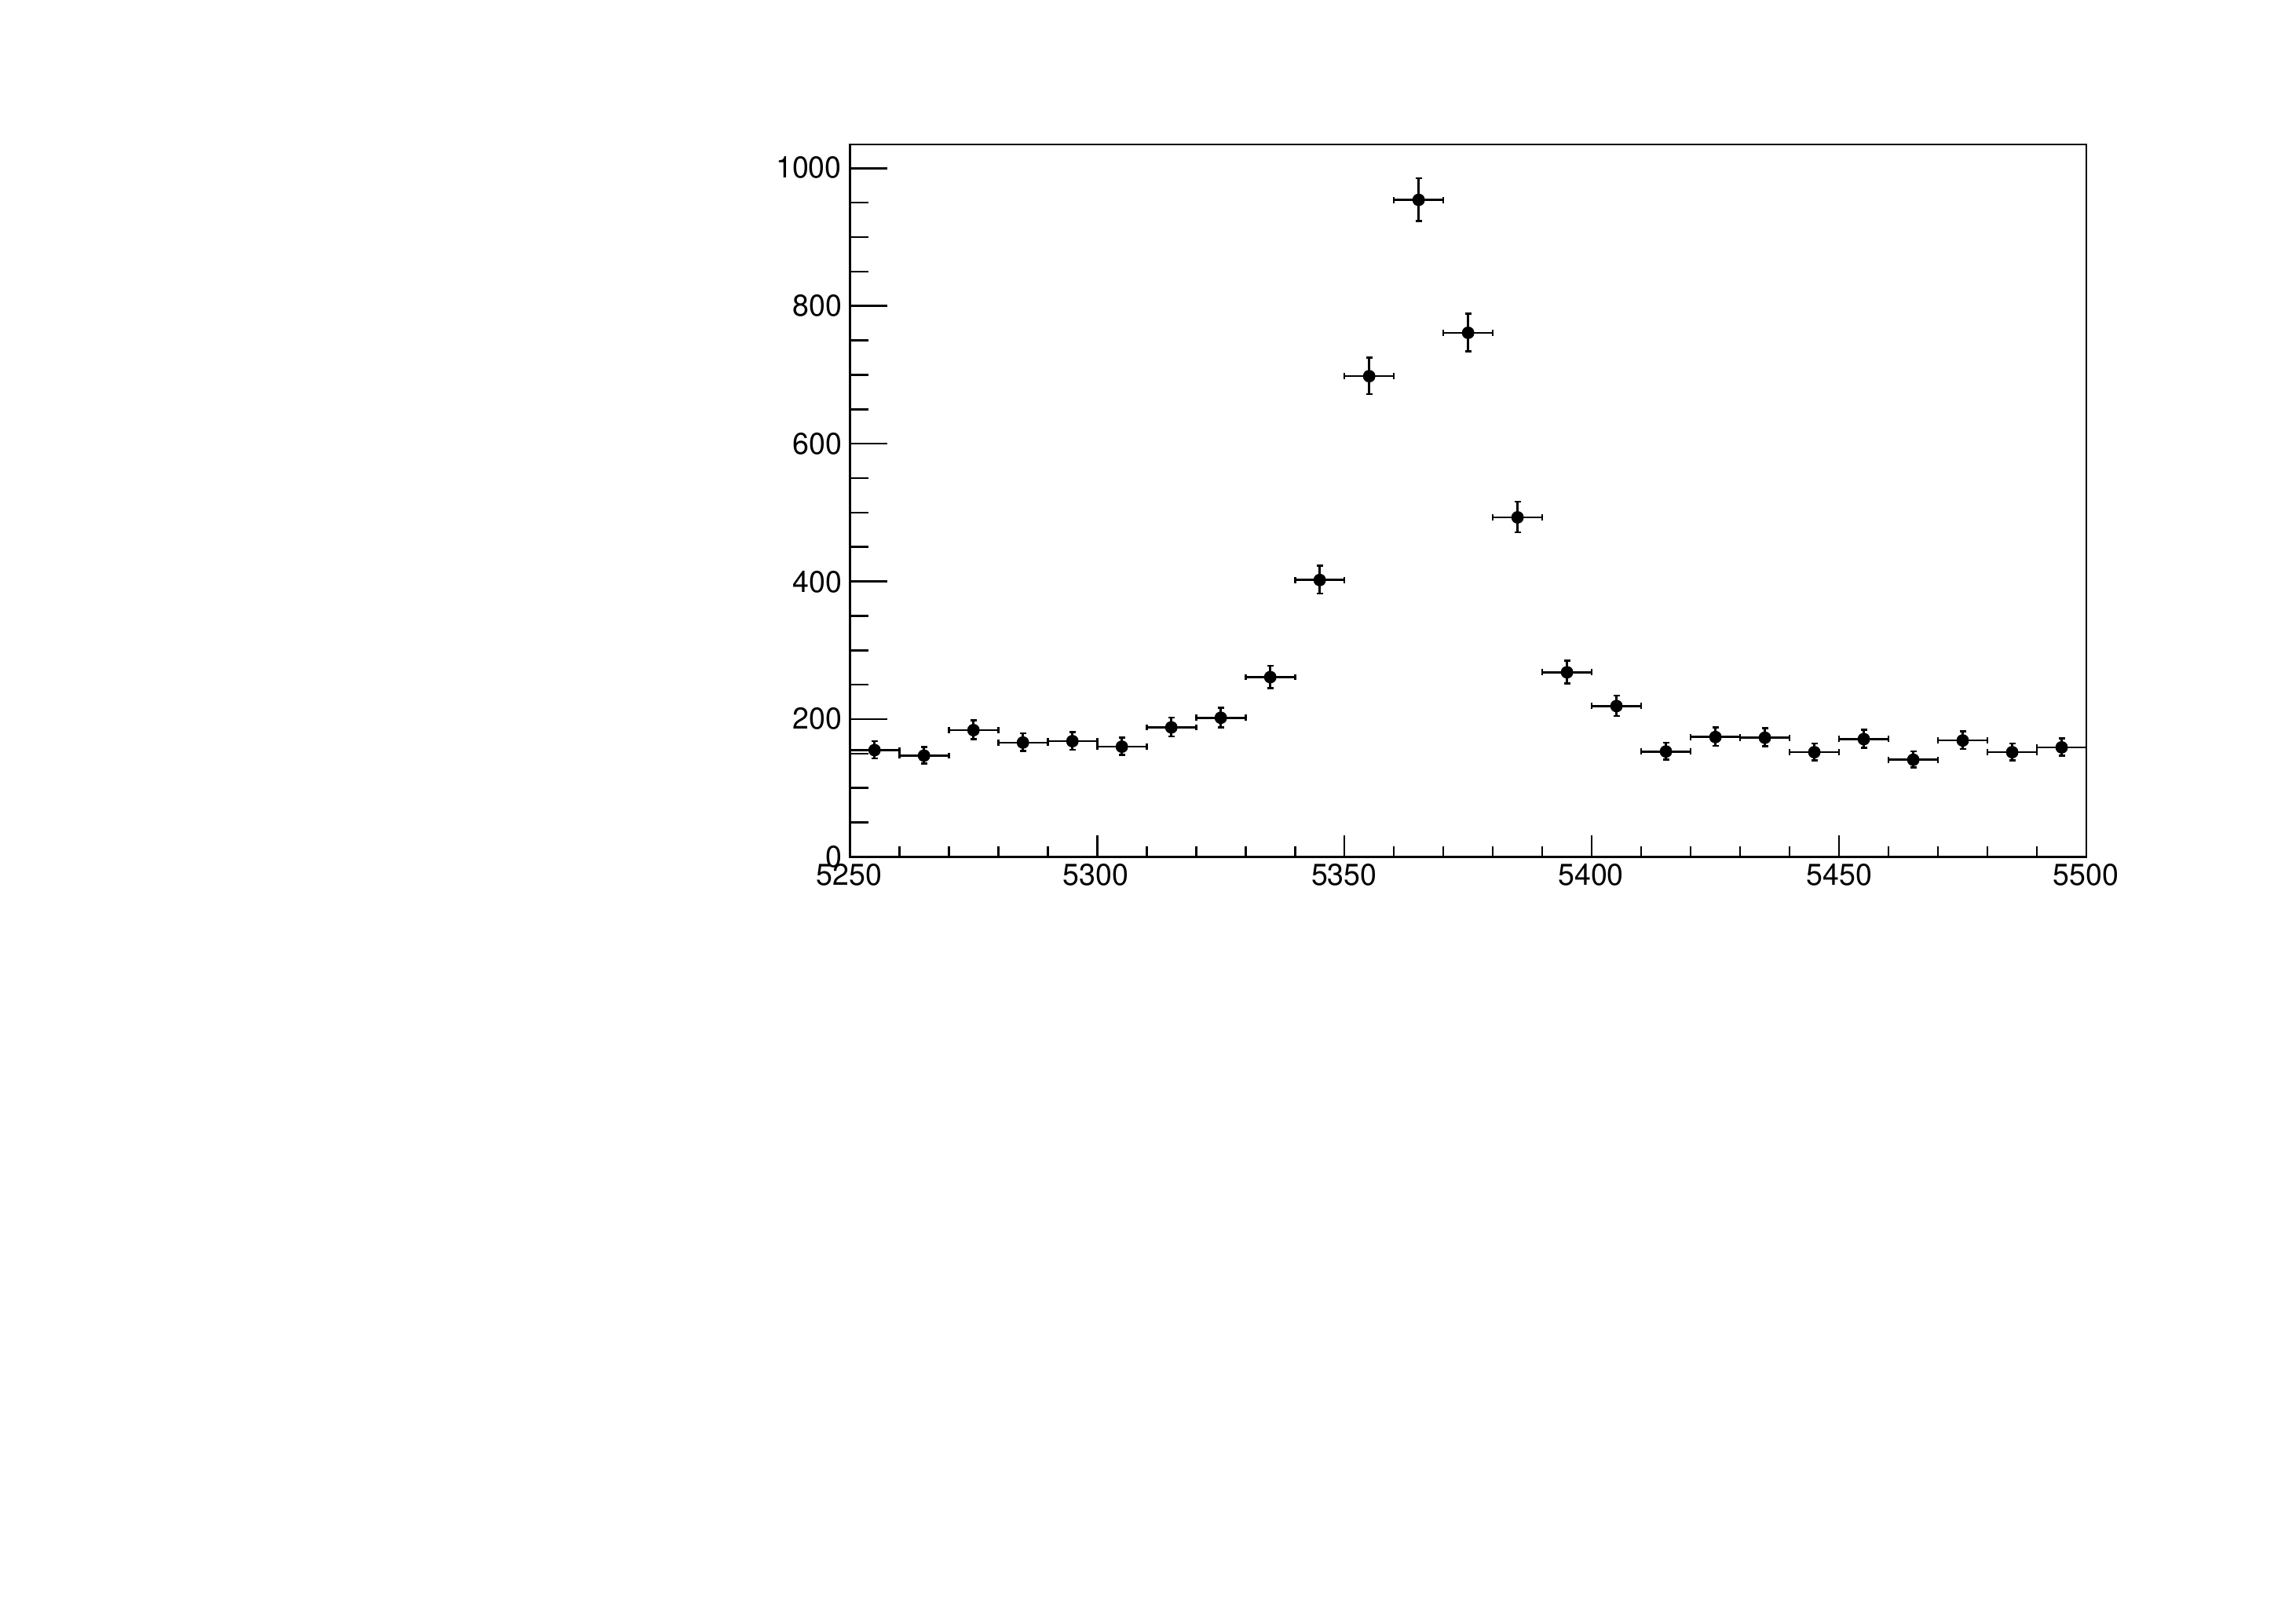}
                \put(-450,110){\rotatebox{90}{{Events/10 \mev}}}
                \put(-75,0) {{\mev}}
                \put(-150,180) {\lhcb preliminary}
                \put(-150,160) {3 fb$^{-1}$}
                \put(-240,0) {{$M( \phi \phi )$}}
\caption{Distribution of the $\phi \phi$ invariant mass for combined data sample, 
accumulated at $\sqs = 7 \tev$ and $\sqs = 8 \tev$. 
No 2D fit is performed 
\label{fig:twophiall}}
\end{figure}
\begin{figure}[h]
\centering
\protect\protect\includegraphics[width=1\linewidth,height=8.cm]{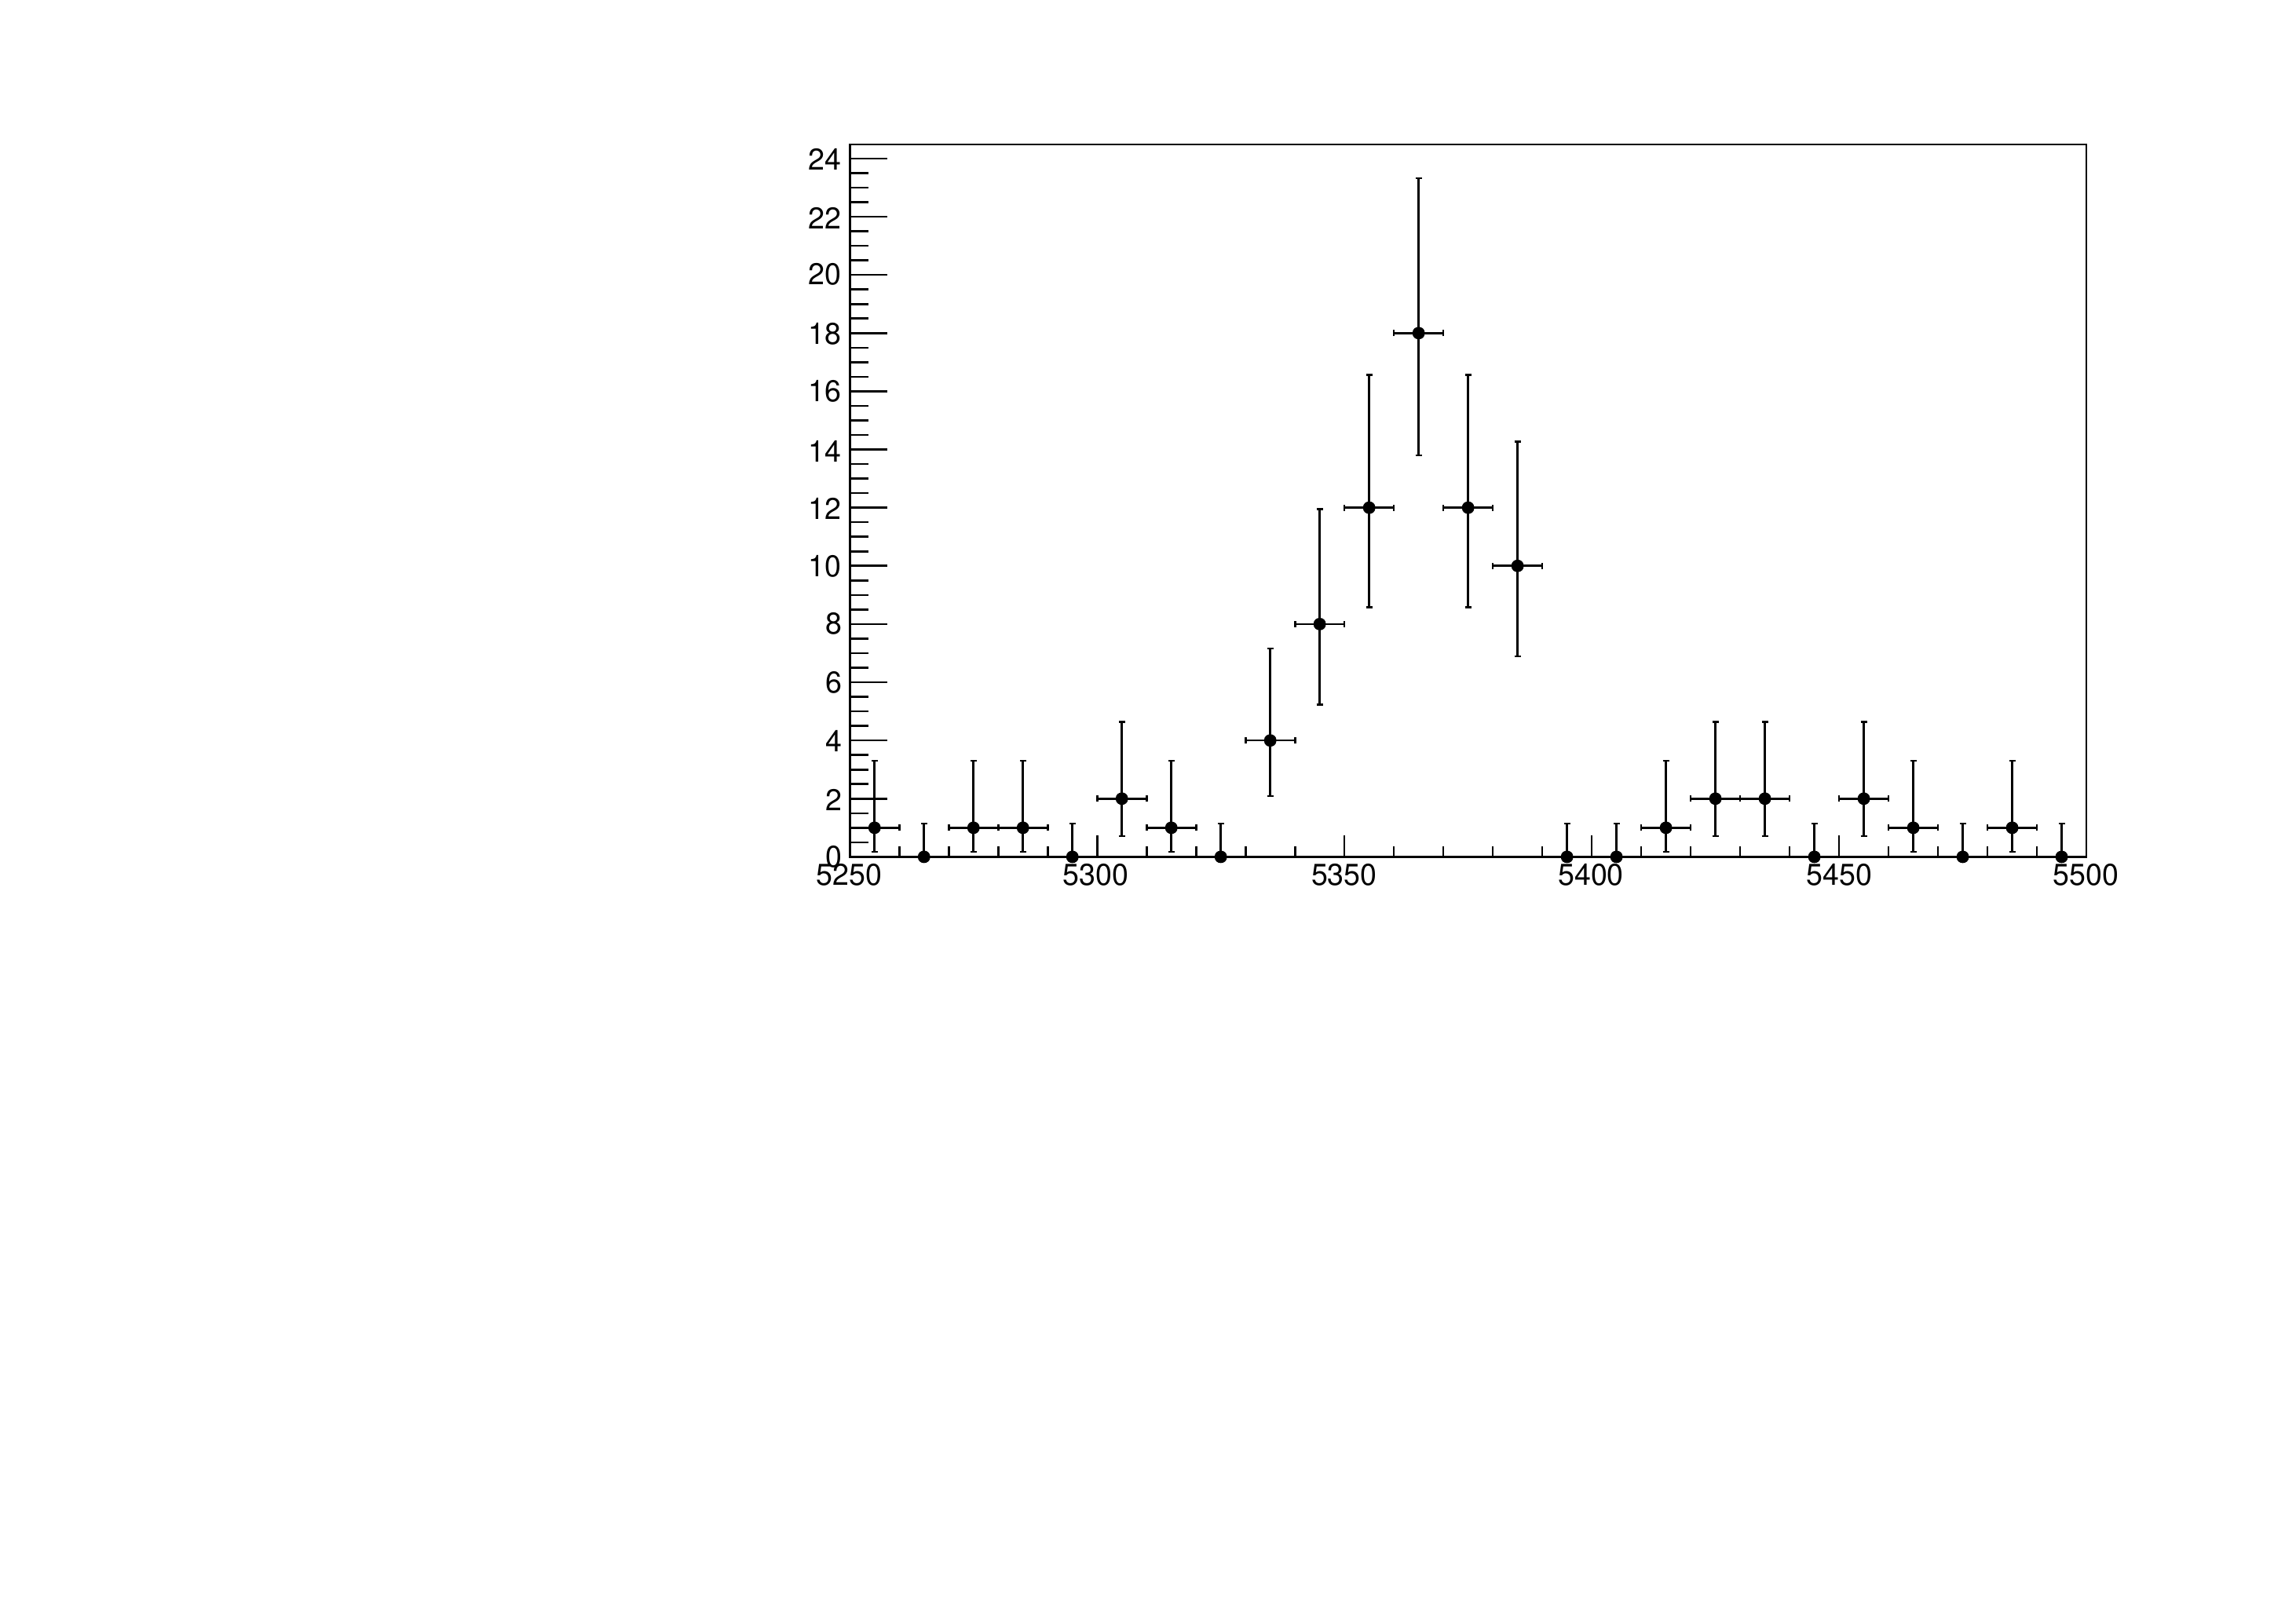}
                \put(-440,110){\rotatebox{90}{{Events/10 \mev}}}
                \put(-75,0) {{\mev}}
                \put(-150,180) {\lhcb preliminary}
                \put(-150,160) {3 fb$^{-1}$}
                \put(-240,0) {{$M( \phi \phi \phi )$}}
\caption{Distribution of the $\phi \phi \phi$ invariant mass for combined data sample, 
accumulated at $\sqs = 7 \tev$ and $\sqs = 8 \tev$. 
No 3D fit is performed 
\label{fig:threephiall}}
\end{figure}

Comparing the plots with those obtained using 2D or 3D fits, one observes 
significant or dominant $\phi \phi$- and $\phi \phi \phi$-components in charmonia or \Bs decays to $\phi$ mesons.

\clearpage

\section{Cross-check for charmonia production and masses: shift by half a bin size}
\label{sec:bincheck}

Table~\ref{tab:bincheckm} compares the results for charmonia mass and $\Gamma_{\etac(1S)}$ values obtained 
in section~\ref{sec:masses} to those obtained with the shift by half a bin of the invariant mass 
distribution. 
\begin{table}[h]
\centering
\begin{tabular}{l|c|c}
              & Measured value, \mev (\mev) & Shift with respect    \\ 
              &                             & to the measured value, \mev \\ \hline
$M_{\etac(1S)}$ & $2982.81 \pm 0.99 \pm 0.45$ & $0.56$ \\ \hline
$M_{\chiczero}$ & $3412.99 \pm 1.91 \pm 0.62$ & $- 0.88$ \\ \hline
$M_{\chicone}$  & $3508.38 \pm 1.91 \pm 0.66$ & $2.40$ \\ \hline
$M_{\chictwo}$  & $3557.29 \pm 1.71 \pm 0.66$ & $2.13$ \\ \hline
$M_{\etac(2S)}$ & $3636.35 \pm 4.06 \pm 0.69$ & $- 0.83$ \\ \hline
$\Gamma_{\etac(1S)}$ & $31.35 \pm 3.51 \pm 2.00$ & $- 1.24$ 
\end{tabular}
\caption{Cross-check for charmonia mass and $\Gamma_{\etac(1S)}$ values against a shift by half a bin of the invariant mass 
distribution
\label{tab:bincheckm}}
\end{table}

Table~\ref{tab:bincheckdm} compares the results for charmonia mass difference values obtained 
in section~\ref{sec:masses} to those obtained with the shift by half a bin of the invariant mass 
distribution. 
\begin{table}[h]
\centering
\begin{tabular}{l|c|c}
                             & Measured value, \mev & Shift with respect    \\ 
                             &                        & to the measured value, \mev \\ \hline
$M_{\chicone} - M_{\chiczero}$  & $95.38 \pm 2.71 \pm 0.11$ & $3.28$ \\ \hline
$M_{\chictwo} - M_{\chiczero}$  & $144.28 \pm 2.59 \pm 0.17$ & $3.01$ \\ \hline
$M_{\etac(2S)} - M_{\etac(1S)}$ & $653.54 \pm 4.22 \pm 0.42$ & $- 1.38$ 
\end{tabular}
\caption{Cross-check for charmonia mass difference values against a shift by half a bin of the invariant mass 
distribution
\label{tab:bincheckdm}}
\end{table}
The results are found to be stable within the statistical uncertainties.

\section{Choice of kaon identification and flight distance selection criteria}
\label{sec:selection}

Almost all selection had to be fixed already at the trigger/stripping level to limit the corresponding
bandwidth. 
Exceptions are kaon identification and distance between primary and secondary vertices.
The method applied to extract the signal does not seem to require strong kaon identification, since narrow $\phi$
peaks are selected. The results are checked for stability against ProbNNk cut value variation, and the
results are similar within statistical uncertainty. 
For ProbNNk 0.05, 0.10 and 0.15 values:
\begin{align*}
N_\chiczero / N_{\etac(1S)} & = 0.140, 0.138, 0.136, \\
N_\chicone / N_{\etac(1S)} & = 0.067, 0.073, 0.078, \\
N_\chictwo / N_{\etac(1S)} & = 0.081, 0.092, 0.098, \\
N_{\etac(2S)} / N_{\etac(1S)} & = 0.045, 0.053, 0.054.
\end{align*}
The distance between the primary and secondary vertices is retained at minimum possible value, and
contribution from prompt production estimated. Taking $\etac(1S)$ as an example, and using the
production from the ppbar analysis, the ratio of the prompt contribution to the etac from b-decays
(without trigger, flight distance cut and neither IP cuts) is estimated as $\approx 40$. 
Using simulated
sample, the trigger, and the two important cuts give a factor of $1.5 \times 10^{-4}$. 
This gives an estimated contamination by prompt charmonia at the level of $\sim 0.6 \%$.

\clearpage

\section{Example of the 2D fit in bin of the $\phi \phi$ invariant mass}
\label{sec:binfit}

Fig.~\ref{fig:twophibin} illustrates an example of the 2D fit in the bin of the $\phi \phi$ invariant mass.
\begin{figure}[h]
\centering
\protect\protect\includegraphics[width=0.95\linewidth]{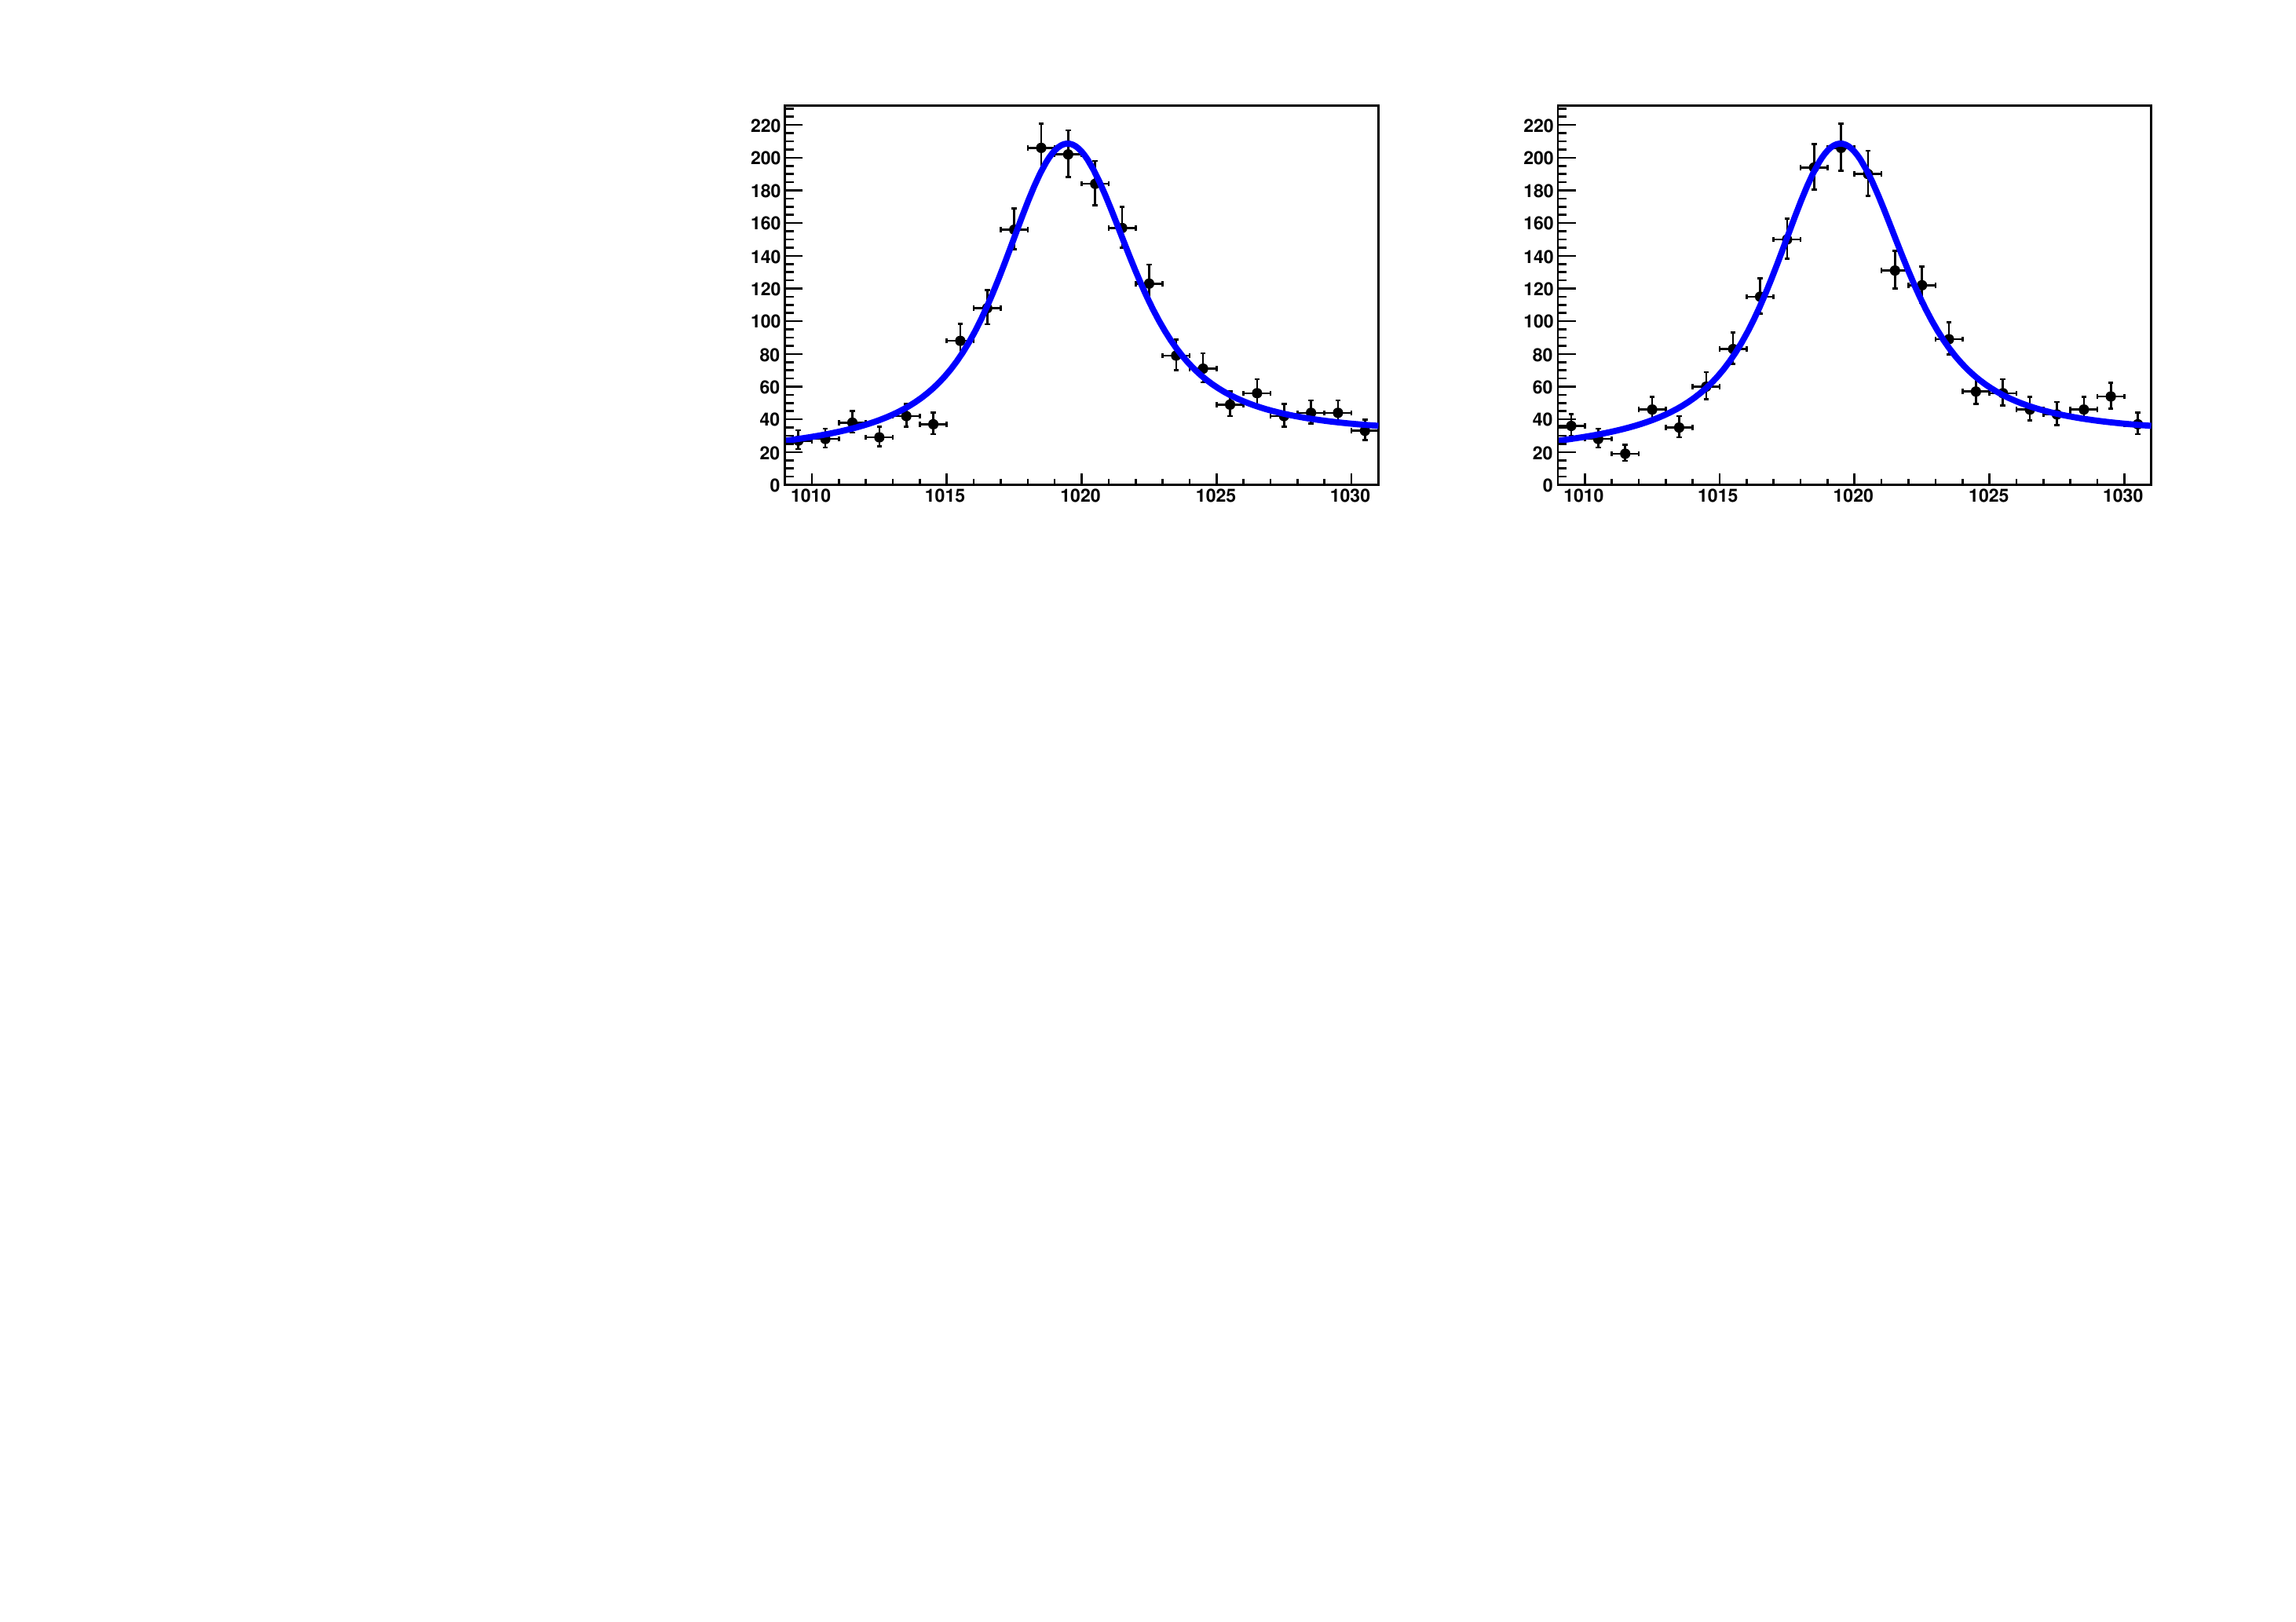}
%                \put(-290,100){\rotatebox{90}{\small{\PDF}}}
%                \put(-150,-3) {\small{$f_T$}}
                \put(-185,108) {{\small{\lhcb preliminary}}}
                \put(-185,95) {{\small{3 fb$^{-1}$}}}
                \put(-400,108) {{\small{\lhcb preliminary}}}
                \put(-400,95) {{\small{3 fb$^{-1}$}}}
\caption{Example of the 2D fit in the bin of the $\phi \phi$ invariant mass. Projections of the 2D fit are shown.}
\label{fig:twophibin}
\end{figure}
The contribution of $953 \pm 69$, $376 \pm 50$ and $138 \pm 50$,
for the $\phi \phi$,  $\phi \Kp \Km$ and  $\Kp \Km \Kp \Km$ modes, respectively, 
is suggested by the fit.
