# Supplementary material for: Study of charmonium production using decays to hadronic final states with the LHCb experiment
Source: arXiv:1910.08796 source file (2019-10-19)
Supplement: Supplementary file 2 [file appendix.tex]

% $Id: appendix.tex 116636 2018-01-22 16:05:04Z fwilson $
% ===============================================================================
% Purpose: appendix to the standard template: standard symbol alises from Ulrik
% Author: Tomasz Skwarnicki
% Created on: 2009-09-24
% ===============================================================================

\clearpage

{\noindent\normalfont\bfseries\Large Appendices}

\appendix
\section{Cross-check: shifts of peak positions}

The comparison of peaks positions shifts from data with applying and without applying momentum scale calibration and from MC is shown on Fig.~\ref{fig:shifts_vs_m_scaled}. The shifts from data are extracted from simultaneous fit in 7 bins of $t_z$. No significant effect of momentum scale calibration is observed.
\begin{figure}[ht]
\centering
\protect\protect\protect\includegraphics[width=0.6\textwidth]{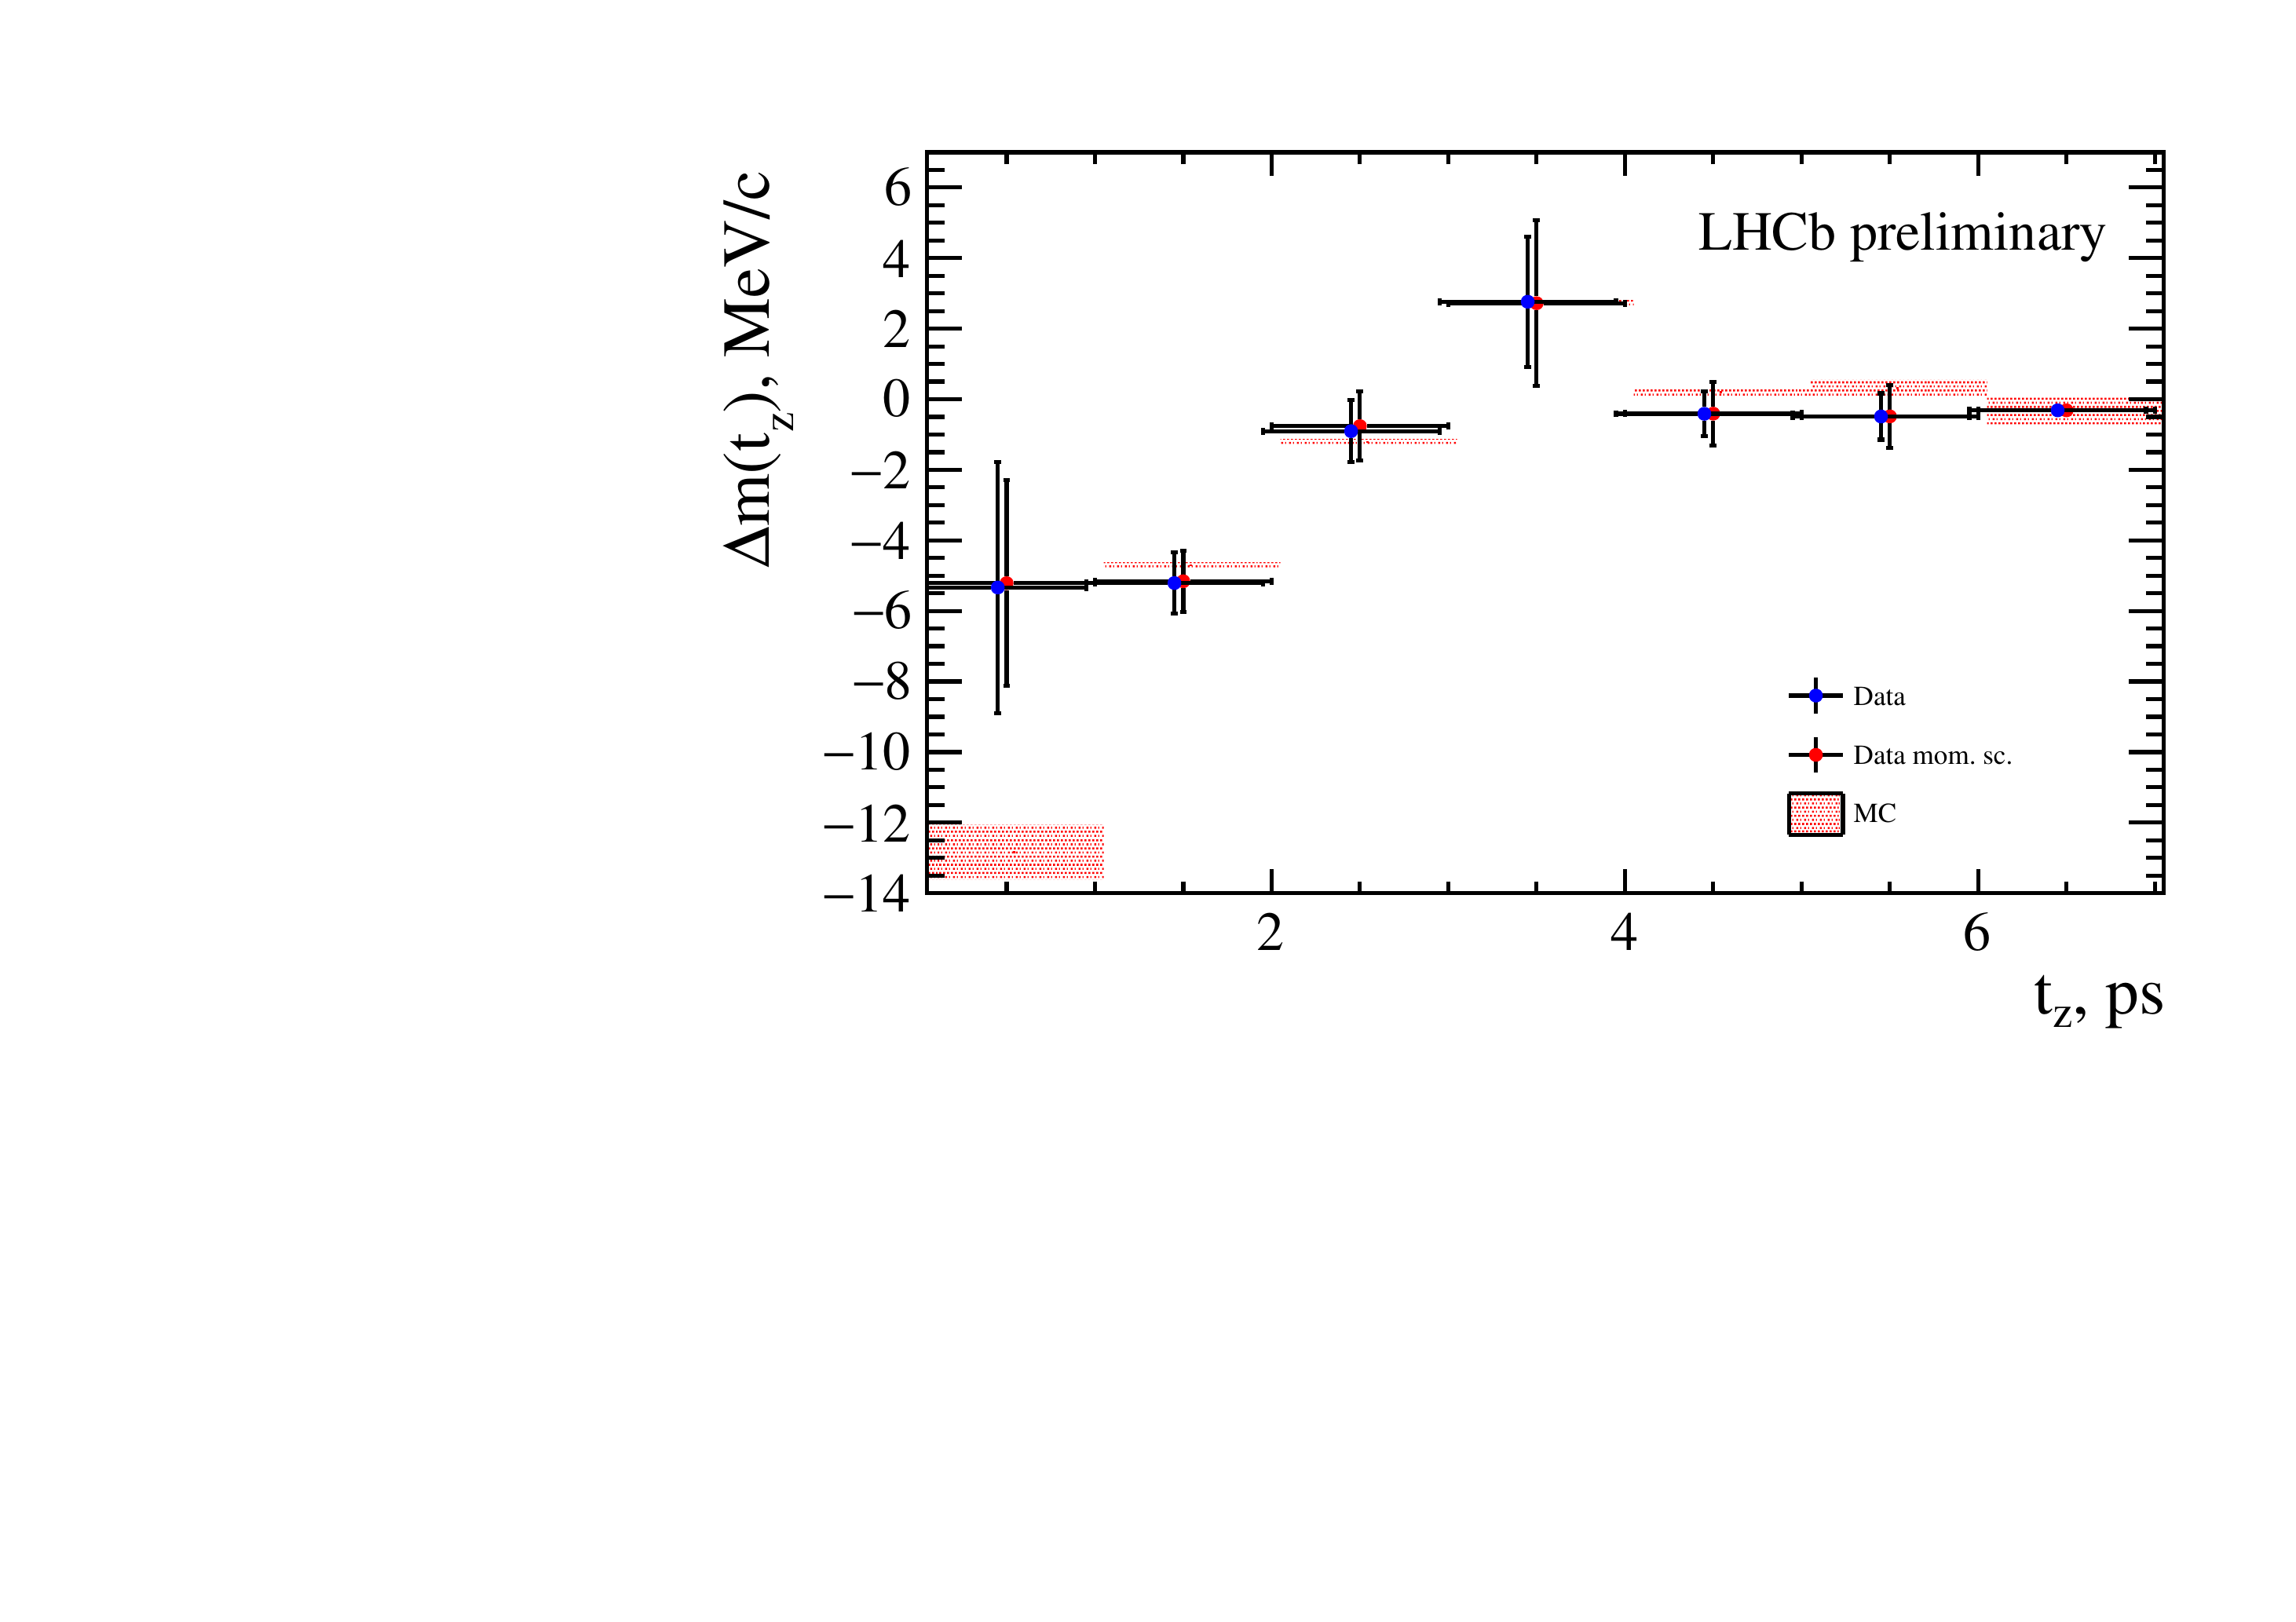}
\put(-80,5){\colorbox{shadecolor}{\small{$t_z$ bin number}}}
\caption{Peaks positions shifts from \pt-integrated data sample with applying momentum scale calibration (blue points), without applying momentum scale calibration (red points) and from MC (red boxes) as function of $t_z$ bin number} 
\label{fig:shifts_vs_m_scaled}
\end{figure}

The comparison of peaks positions shifts for \etac and \jpsi from MC is shown on Fig.~\ref{fig:shifts_vs_m_scaled}. No significant difference between \etac and \jpsi shifts observed.
\begin{figure}[ht]
\centering
\protect\protect\protect\includegraphics[width=0.6\textwidth]{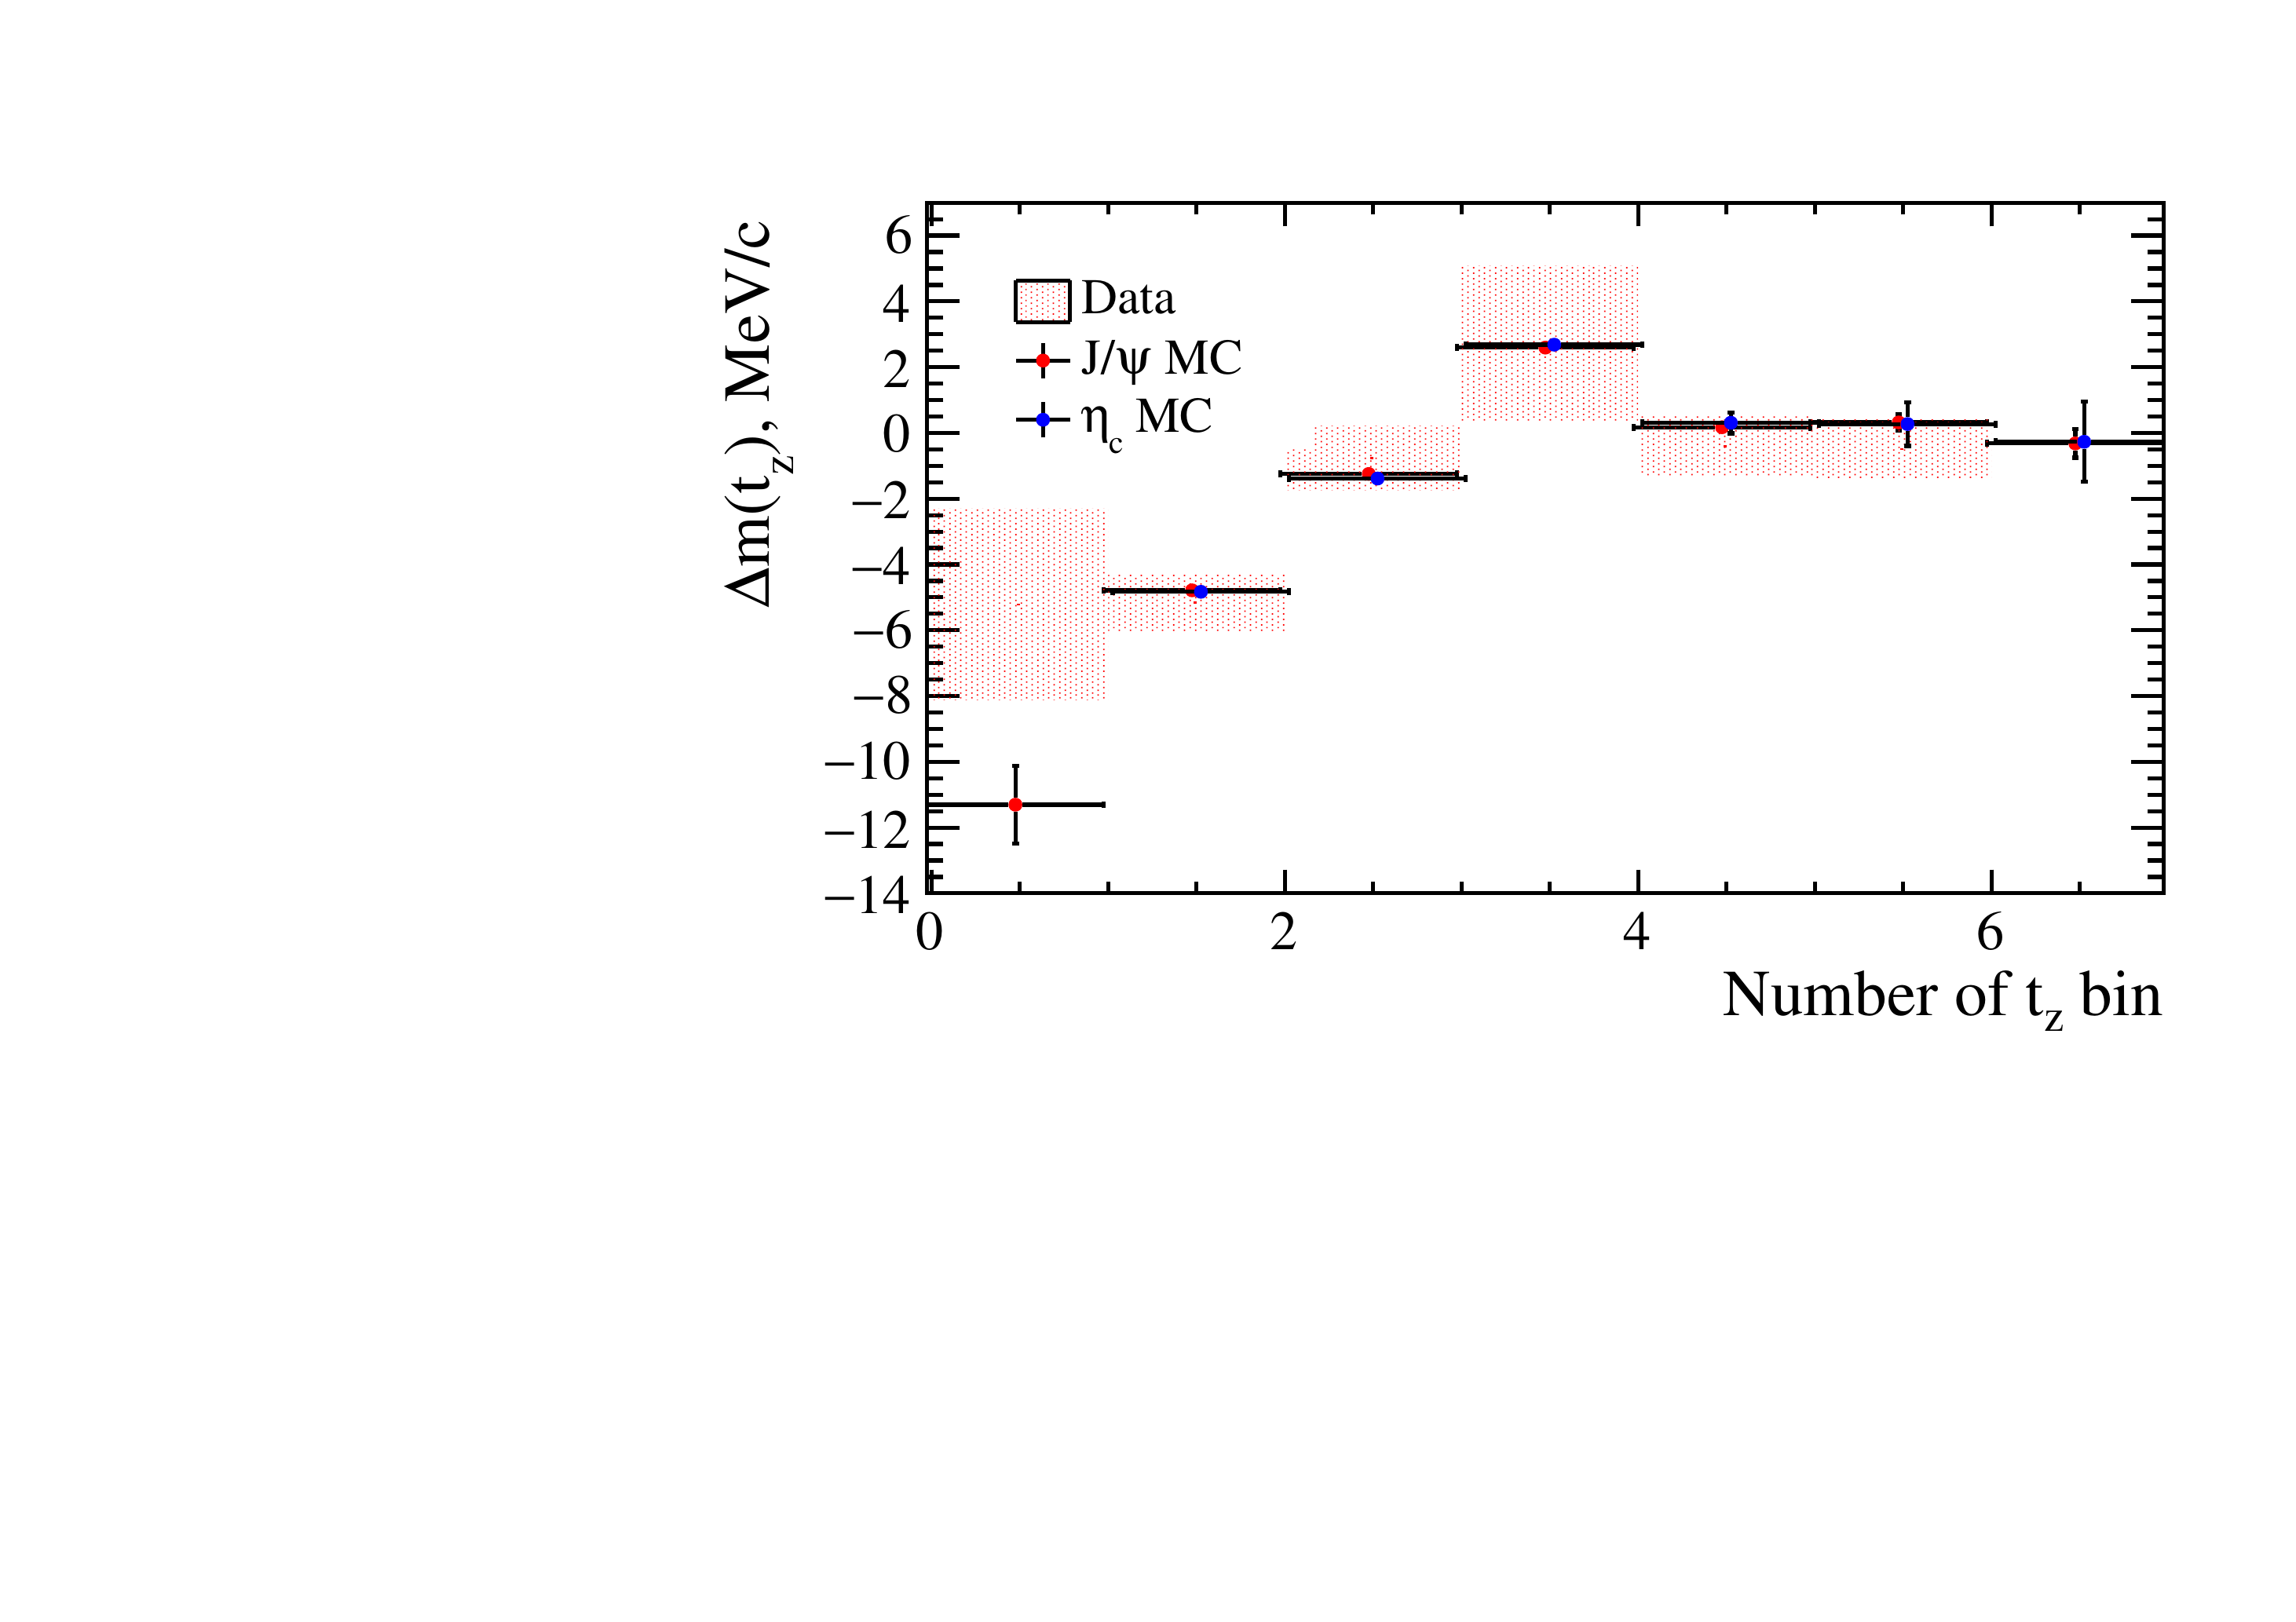}
\caption{Peaks positions shifts for \etac (blue points) and \jpsi (red points) separately from \pt-integrated MC sample.} 
\label{fig:shifts_etac_vs_jpsi}
\end{figure}

The comparison of peaks positions shifts from MC in bins of \pt is shown on Fig.~\ref{fig:shifts_vs_PT}. 
No significant \pt-dependence of shifts is observed.
\begin{figure}[ht]
\centering
\protect\protect\protect\includegraphics[width=0.6\textwidth]{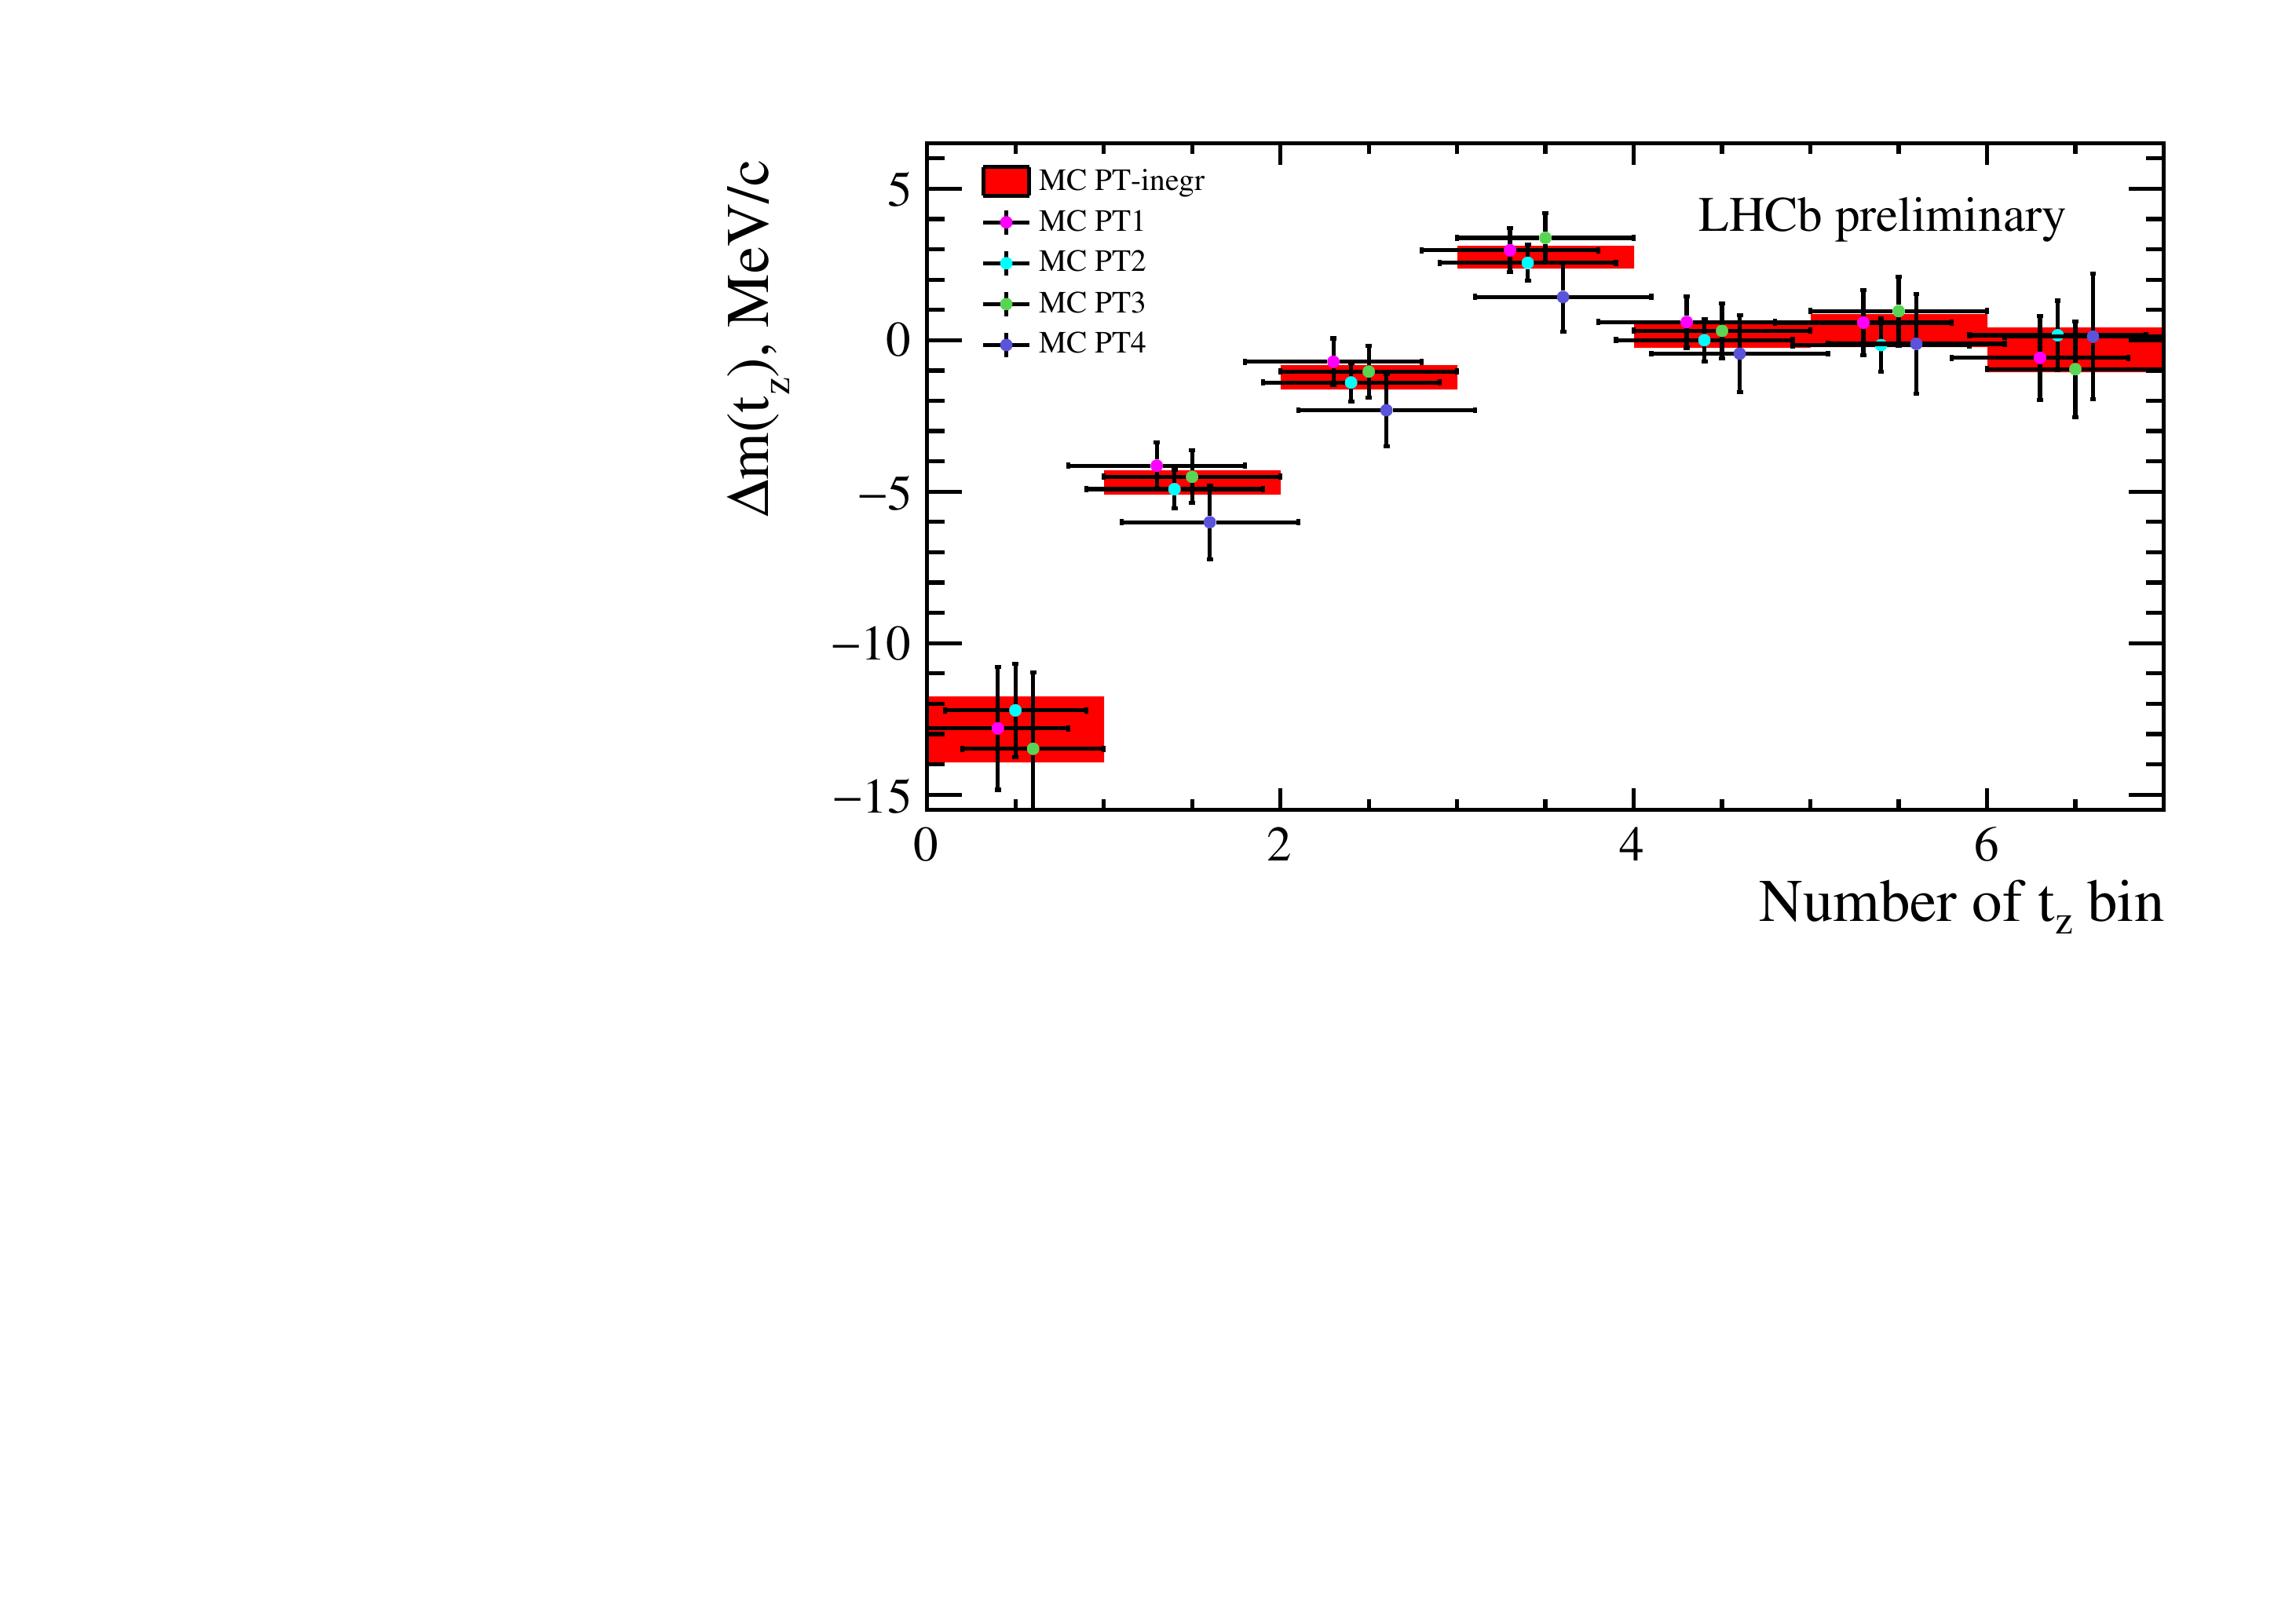}
\caption{Peaks positions shifts in \pt-bins (points) from MC and from \pt-integrated MC sample (red boxes)}
\label{fig:shifts_vs_PT}
\end{figure}

\newpage
\section{Cross-check: comparison of \jpsi and \etac masses from fits to prompt and \bquark-decays samples}
\label{app:massChecksTzCut}

The mass of \jpsi and the \jpsi and \etac mass difference for \tzcut is cross-checked by performing individual fits to prompt and \bquark-decays samples in \pt-bins. In each fit the mass of \jpsi and \jpsi and \etac mass difference are free fit parameters.

Table~\ref{tab:massComparison} summarises results of fits to prompt and \bquark-decays samples in bins of \pt, results of simultaneous fits to both prompt and \bquark-decays samples in bins of \pt, results of fits to \pt-integrated sample and the result of simultaneous fit to prompt and \bquark-decays samples of all \pt-bins. The obtained values of masses are consistent with each other within uncertainties.

\begin{table}[ht]
\centering
\small
\begin{tabular}{c|c|c|c}
Fit type    		 & \pt, \gevc    & $M_{\jpsi}-M_{\etac}, \mev$ & $M_{\jpsi}, \mev$  \\ \hline 
\bquark-decays 		& 6.5 - 8.0 	 &  $115.0\pm2.7$ & $3097.0\pm0.2$ \\ 
\bquark-decays 		& 8.0 - 10.0 	 &  $113.7\pm1.5$ & $3097.0\pm0.2$ \\ 
\bquark-decays 		& 10.0 - 12.0    &  $116.3\pm2.4$ & $3097.1\pm0.2$ \\  
\bquark-decays 		& 12.0 - 14.0 	 &  $112.5\pm2.9$ & $3096.9\pm0.3$ \\ \hline
prompt 				& 6.5 - 8.0 	 &  $108.0\pm4.0$ & $3097.0\pm0.9$ \\ 
prompt 				& 8.0 - 10.0 	 &  $110.0\pm2.6$ & $3096.4\pm0.6$ \\ 
prompt 				& 10.0 - 12.0    &  $112.5\pm2.9$ & $3097.6\pm0.7$ \\  
prompt 				& 12.0 - 14.0    &   $99.6\pm5.2$ & $3095.2\pm1.6$ \\ \hline
simultaneous		& 6.5 - 8.0 	 &  $112.2\pm2.1$ & $3097.0\pm0.2$ \\ 
simultaneous		& 8.0 - 10.0 	 &  $112.2\pm1.3$ & $3097.0\pm0.2$ \\ 
simultaneous		& 10.0 - 12.0    &  $114.6\pm1.8$ & $3097.2\pm0.2$ \\  
simultaneous		& 12.0 - 14.0    &  $106.5\pm2.2$ & $3096.9\pm0.3$ \\ \hline 
simultaneous to all samples&         &  $112.3\pm0.9$ & $3097.0\pm0.1$ \\
in all \pt-bins				& & & \\ \hline
simultaneous		& 6.5 - 14.0 	 &  $112.6\pm0.9$ & $3097.0\pm0.1$ \\ 
\end{tabular} 
\caption{Comparison of the \etac and \jpsi mass difference and \jpsi mass as obtained from various fit types using prompt and \bquark-decays samples from \tzcut.}
\label{tab:massComparison}
\end{table} 

\newpage
\section{Tables of relative \pt-differential \etac production}
\label{app:sigmaRel}

\subsection{Prompt}
The results on total relative \etac prompt production from \tzfit and \tzcut are shown in Table ~\ref{tab:relPromptTable}. The first uncertainty is statistical, the second is systematic, and  the last uncertainty is related to $\BR_{\JpsiToPpbar}$ and $\BR_{\EtacToPpbar}$.
\begin{table}[ht]
\centering
\small
\begin{tabular}{c|c|c}
\pt, \gevc      & \multicolumn{2}{c}{$d\sigma^{prompt}_{\etac}/d\sigma^{prompt}_{\jpsi}$} \\ \hline
   & \tzfit & \tzcut \\ \hline
6.5 - 14.0 		&  1.88 $\pm$ 0.16 $\pm$ 0.14 $\pm$ 0.21  & 1.69 $\pm$ 0.15 $\pm$ 0.10 $\pm$ 0.18
\end{tabular} 
\caption{The total relative \etac prompt production}
\label{tab:relTotalPromptTable}
\end{table}

\subsection{From \bquark-decays}
The results on total relative \etac production in inclusive \bquark-decays from \tzfit and \tzcut are shown in Table ~\ref{tab:relTotalSecondaryTable}. The first uncertainty is statistical, the second is systematic, the last uncertainty is related to $\BR_{\JpsiToPpbar}$ and $\BR_{\EtacToPpbar}$.
\begin{table}[ht]
\centering
\small
\begin{tabular}{c|c|c}
\pt, \gevc     & \multicolumn{2}{c}{$d\sigma^{\bquark-decays}_{\etac}/d\sigma^{\bquark-decays}_{\jpsi}$} \\ \hline 
    & \tzfit & \tzcut \\ \hline
6.5 - 14.0 		& 0.47 $\pm$ 0.04 $\pm$ 0.03 $\pm$ 0.05 & 0.48 $\pm$ 0.03 $\pm$ 0.03 $\pm$ 0.05   
\end{tabular} 
\caption{The total relative \etac production in inclusive \bquark-decays}
\label{tab:relTotalSecondaryTable}
\end{table}

\newpage
\section{Tables of absolute \pt-differential \etac production}
\label{app:sigmaAbs}

\subsection{Prompt}
The results on total \etac prompt production cross-section from \tzfit and \tzcut are shown in Table ~\ref{tab:TotalPromptTable}. The first uncertainty is statistical, the second is systematic and the last uncertainty is related to $\BR_{\JpsiToPpbar}$ and $\BR_{\EtacToPpbar}$ and \jpsi production measurement.
\begin{table}[ht]
\centering
\small
\begin{tabular}{c|c|c}
\pt, \gevc     & \multicolumn{2}{c}{$\sigma^{prompt}_{\etac}$, \mub}     \\ \hline 
   & \tzfit & \tzcut \\ \hline
6.5 - 14.0   & 1.41 $\pm$ 0.12 $\pm$ 0.10 $\pm$ 0.16  & 1.26 $\pm$ 0.11 $\pm$ 0.08 $\pm$ 0.14
\end{tabular} 
\caption{The total \etac prompt production cross-section}
\label{tab:TotalPromptTable}
\end{table}

The results on \pt-differential \etac prompt production cross-section from \tzfit and \tzcut are shown in Table ~\ref{tab:PromptTable}. The first uncertainty is statistical, the second is uncorrelated between bins systematic uncertainty, the third is correlated between bins systematic uncertainty, the last uncertainty is related to $\BR_{\JpsiToPpbar}$ and $\BR_{\EtacToPpbar}$ and \jpsi production measurement.

\clearpage

\subsection{From \bquark-decays}
The results on total \etac production cross-section in inclusive \bquark-decays from \tzfit and \tzcut are shown in Table ~\ref{tab:TotalSecondaryTable}. The first uncertainty is statistical, the second is systematic and the last uncertainty is related to $\BR_{\JpsiToPpbar}$ and $\BR_{\EtacToPpbar}$ and \jpsi production measurement.
\begin{table}[ht]
\centering
\small
\begin{tabular}{c|c|c}
\pt, \gevc     & \multicolumn{2}{c}{$\sigma^{\bquark-decays}_{\etac}$, \nb}     \\ \hline 
   & \tzfit & \tzcut \\ \hline
6.5 - 14.0   & 96.4 $\pm$ 8.9 $\pm$ 6.4 $\pm$ 11.2  & 97.0 $\pm$ 5.6 $\pm$ 5.1 $\pm$ 11.3
\end{tabular} 
\caption{The total \etac production cross-section in inclusive \bquark-decays}
\label{tab:TotalSecondaryTable}
\end{table}`

The results on \pt-differential \etac production cross-section in inclusive \bquark-decays from \tzfit and \tzcut are shown in Table ~\ref{tab:SecondaryTable}. The first uncertainty is statistical, the second is uncorrelated between bins systematic uncertainty, the third is correlated between bins systematic uncertainty, the last uncertainty is related to $\BR_{\JpsiToPpbar}$ and $\BR_{\EtacToPpbar}$ and \jpsi production measurement.

\newpage
\section{Cross-check of mass measurement using simultaneous fit to \pt bins}
\label{app:massInBins}
This appendix shows the fit of the invariant mass is performed simultaneously in 7 bins of charmonium transverse momentum.
The bin edges of $\pt(\ppbar)$ are [5.5, 6.5, 8.0, 10.0, 12.0, 14.0, 18.0, 30.0] expressed in \gevc. 
Distributions of invariant mass in each \pt-bin is shown on Fig.~\ref{fig:massTopo7Bins}.
In general, fit yields a good description of all $M_{\ppbar}$ distributions.
The fit gives the value of the \jpsi and \etac mass difference to be $\Delta M _{\jpsi , \, \etac} = \etacMassDiffInBins$, which is consistent with nominal result. 

\begin{figure}[hb]
\centering
\protect\protect\protect\includegraphics[width=1.4\linewidth, angle=90]{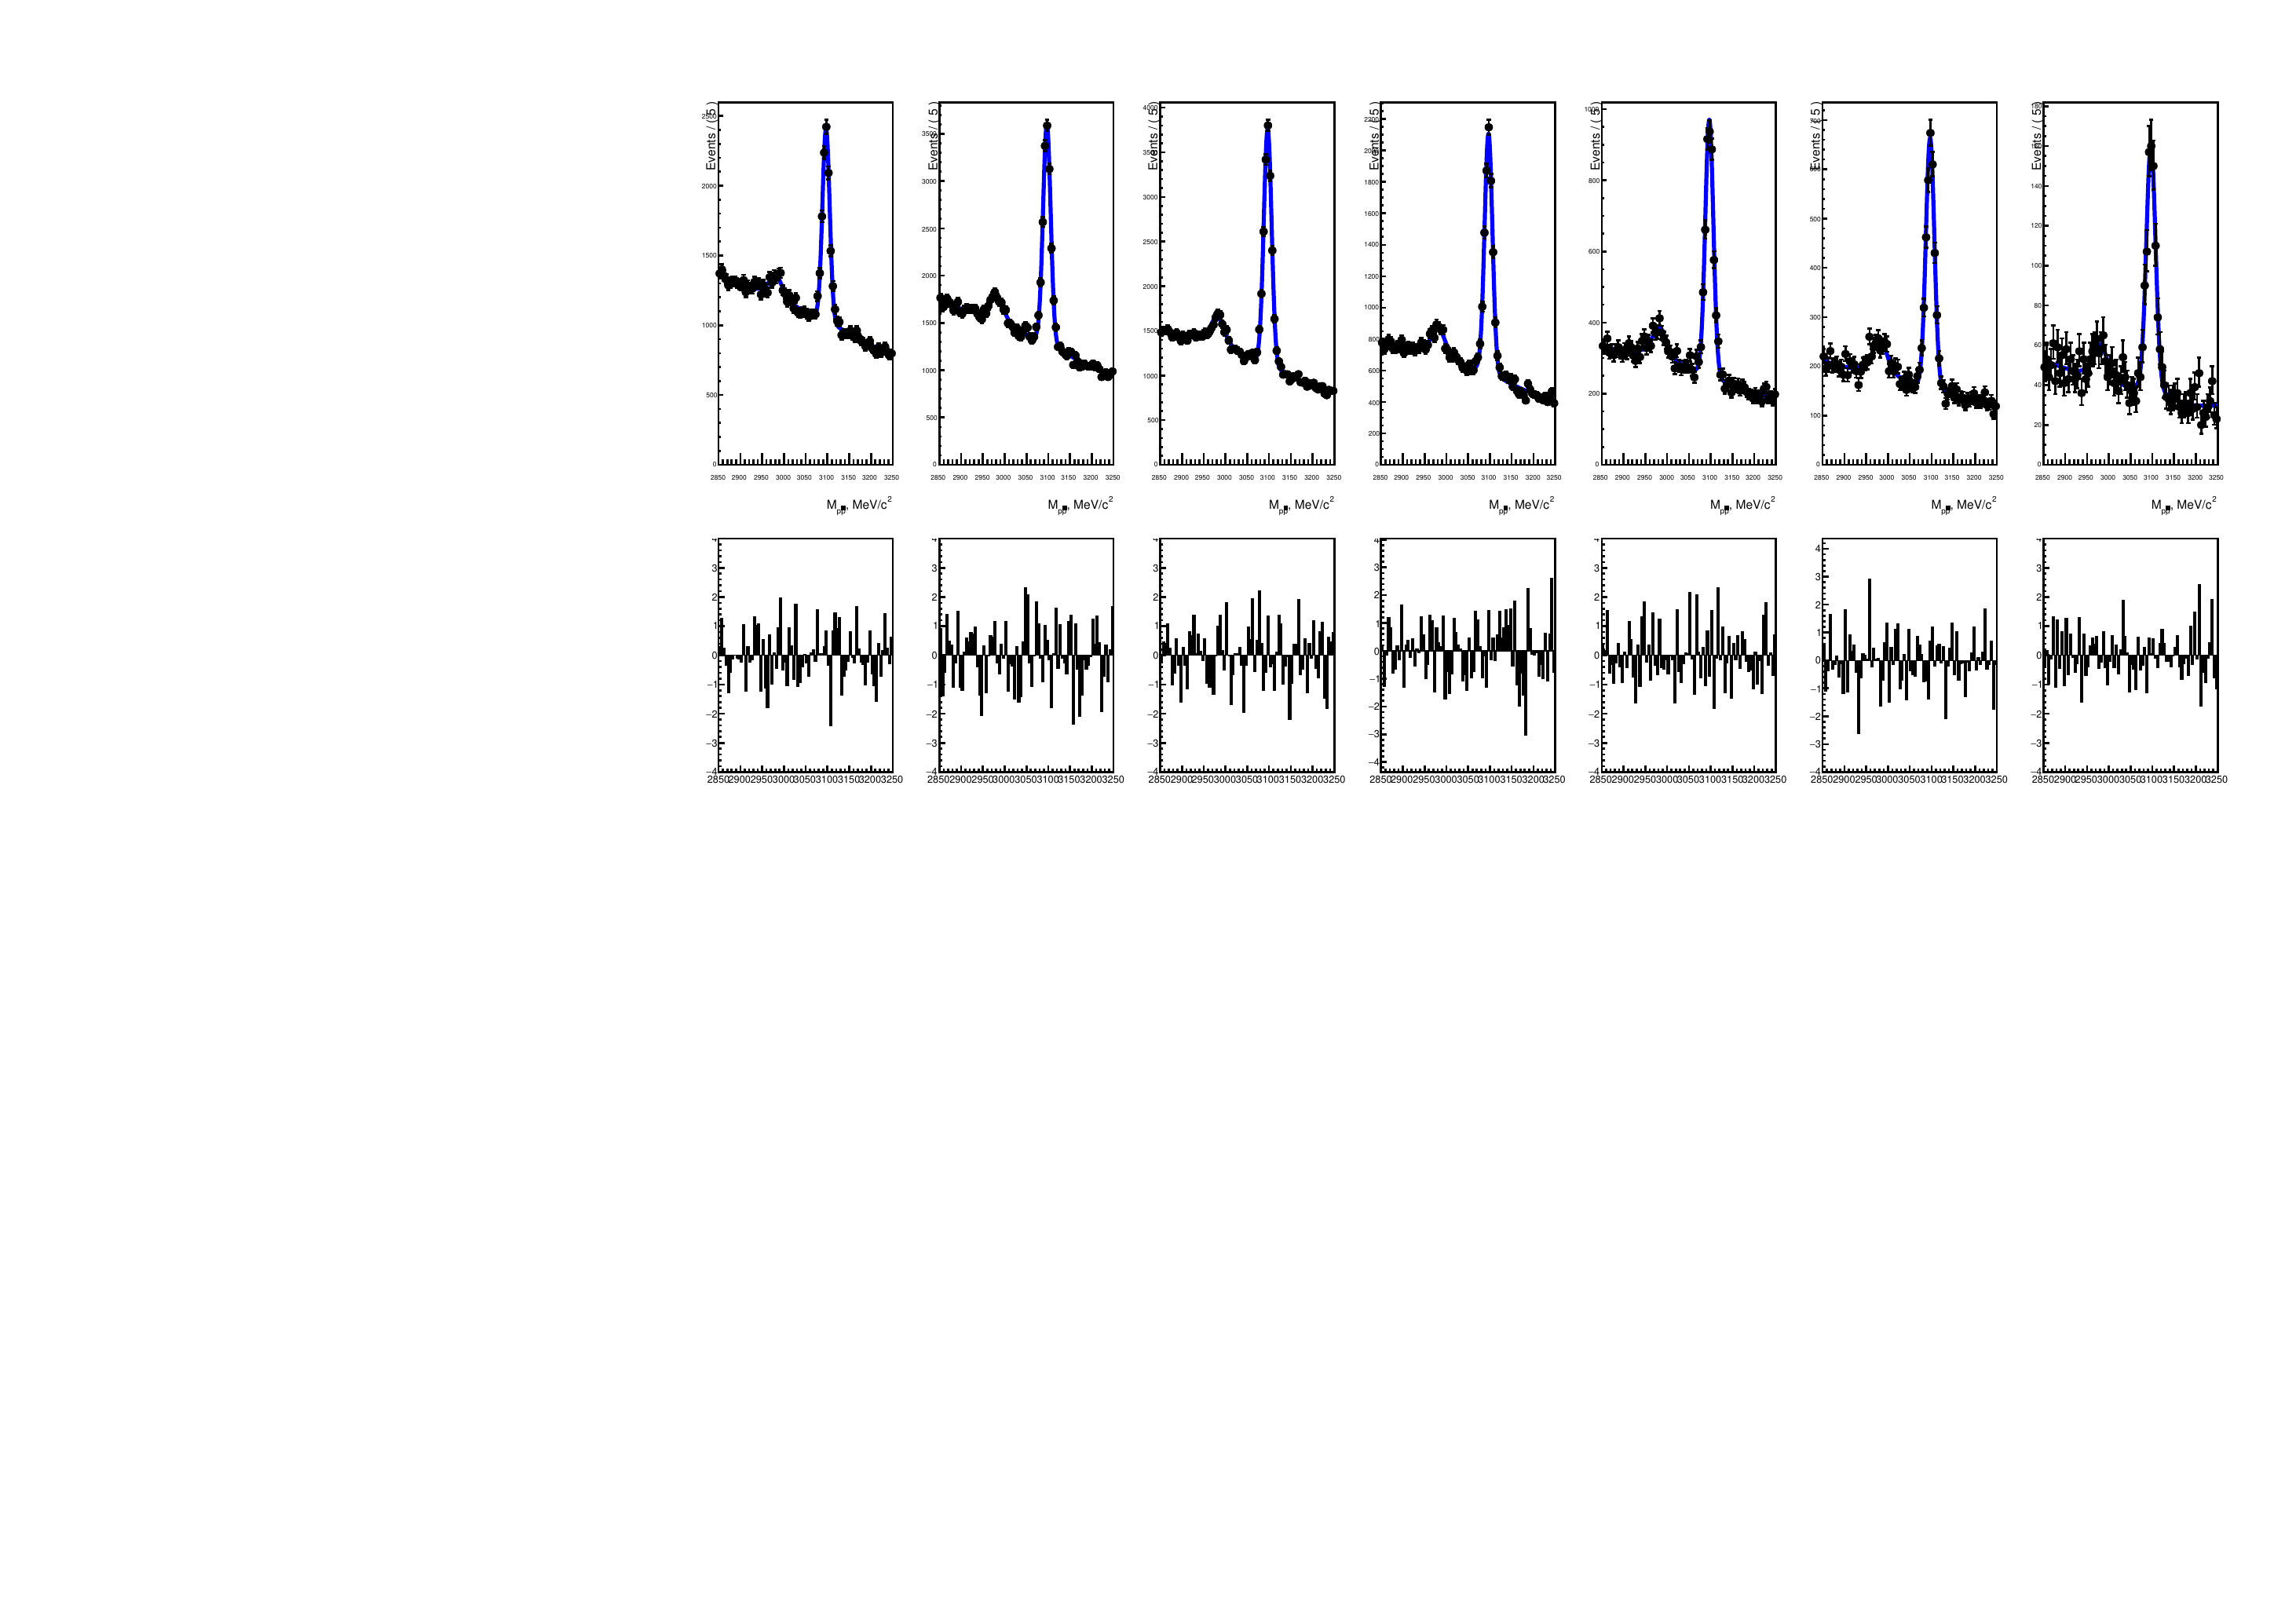}
\caption{Distributions of $M_{\ppbar}$ in \pt bins. The solid blues lines represent the simultaneous fit result. The corresponding pull distributions are shown below each plot.} 
\label{fig:massTopo7Bins}
\end{figure}
\clearpage

\newpage
\section{Cross-checks on PID efficiency ratio}
The PID efficiency ratio for \etac and \jpsi has been cross-checked by applying tighter PID cuts on MC. For this cross-check cuts $[PIDp>25\:\&\:(PIDp-PIDK)>15]$, $[PIDp>20\:\&\:(PIDp-PIDK)>20]$ and $[PIDp>25\:\&\:(PIDp-PIDK)>20]$ are used. Comparison of efficiency ratios for different cuts is shown in Table~\ref{tab:PIDCutsCheck}
\begin{table}[ht]
\centering
\small
\begin{tabular}{c|c}
cut            		       & $\epsilon_{\jpsi}/\epsilon_{\etac}$ \\ \hline 
nominal ($PIDp>20\:\&\:(PIDp-PIDK)>15$) & $1.00\pm0.02$ \\  \hline
$PIDp>25\:\&\:(PIDp-PIDK)>15$  		    & $0.99\pm0.02$ \\  
$PIDp>20\:\&\:(PIDp-PIDK)>20$  	        & $1.00\pm0.02$ \\
$PIDp>25\:\&\:(PIDp-PIDK)>20$  	        & $0.99\pm0.02$ \\
\end{tabular} 
\caption{The \jpsi and \etac efficiency ratio from MC for different PID cuts}
\label{tab:PIDCutsCheck}
\end{table} 

Another cross-check of PID efficiency is done by estimating PID efficiency ratio using PIDCalib package. The PID efficiency map is extracted using calibration samples of \decay{\Lambda}{\proton\pim} for Run II data and then applied to \etac and \jpsi MC samples. The extracted PID efficiency ratio compare to PID efficiency ratio from MC samples is shown in Eq.~\ref{eq:pidcalib}
\begin{equation}
\label{eq:pidcalib}
\begin{aligned}
\epsilon_{\jpsi}^{PID,MC}/\epsilon_{\etac}^{PID,MC}             &= 0.99\pm0.04\\
\epsilon_{\jpsi}^{PID,PIDCalib}/\epsilon_{\etac}^{PID,PIDCalib} &= 0.98\pm0.04
\end{aligned}
\end{equation}
No significant difference of \jpsi and \etac efficiency ratio from unity is observed for all cross-checks.
\clearpage

\newpage
\section{Fits to $t_z - t_z^{TRUE}$ in the MC samples in bins of \pt}
\label{app:TzResoPulls_PTbins}

This appendix shows fits to $t_z - t_z^{TRUE}$ in the MC samples in bins of \pt.
The fit for \pt-integrated samples ($6.5 \gevc < \pt < 14.0 \gevc$) is shown of Fig.~\ref{fig:fitMCTzReso_PT0}. Fits for $6.5 \gevc < \pt < 8.0 \gevc$, $8.0 \gevc < \pt < 10.0 \gevc$, $10.0 \gevc < \pt < 12.0 \gevc$ and $12.0 \gevc < \pt < 14.0 \gevc$ are shown of Figs.~\ref{fig:fitMCTzReso_PT1},~\ref{fig:fitMCTzReso_PT2},~\ref{fig:fitMCTzReso_PT3} and ~\ref{fig:fitMCTzReso_PT4}, respectively.
\begin{figure}[ht]
\centering
\protect\protect\protect\includegraphics[width=1.\linewidth]{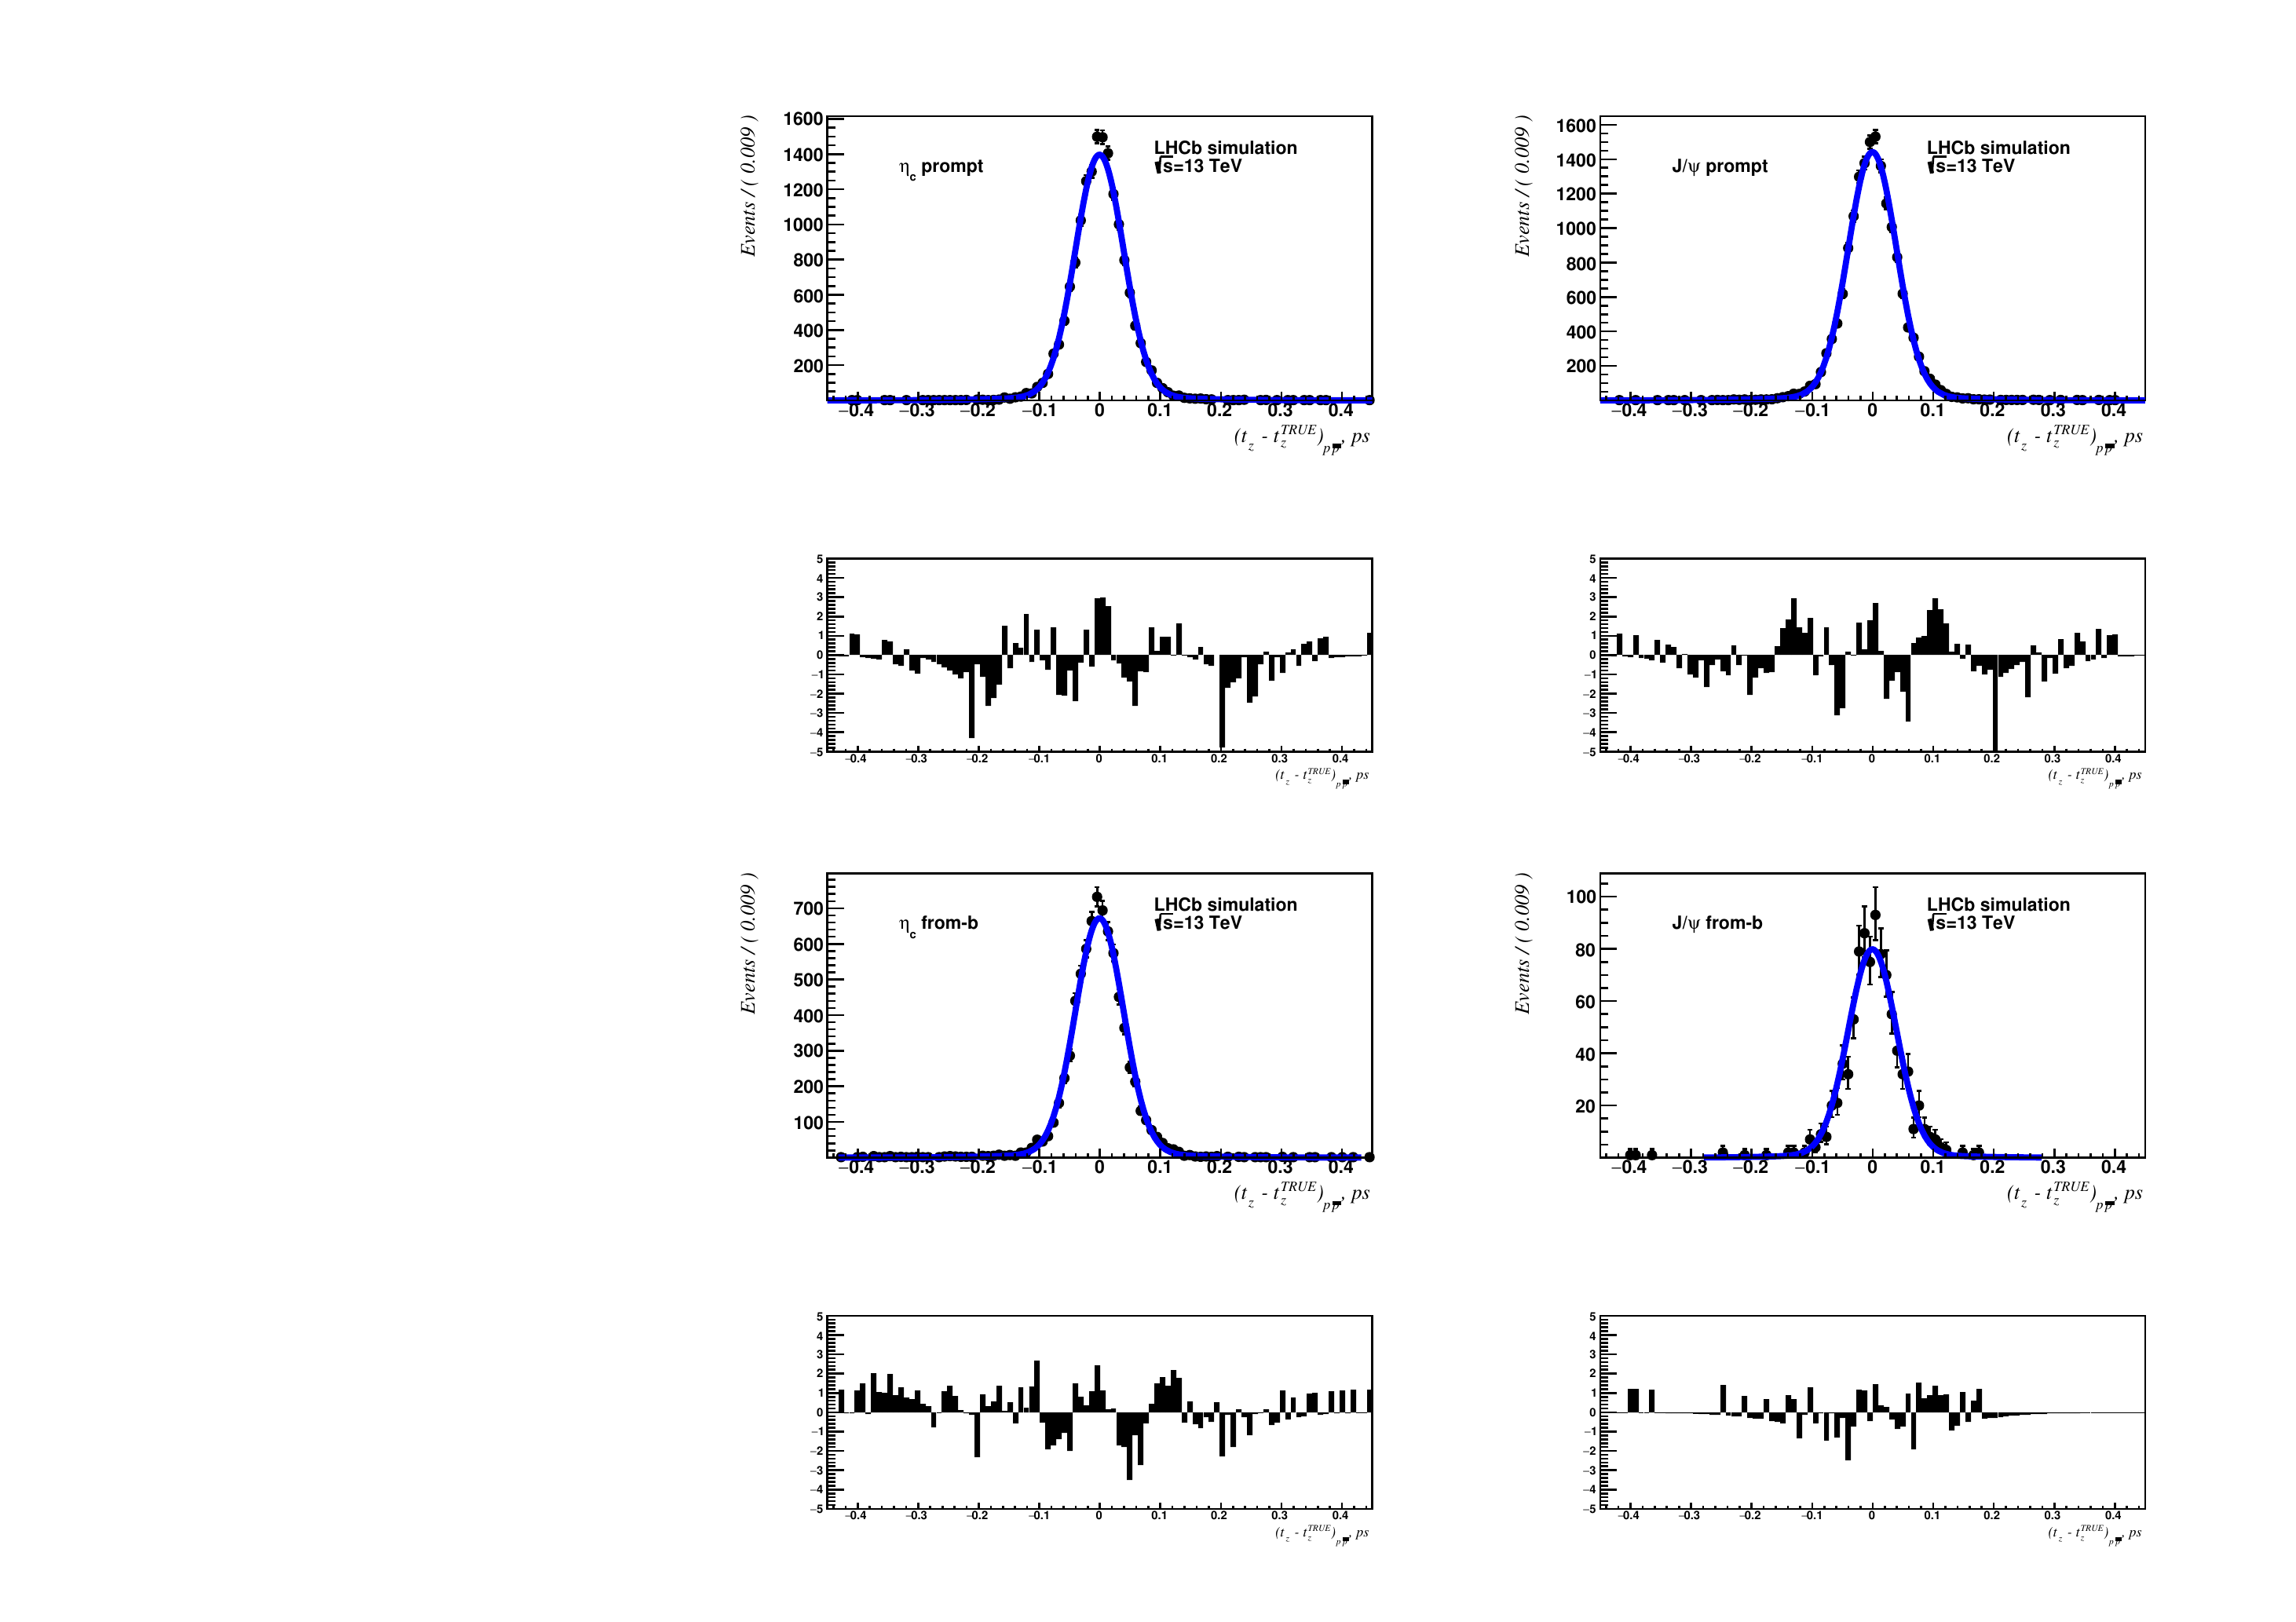}
\caption{Distribution of the $t_z - t_z^{TRUE}$ in the \pt-integrated ($6.5 \gevc < \pt < 14.0 \gevc$) MC samples: prompt \etac (top left), prompt \jpsi (top right), \etac from \bquark-decays (bottom left) and \jpsi from \bquark-decays (bottom right). The solid blue lines represent the result of the simultaneous fit by a double Gaussian function to all four MC samples. The corresponding pull distributions are shown below.}
\label{fig:fitMCTzReso_PT0}
\end{figure}
\clearpage

\begin{figure}[ht]
\centering
\protect\protect\protect\includegraphics[width=1.\linewidth]{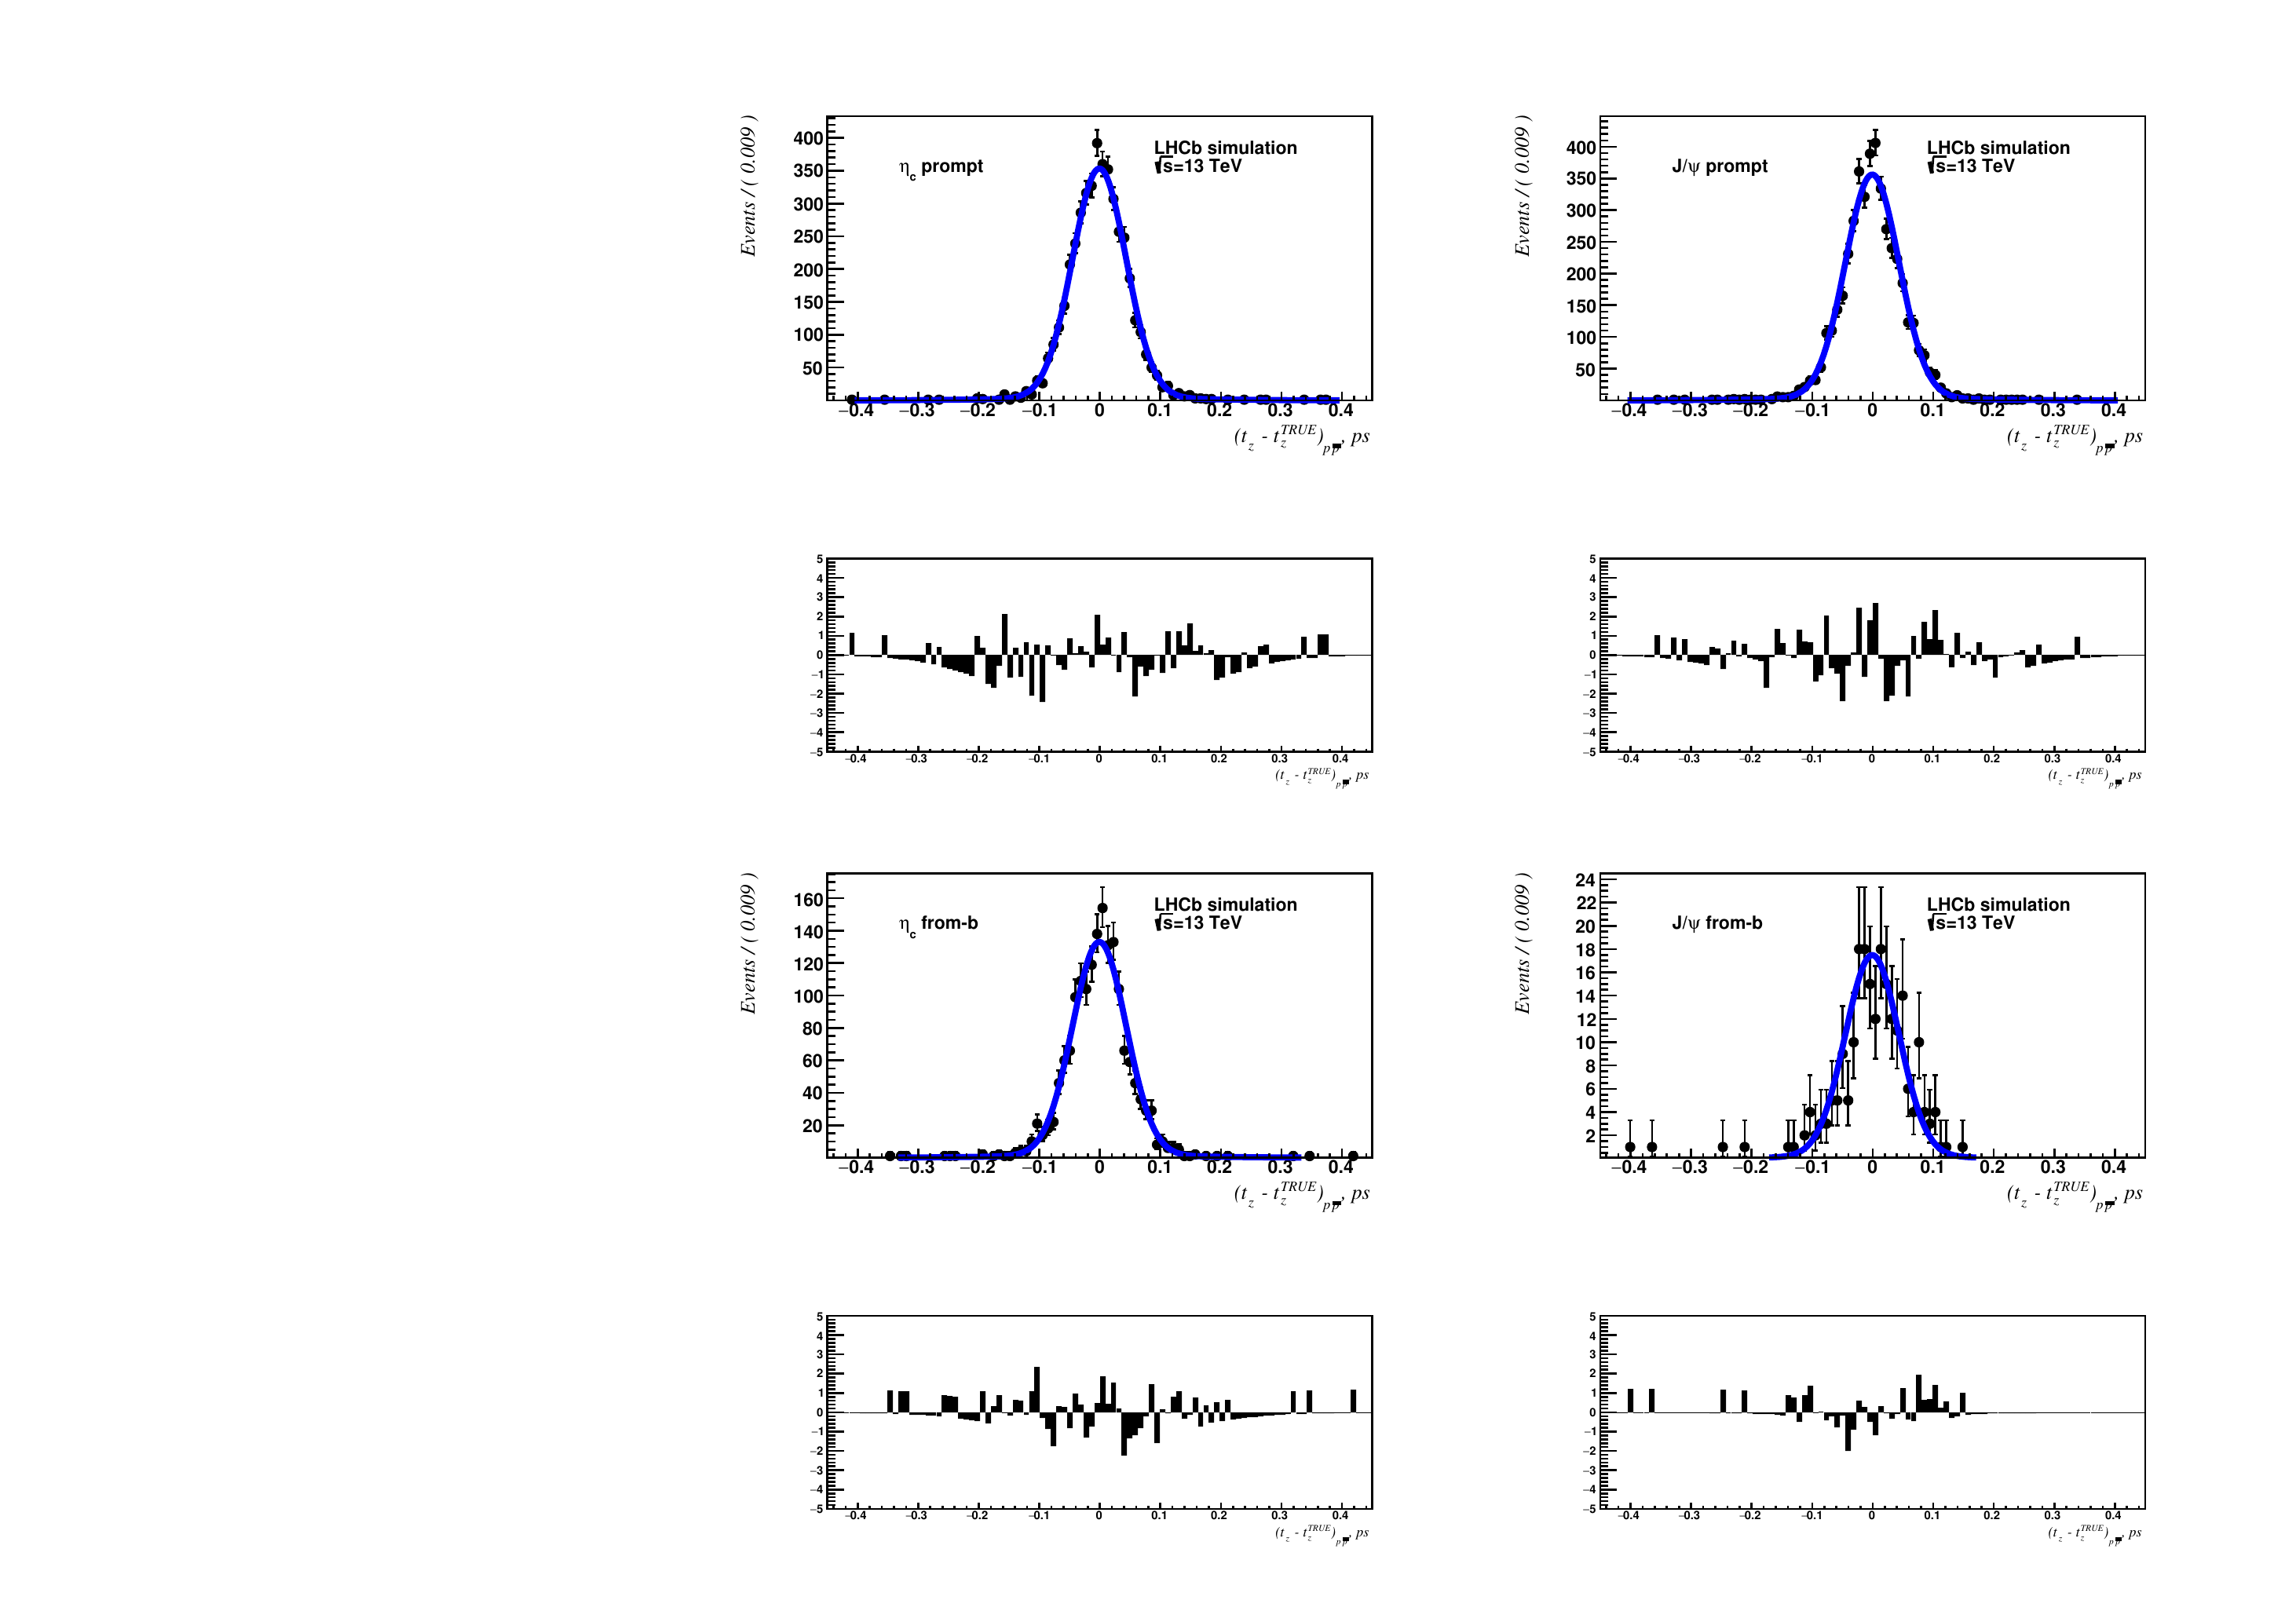}
\caption{Distribution of the $t_z - t_z^{TRUE}$ MC samples: prompt \etac (top left), prompt \jpsi (top right), \etac from \bquark-decays (bottom left) and \jpsi from \bquark-decays (bottom right) for $6.5 \gevc < \pt < 8.0 \gevc$. The solid blue lines represent the result of the simultaneous fit by a double Gaussian function to all four MC samples. The corresponding pull distributions are shown below.}
\label{fig:fitMCTzReso_PT1}
\end{figure}

\begin{figure}[ht]
\centering
\protect\protect\protect\includegraphics[width=1.\linewidth]{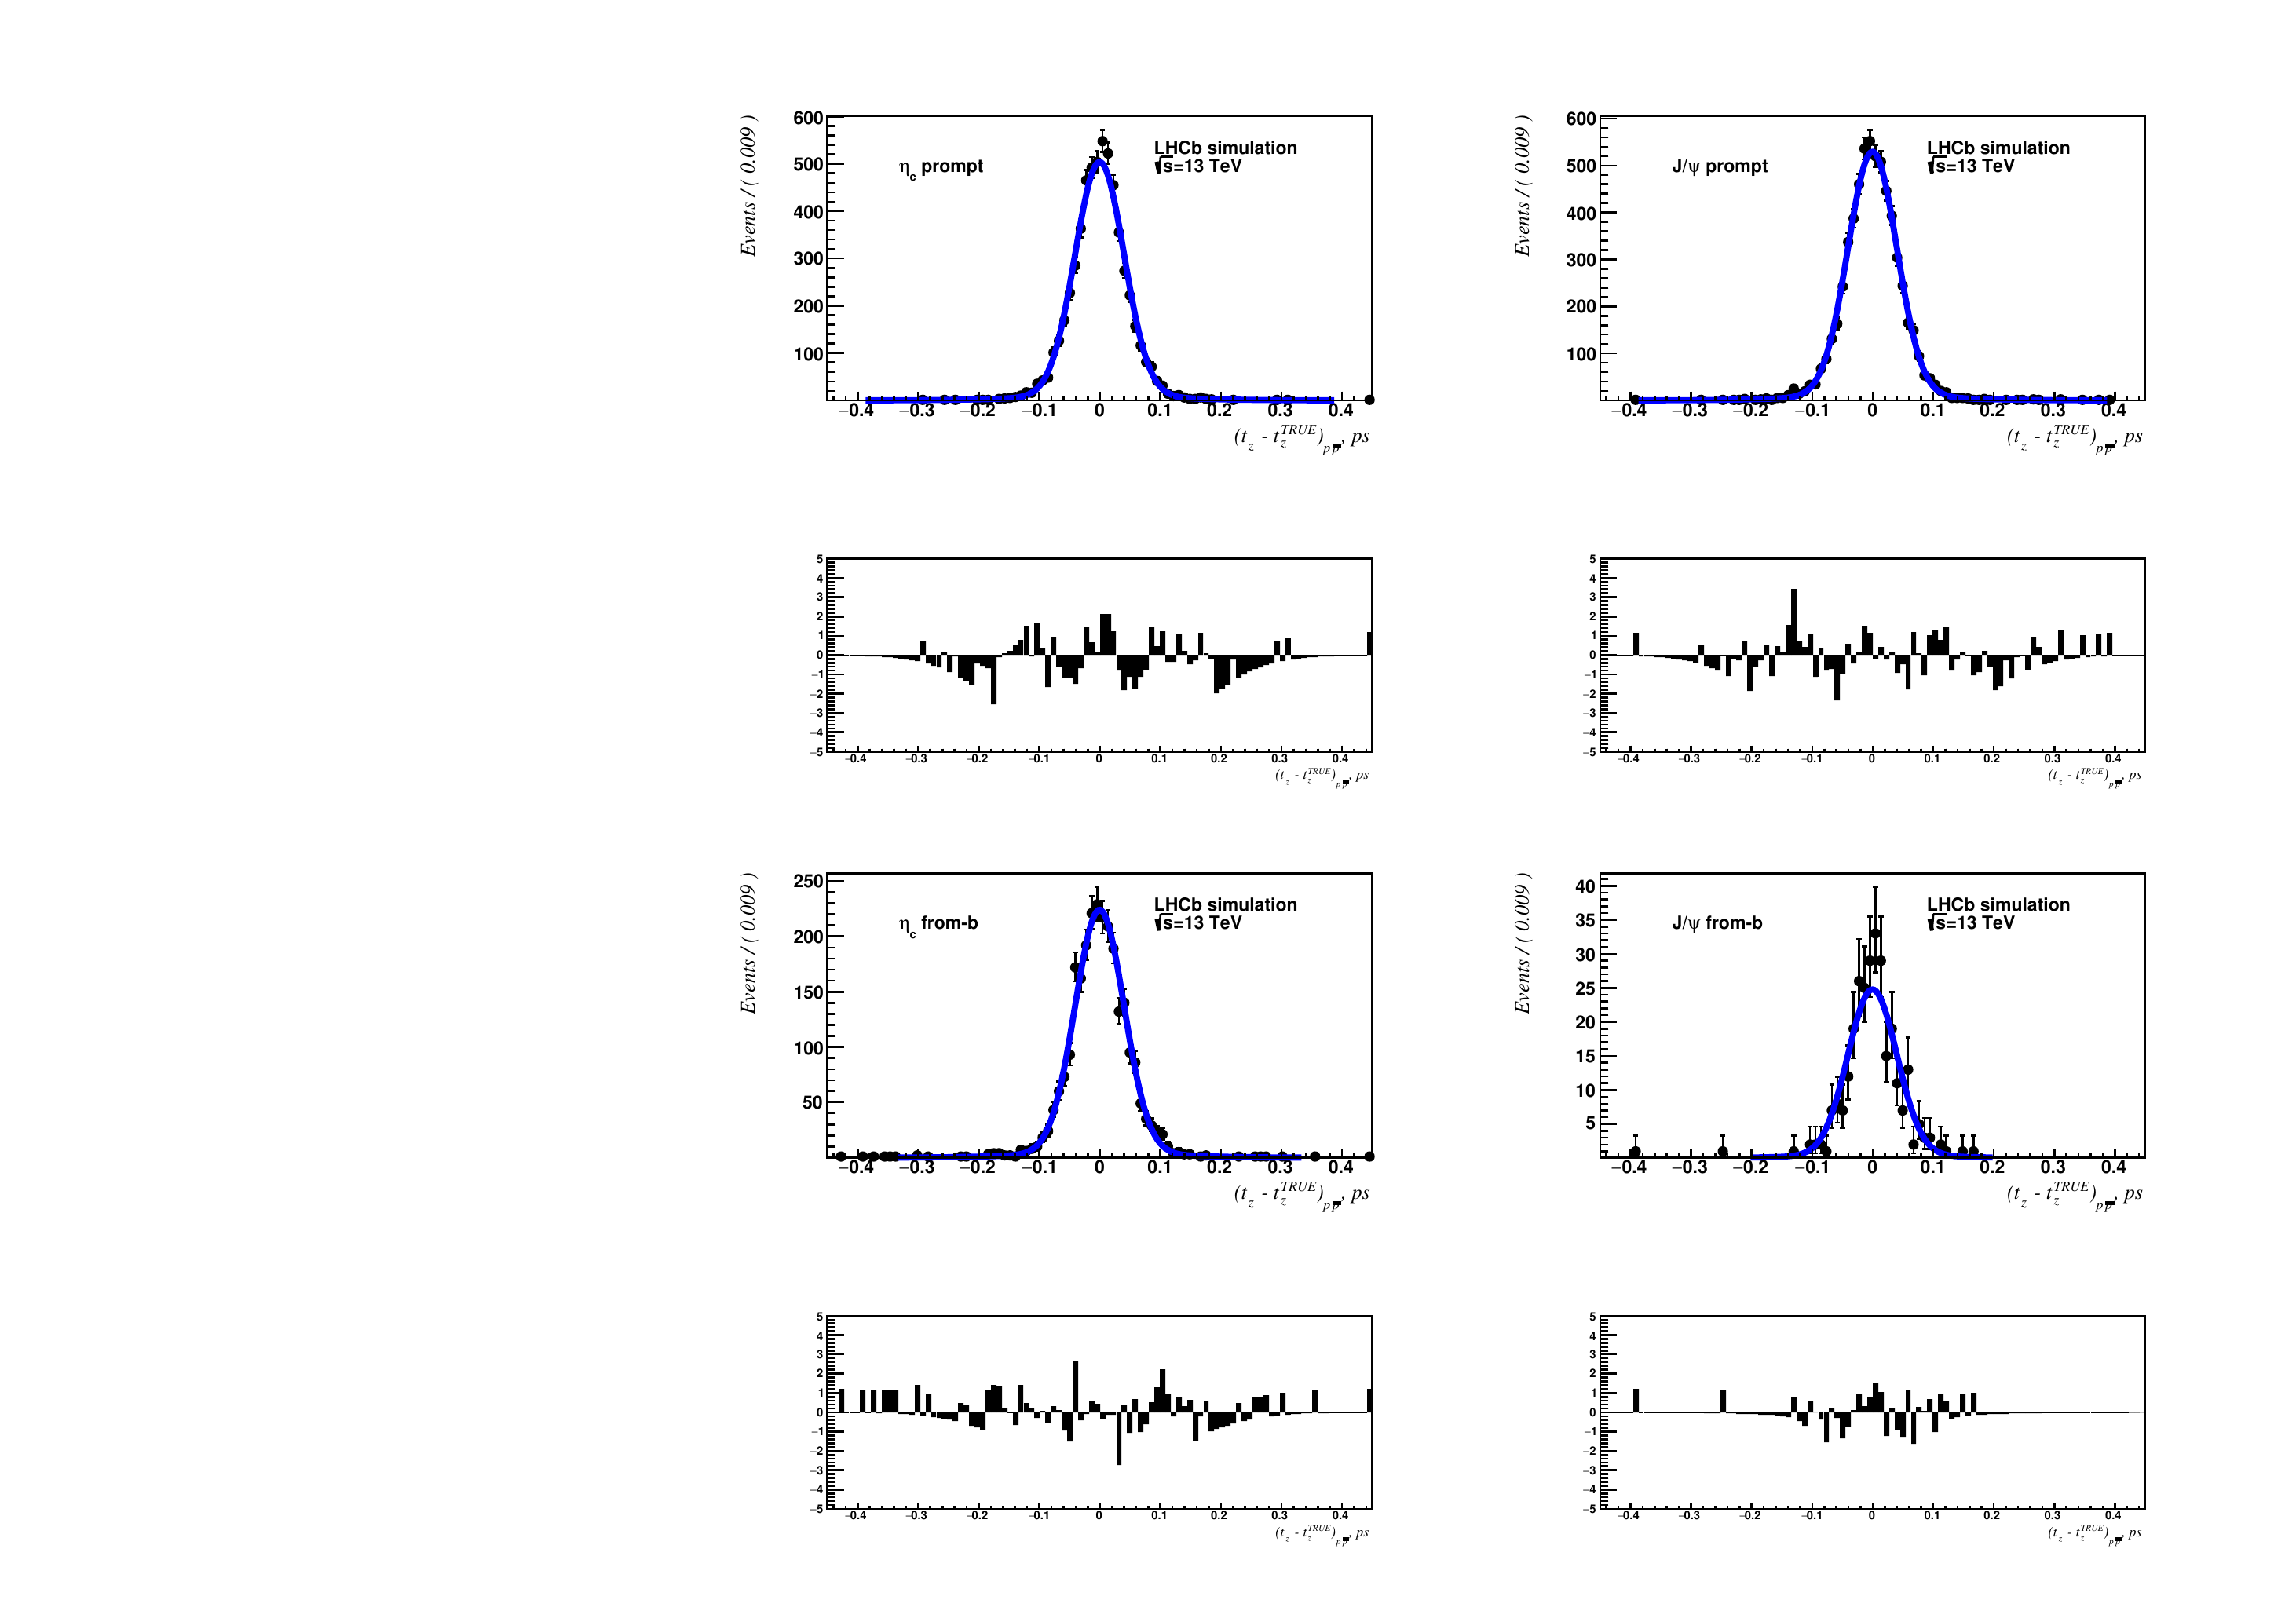}
\caption{Distribution of the $t_z - t_z^{TRUE}$ MC samples: prompt \etac (top left), prompt \jpsi (top right), \etac from \bquark-decays (bottom left) and \jpsi from \bquark-decays (bottom right) for $8.0 \gevc < \pt < 10.0 \gevc$. The solid blue lines represent the result of the simultaneous fit by a double Gaussian function to all four MC samples. The corresponding pull distributions are shown below.}
\label{fig:fitMCTzReso_PT2}
\end{figure}

\begin{figure}[ht]
\centering
\protect\protect\protect\includegraphics[width=1.\linewidth]{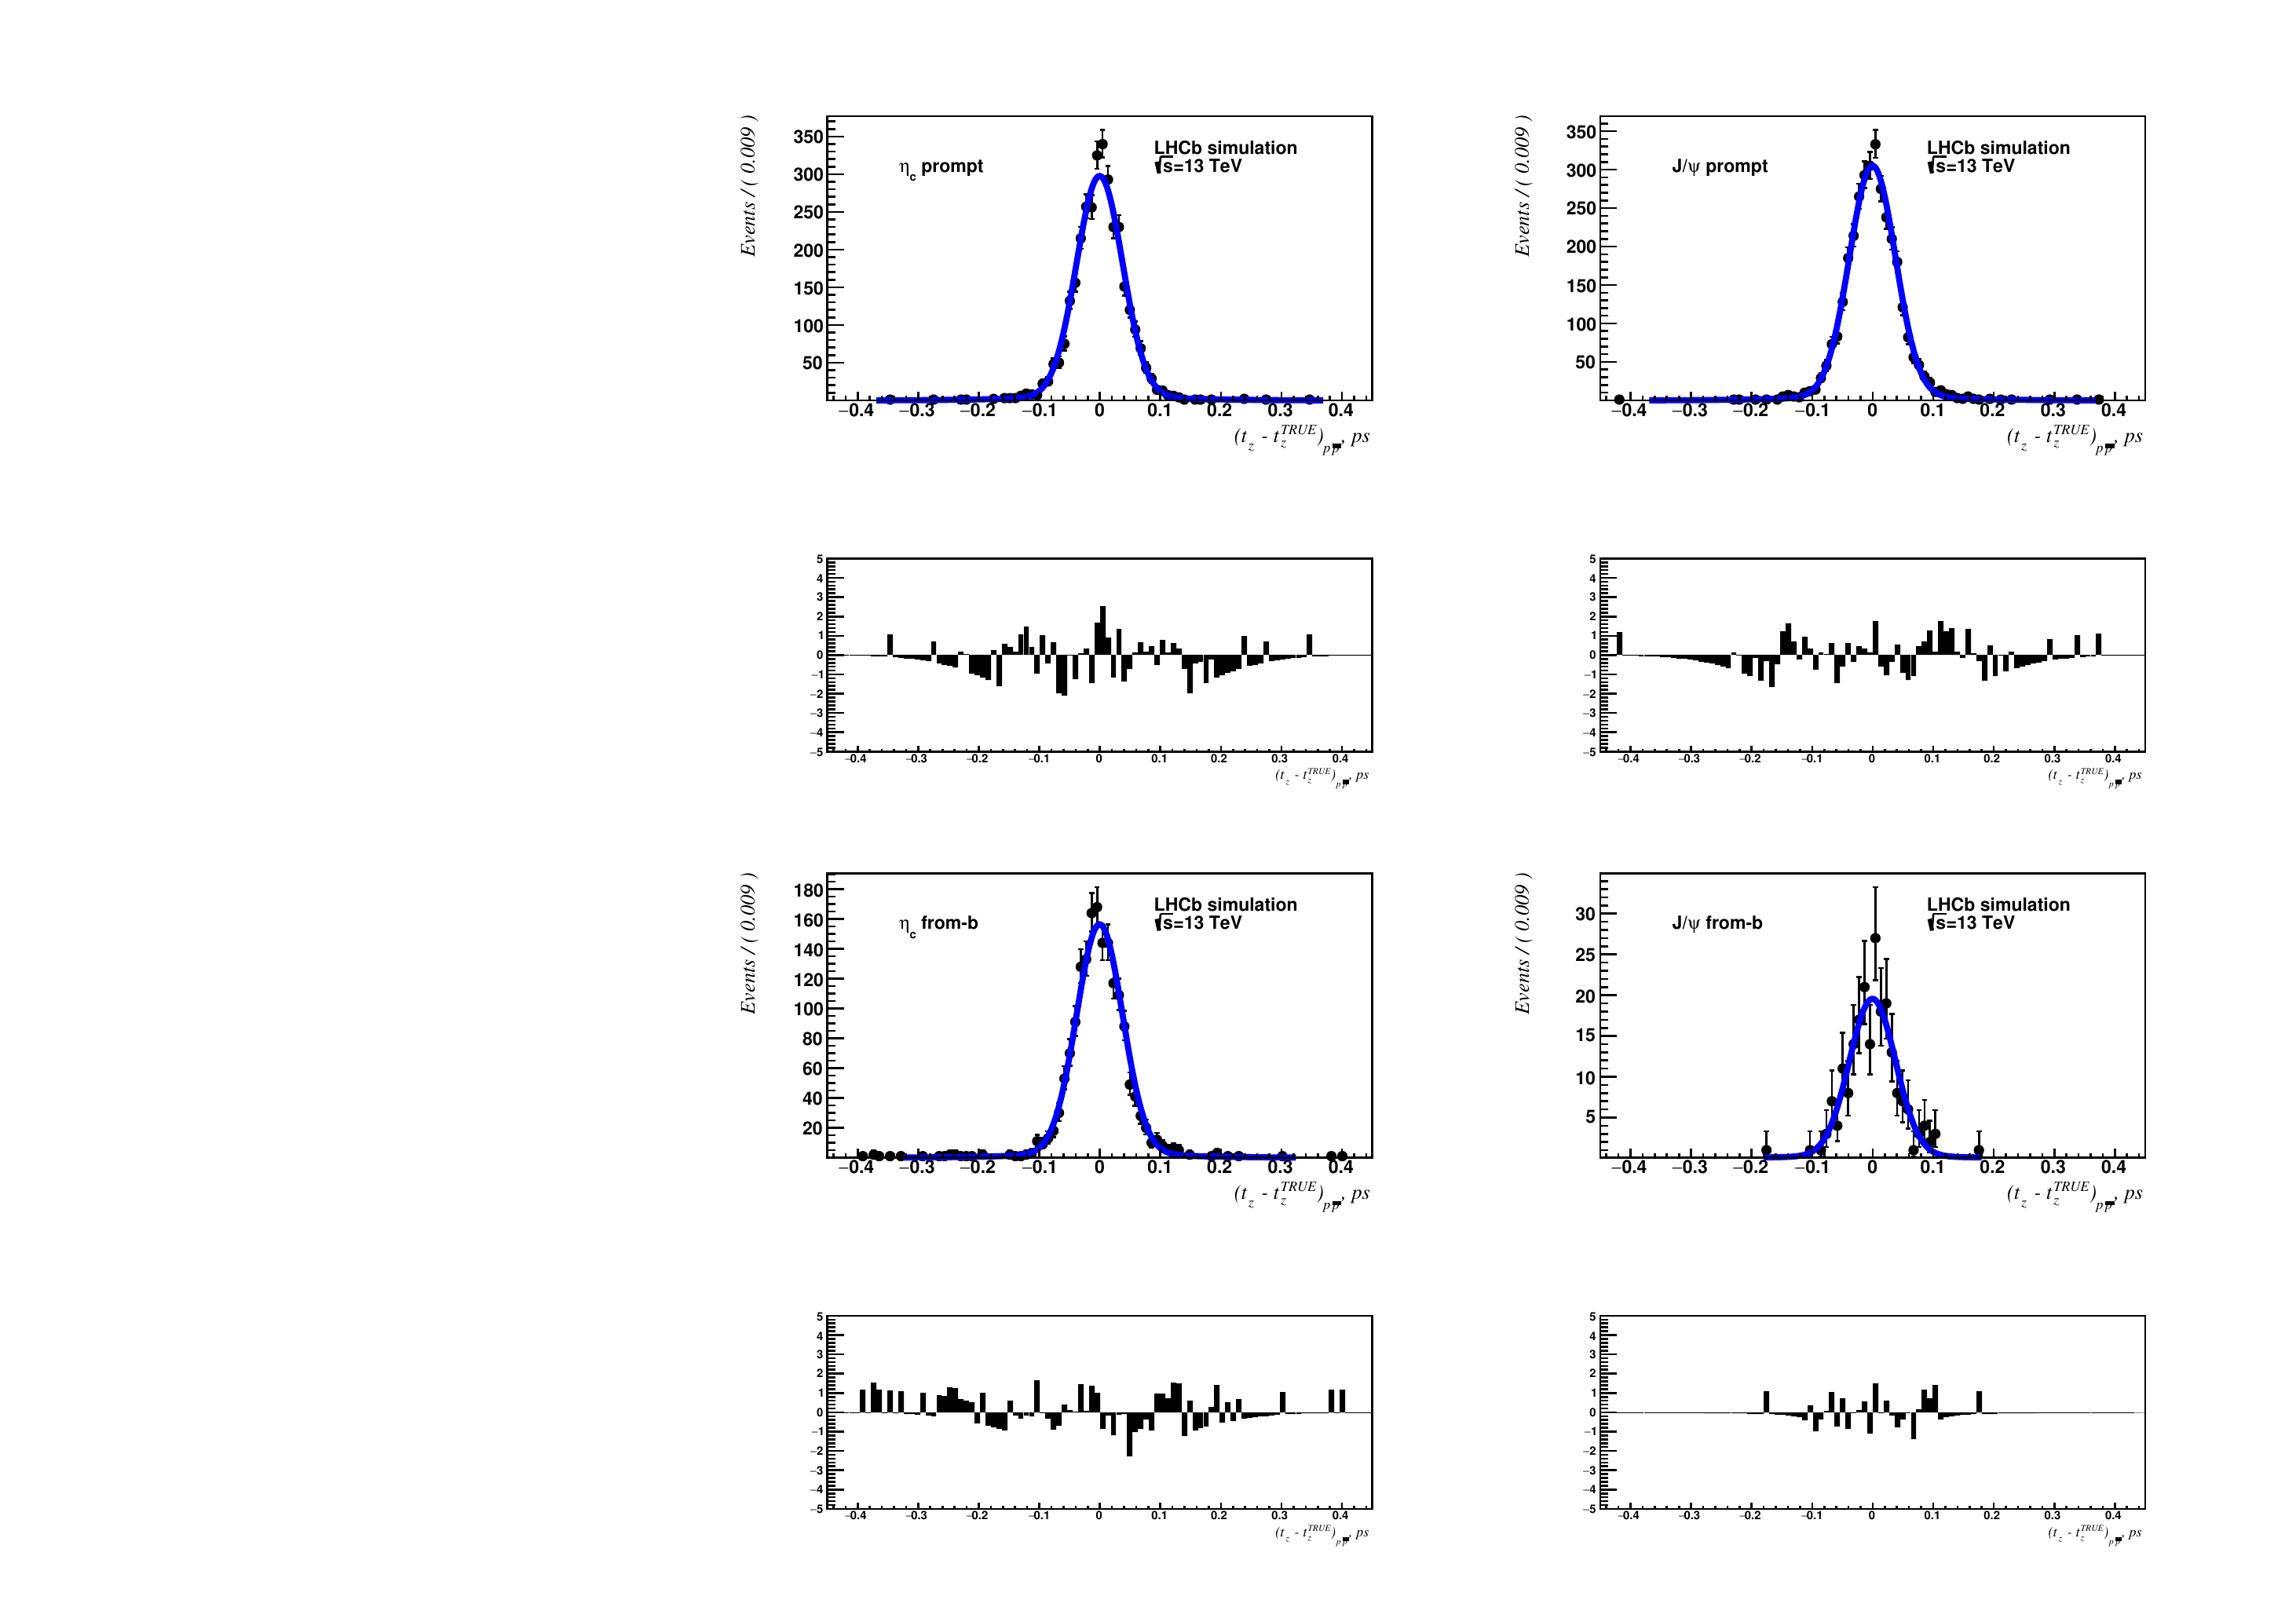}
\caption{Distribution of the $t_z - t_z^{TRUE}$ MC samples: prompt \etac (top left), prompt \jpsi (top right), \etac from \bquark-decays (bottom left) and \jpsi from \bquark-decays (bottom right) for $10.0 \gevc < \pt < 12.0 \gevc$. The solid blue lines represent the result of the simultaneous fit by a double Gaussian function to all four MC samples. The corresponding pull distributions are shown below.}
\label{fig:fitMCTzReso_PT3}
\end{figure}

\begin{figure}[ht]
\centering
\protect\protect\protect\includegraphics[width=1.\linewidth]{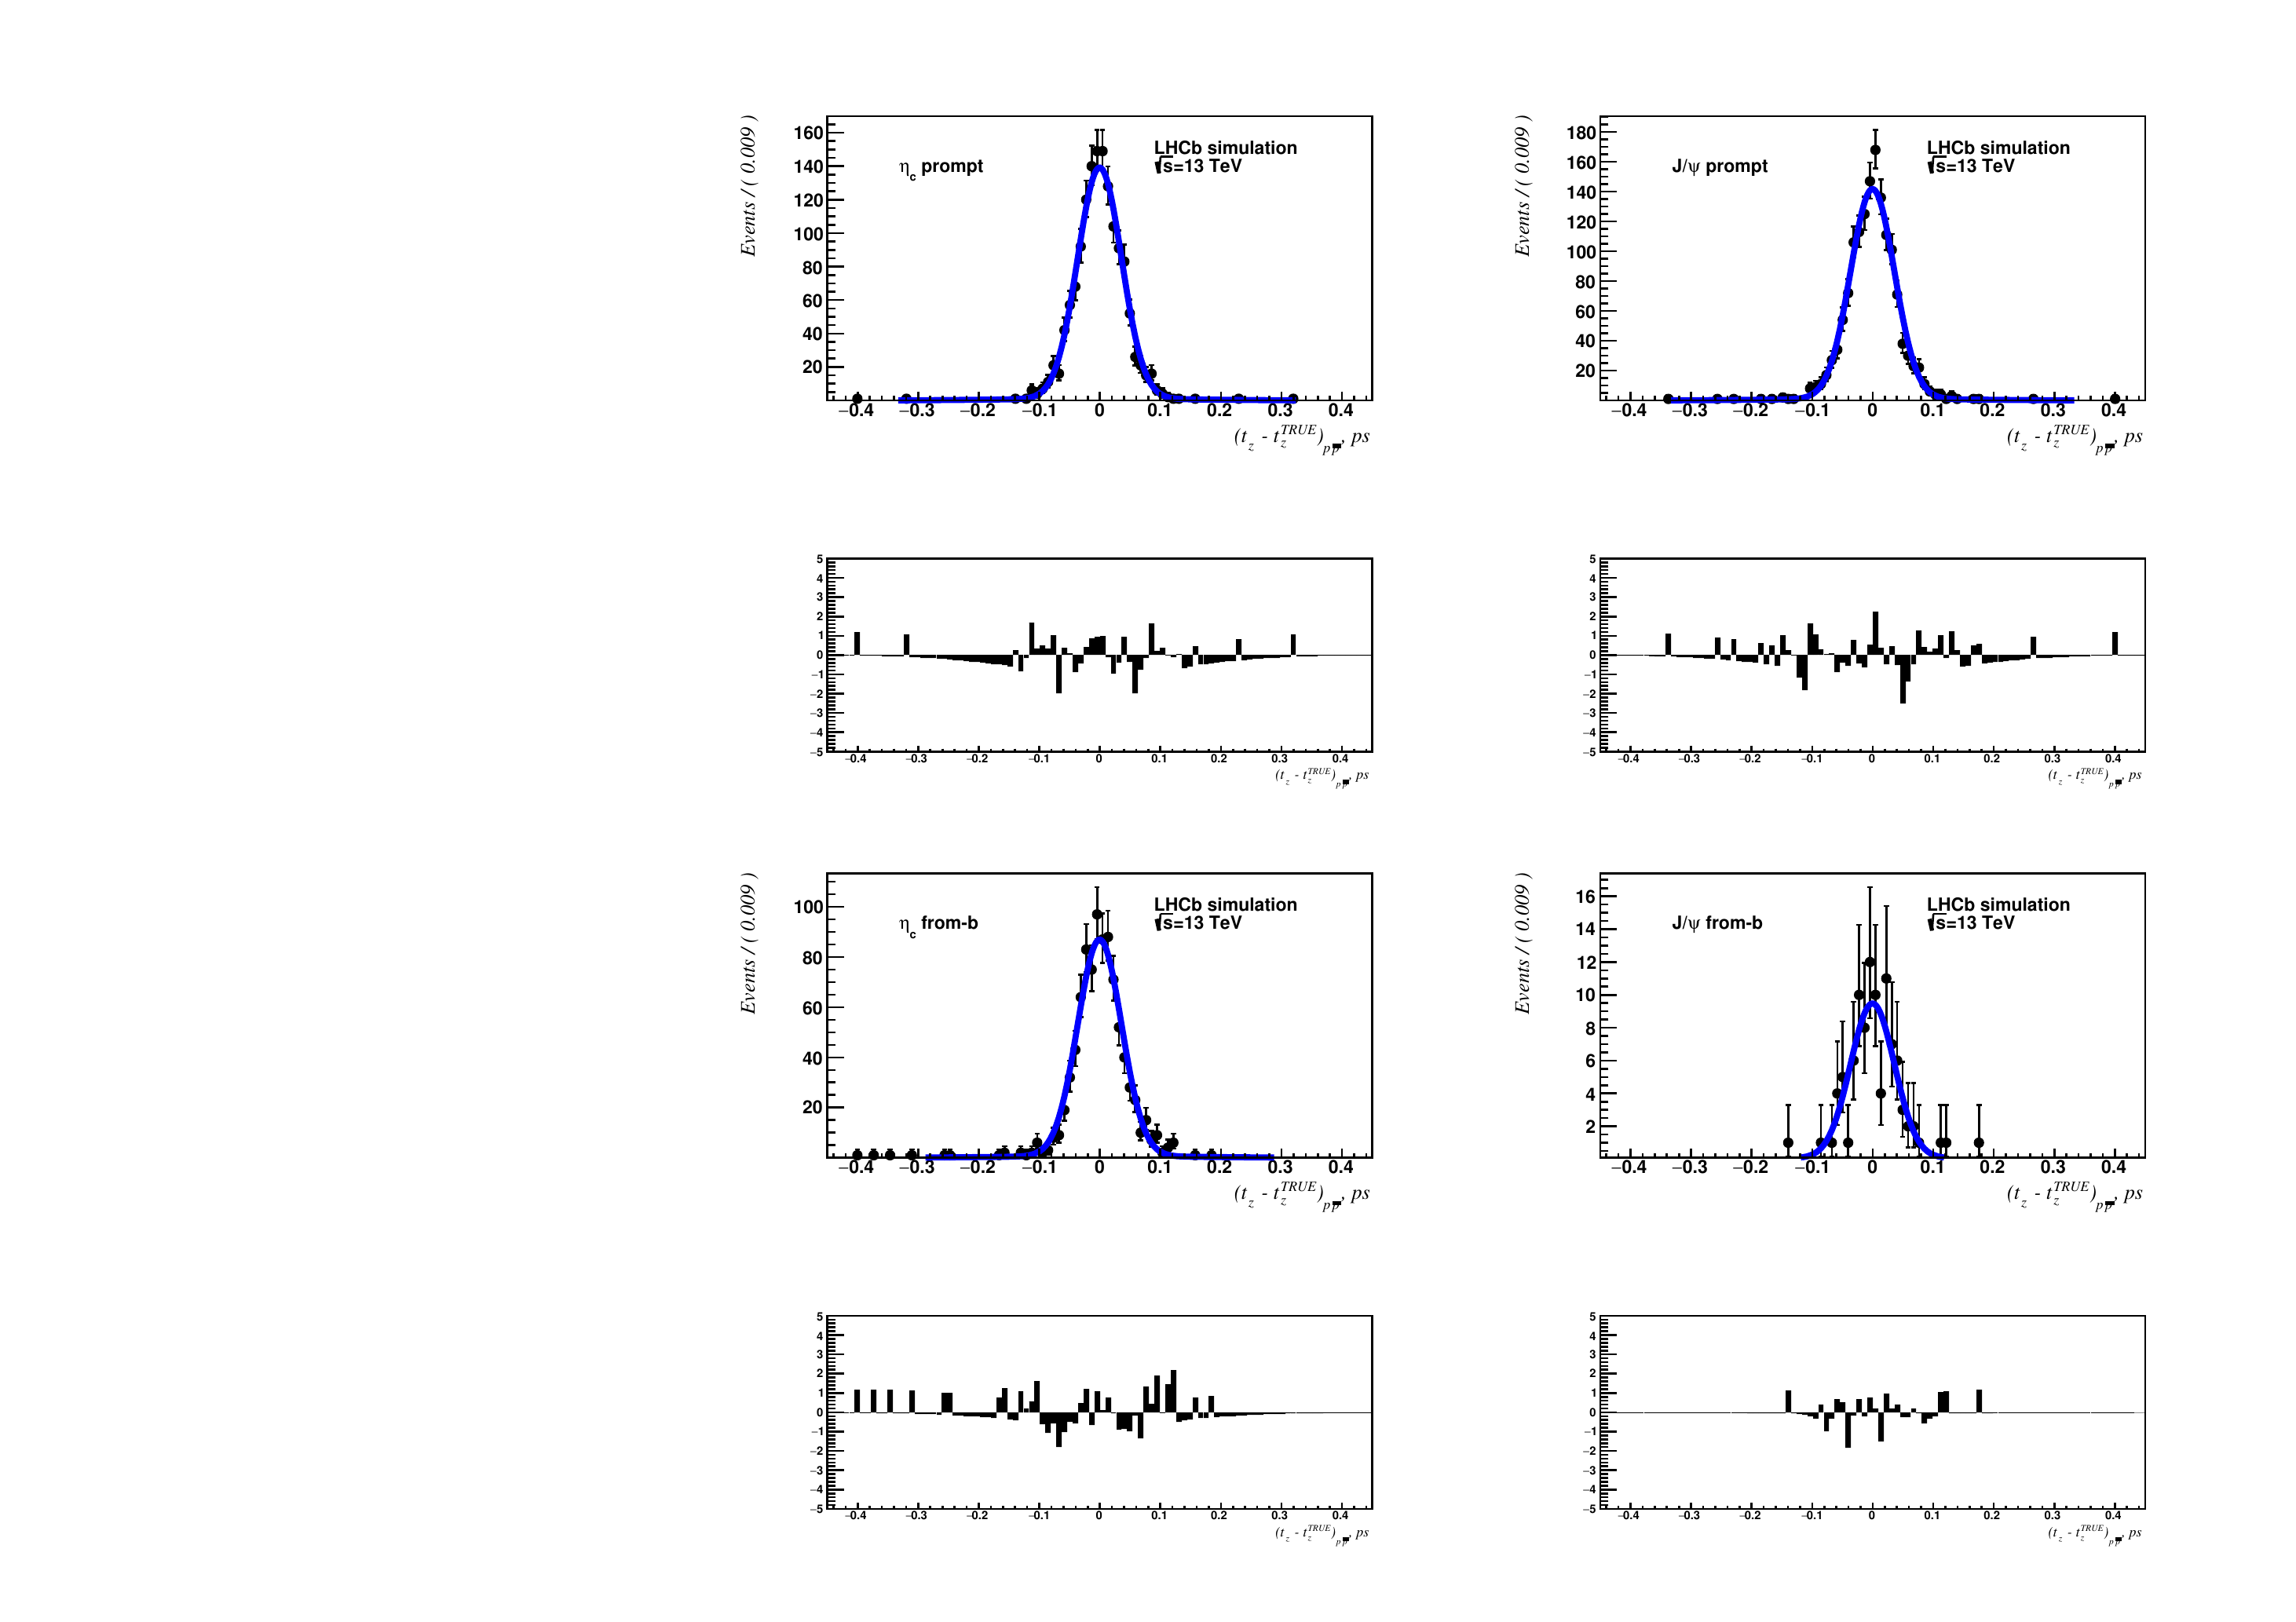}
\caption{Distribution of the $t_z - t_z^{TRUE}$ MC samples: prompt \etac (top left), prompt \jpsi (top right), \etac from \bquark-decays (bottom left) and \jpsi from \bquark-decays (bottom right) for $12.0 \gevc < \pt < 14.0 \gevc$. The solid blue lines represent the result of the simultaneous fit by a double Gaussian function to all four MC samples. The corresponding pull distributions are shown below.}
\label{fig:fitMCTzReso_PT4}
\end{figure}
\clearpage

\newpage
\section{Parameters from fits to $M_{\proton\antiproton} - M^{TRUE}_{\proton\antiproton}$ in the MC samples in bins of \pt}
\label{app:MCReso_PTbins}
Table~\ref{tab:parsResoMass} shows parameter values from fits to $M_{\proton\antiproton} - M^{TRUE}_{\proton\antiproton}$ in the MC samples in bins of \pt.
\begin{table}[ht] 
\begin{center}
{\footnotesize{
\centering
\begin{tabular}{c|c|c|c|c|c|c} 
 \pt, \gevc  & $\sigma_\etac$ & $\sigma_\etac/\sigma_\jpsi$ & $\sigma_n/\sigma_w$  & $f_n$  & mean \etac & mean \jpsi \\ \hline\hline
 6.5 - 14.0  & $7.50\pm0.05$ & $0.945\pm0.008$ & $0.211\pm0.005$ & $0.952\pm0.002$ & $0.52\pm0.06$ & $0.58\pm0.06$ \\ \hline\hline
 6.5 - 8.0   & $7.42\pm0.10$ & $0.948\pm0.016$ & $0.227\pm0.010$ & $0.949\pm0.004$ & $0.66\pm0.16$ & $0.47\pm0.11$ \\ \hline
 8.0 - 10.0  & $7.30\pm0.08$ & $0.932\pm0.013$ & $0.195\pm0.009$ & $0.958\pm0.003$ & $0.45\pm0.10$ & $0.54\pm0.09$ \\ \hline
 10.0 - 12.0 & $7.42\pm0.10$ & $0.944\pm0.018$ & $0.217\pm0.011$ & $0.949\pm0.004$ & $0.51\pm0.14$ & $0.58\pm0.12$ \\ \hline
 12.0 - 14.0 & $7.54\pm0.17$ & $0.960\pm0.027$ & $0.213\pm0.014$ & $0.935\pm0.007$ & $0.64\pm0.21$ & $0.86\pm0.18$ \\ \hline
\end{tabular}
}}
\caption{Parameters from fits to $M_{\proton\antiproton} - M^{TRUE}_{\proton\antiproton}$ in the MC samples in bins of \pt.}
\label{tab:parsResoMass}
\end{center}
\end{table}
\clearpage

\newpage
\section{Zooms of the tz-fit plots}
\label{app:zooms}
Zooms of simultaneous fit curve to $t_z$ in each bin of \pt are shown on Figs.~\ref{fig:tzFitZoomPT1},~\ref{fig:tzFitZoomPT2},~\ref{fig:tzFitZoomPT3},~\ref{fig:tzFitZoomPT4}.

\begin{figure}[ht]
\centering
\protect\protect\protect\includegraphics[width=0.9\textwidth]{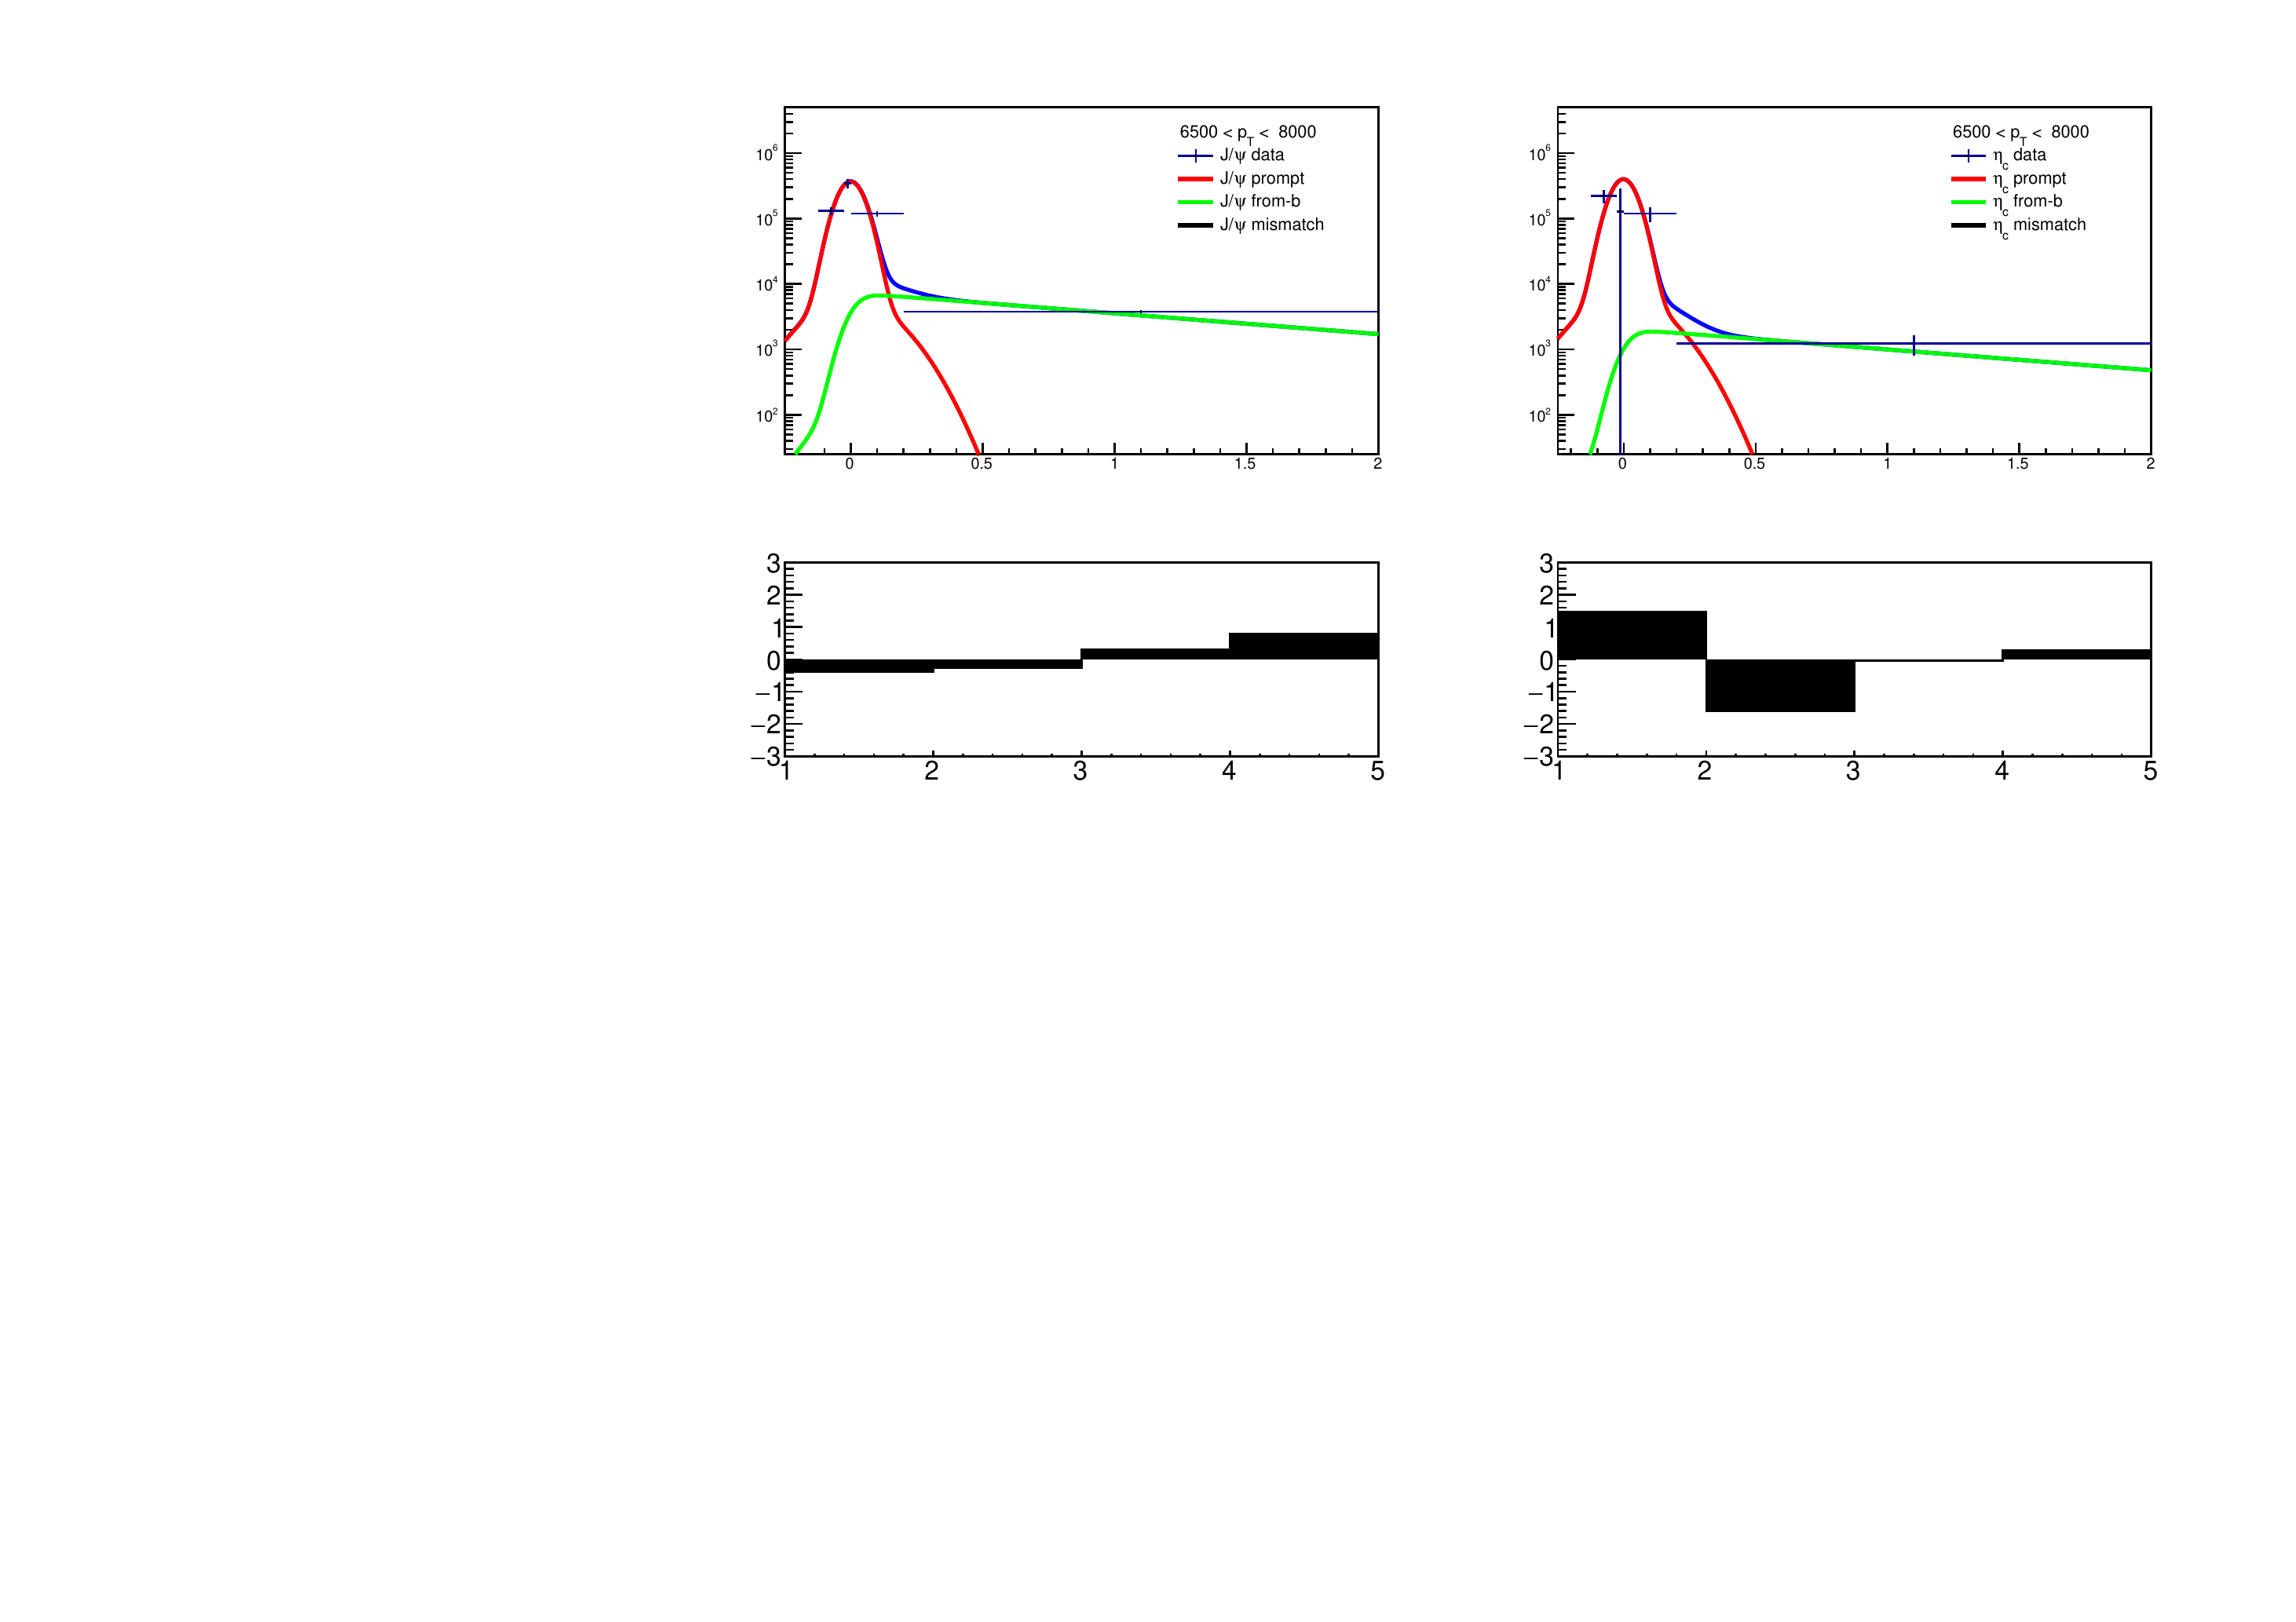}
\put(-46,-7){\scriptsize{$N(t_z)$}}
\put(-274,-7){\scriptsize{$N(t_z)$}}
\put(-192,185){\scriptsize{\lhcb preliminary}}
\put(-420,185){\scriptsize{\lhcb preliminary}}
\caption{The zoom of the $t_z$ distribution for \jpsi (left) and \etac (right) for $6.5 \gevc<\pt<8.0 \gevc$ and the result of simultaneous integral \chisq fit in all \pt bins. Red lines show prompt components, green lines show \etac and \jpsi from inclusive \bquark-decays, black lines show contributions from the events with wrongly associated PV. The corresponding pull distributions are shown below, where the $N(t_z)$ on the pull distributions denotes the $t_z$ bin number.} 
\label{fig:tzFitZoomPT1}
\end{figure}

\begin{figure}[ht]
\centering
\protect\protect\protect\includegraphics[width=0.9\textwidth]{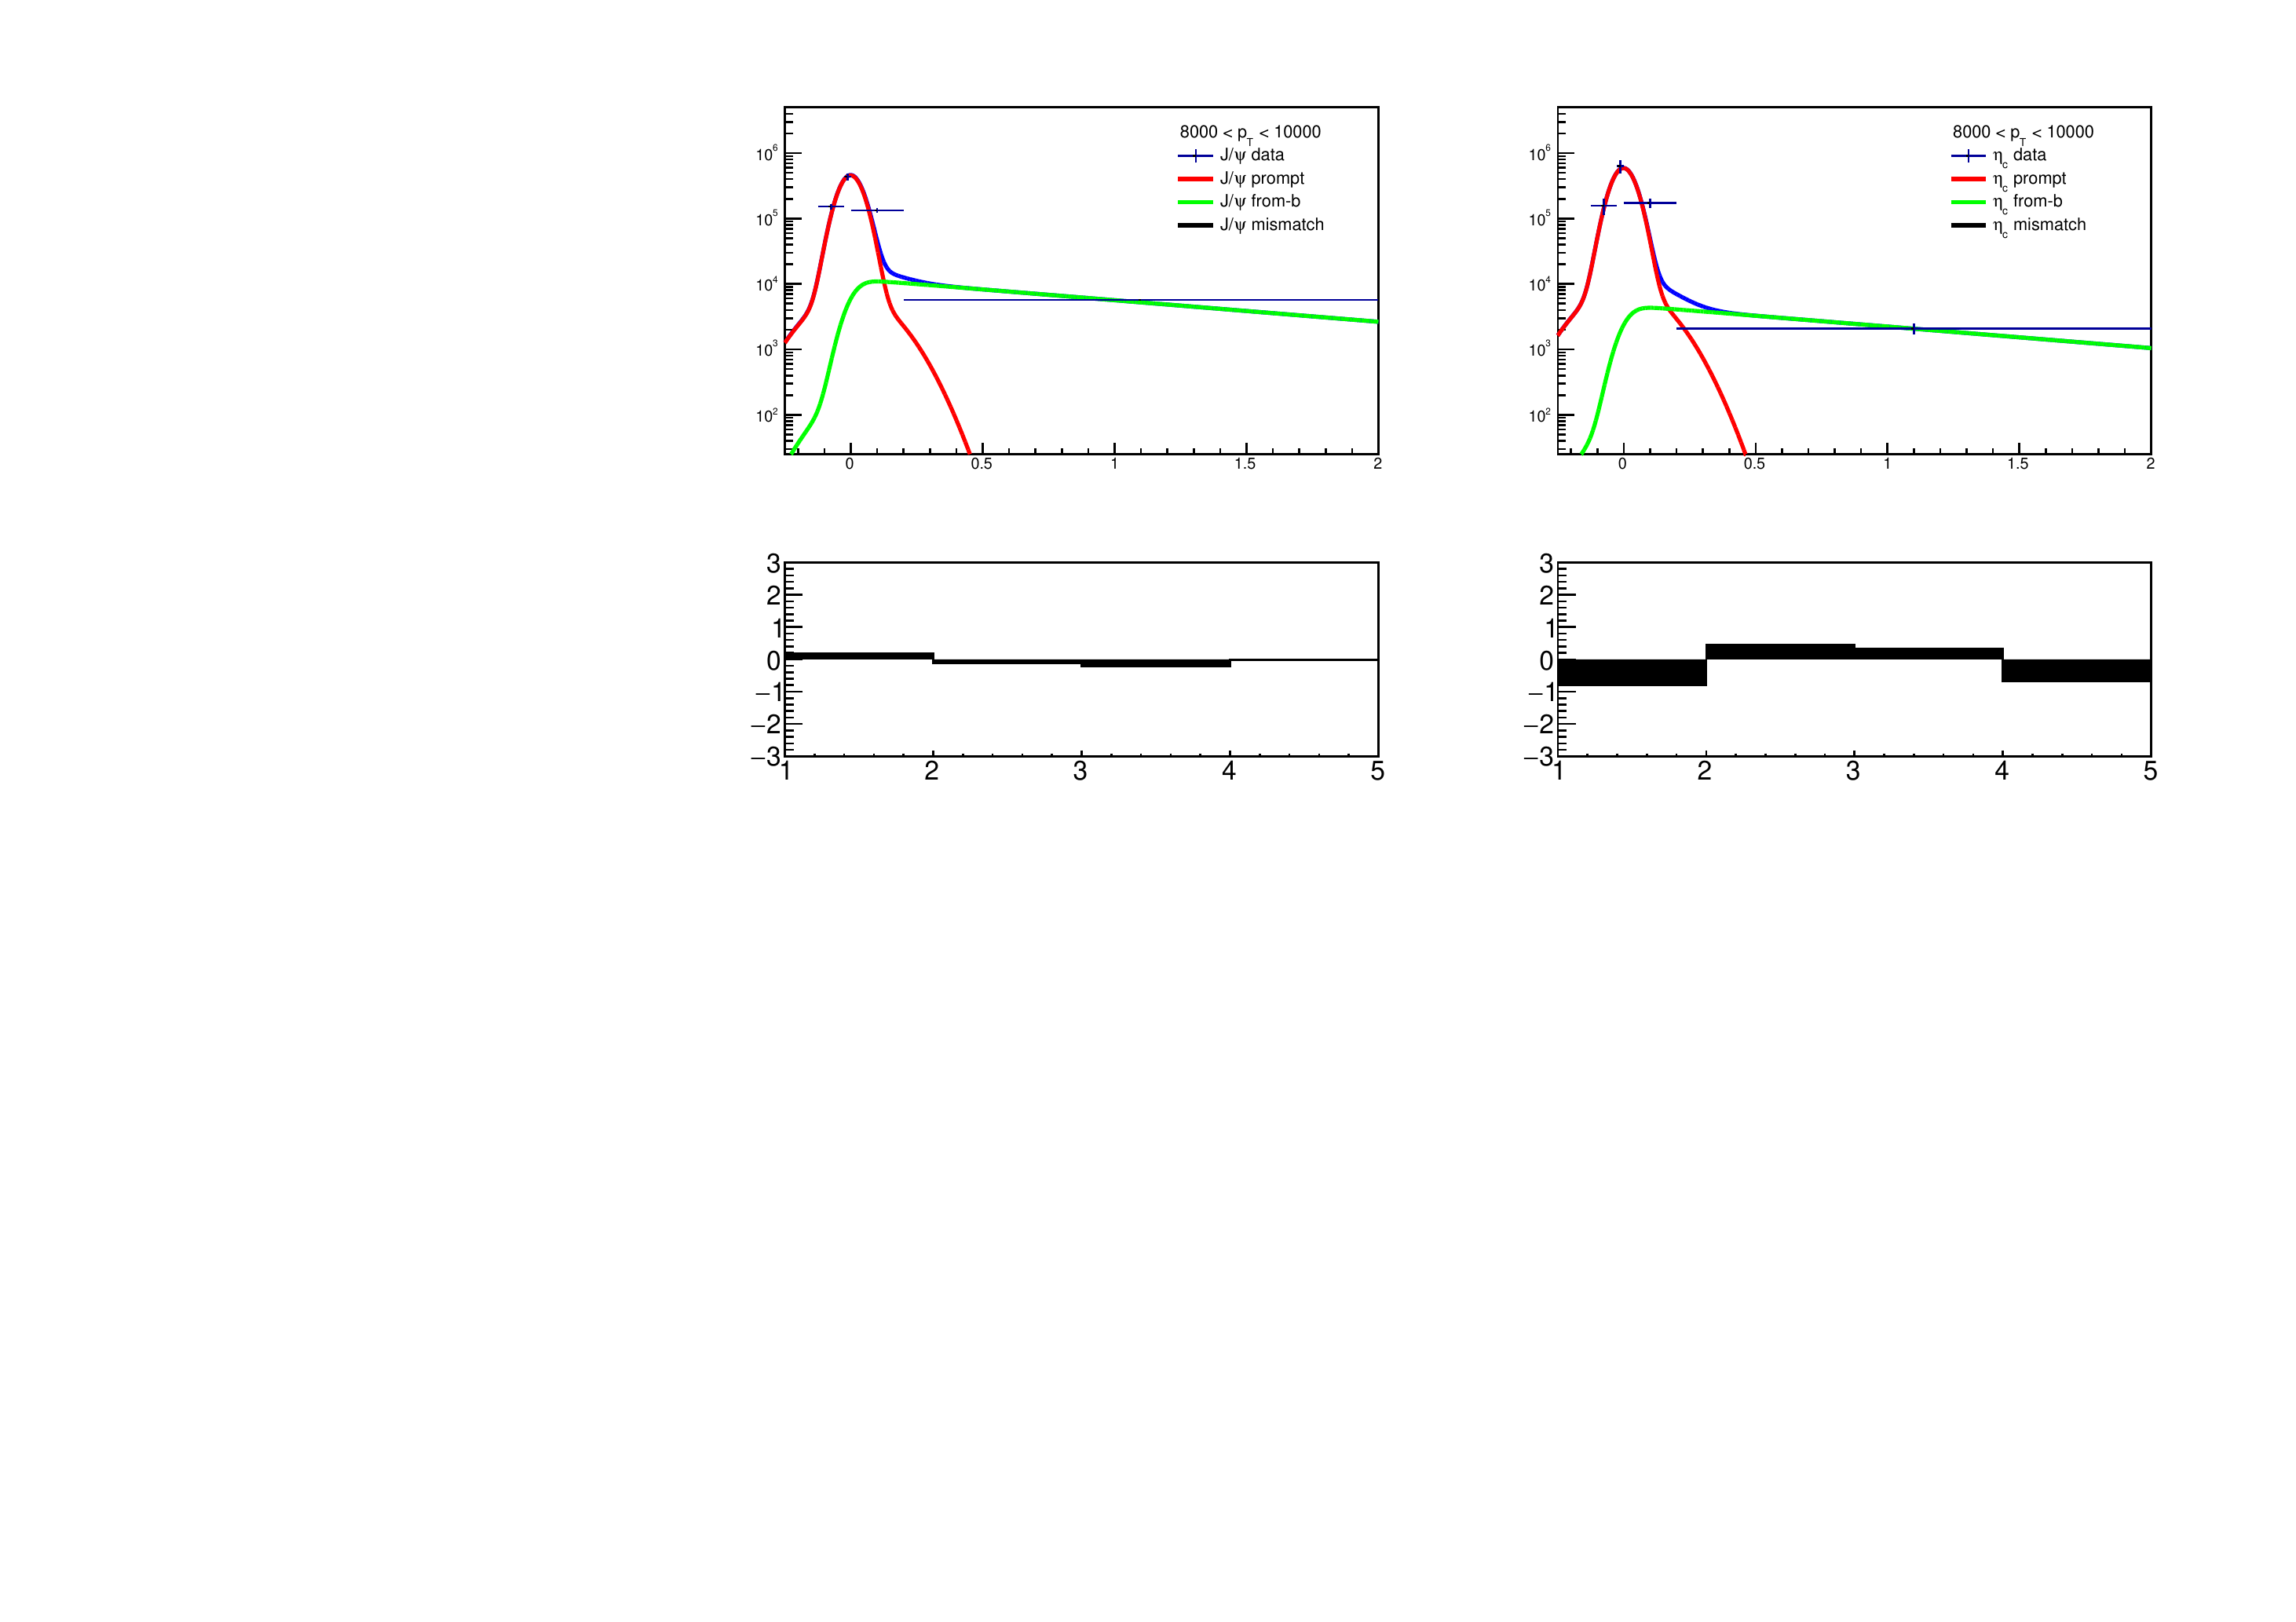}
\put(-46,-7){\scriptsize{$N(t_z)$}}
\put(-274,-7){\scriptsize{$N(t_z)$}}
\put(-192,185){\scriptsize{\lhcb preliminary}}
\put(-420,185){\scriptsize{\lhcb preliminary}}
\caption{The zoom of the $t_z$ distribution for \jpsi (left) and \etac (right) for $8.0 \gevc<\pt<10.0 \gevc$ and the result of simultaneous integral \chisq fit in all \pt bins. Red lines show prompt components, green lines show \etac and \jpsi from inclusive \bquark-decays, black lines show contributions from the events with wrongly associated PV. The corresponding pull distributions are shown below, where the $N(t_z)$ on the pull distributions denotes the $t_z$ bin number.} 
\label{fig:tzFitZoomPT2}
\end{figure}

\begin{figure}[ht]
\centering
\protect\protect\protect\includegraphics[width=0.9\textwidth]{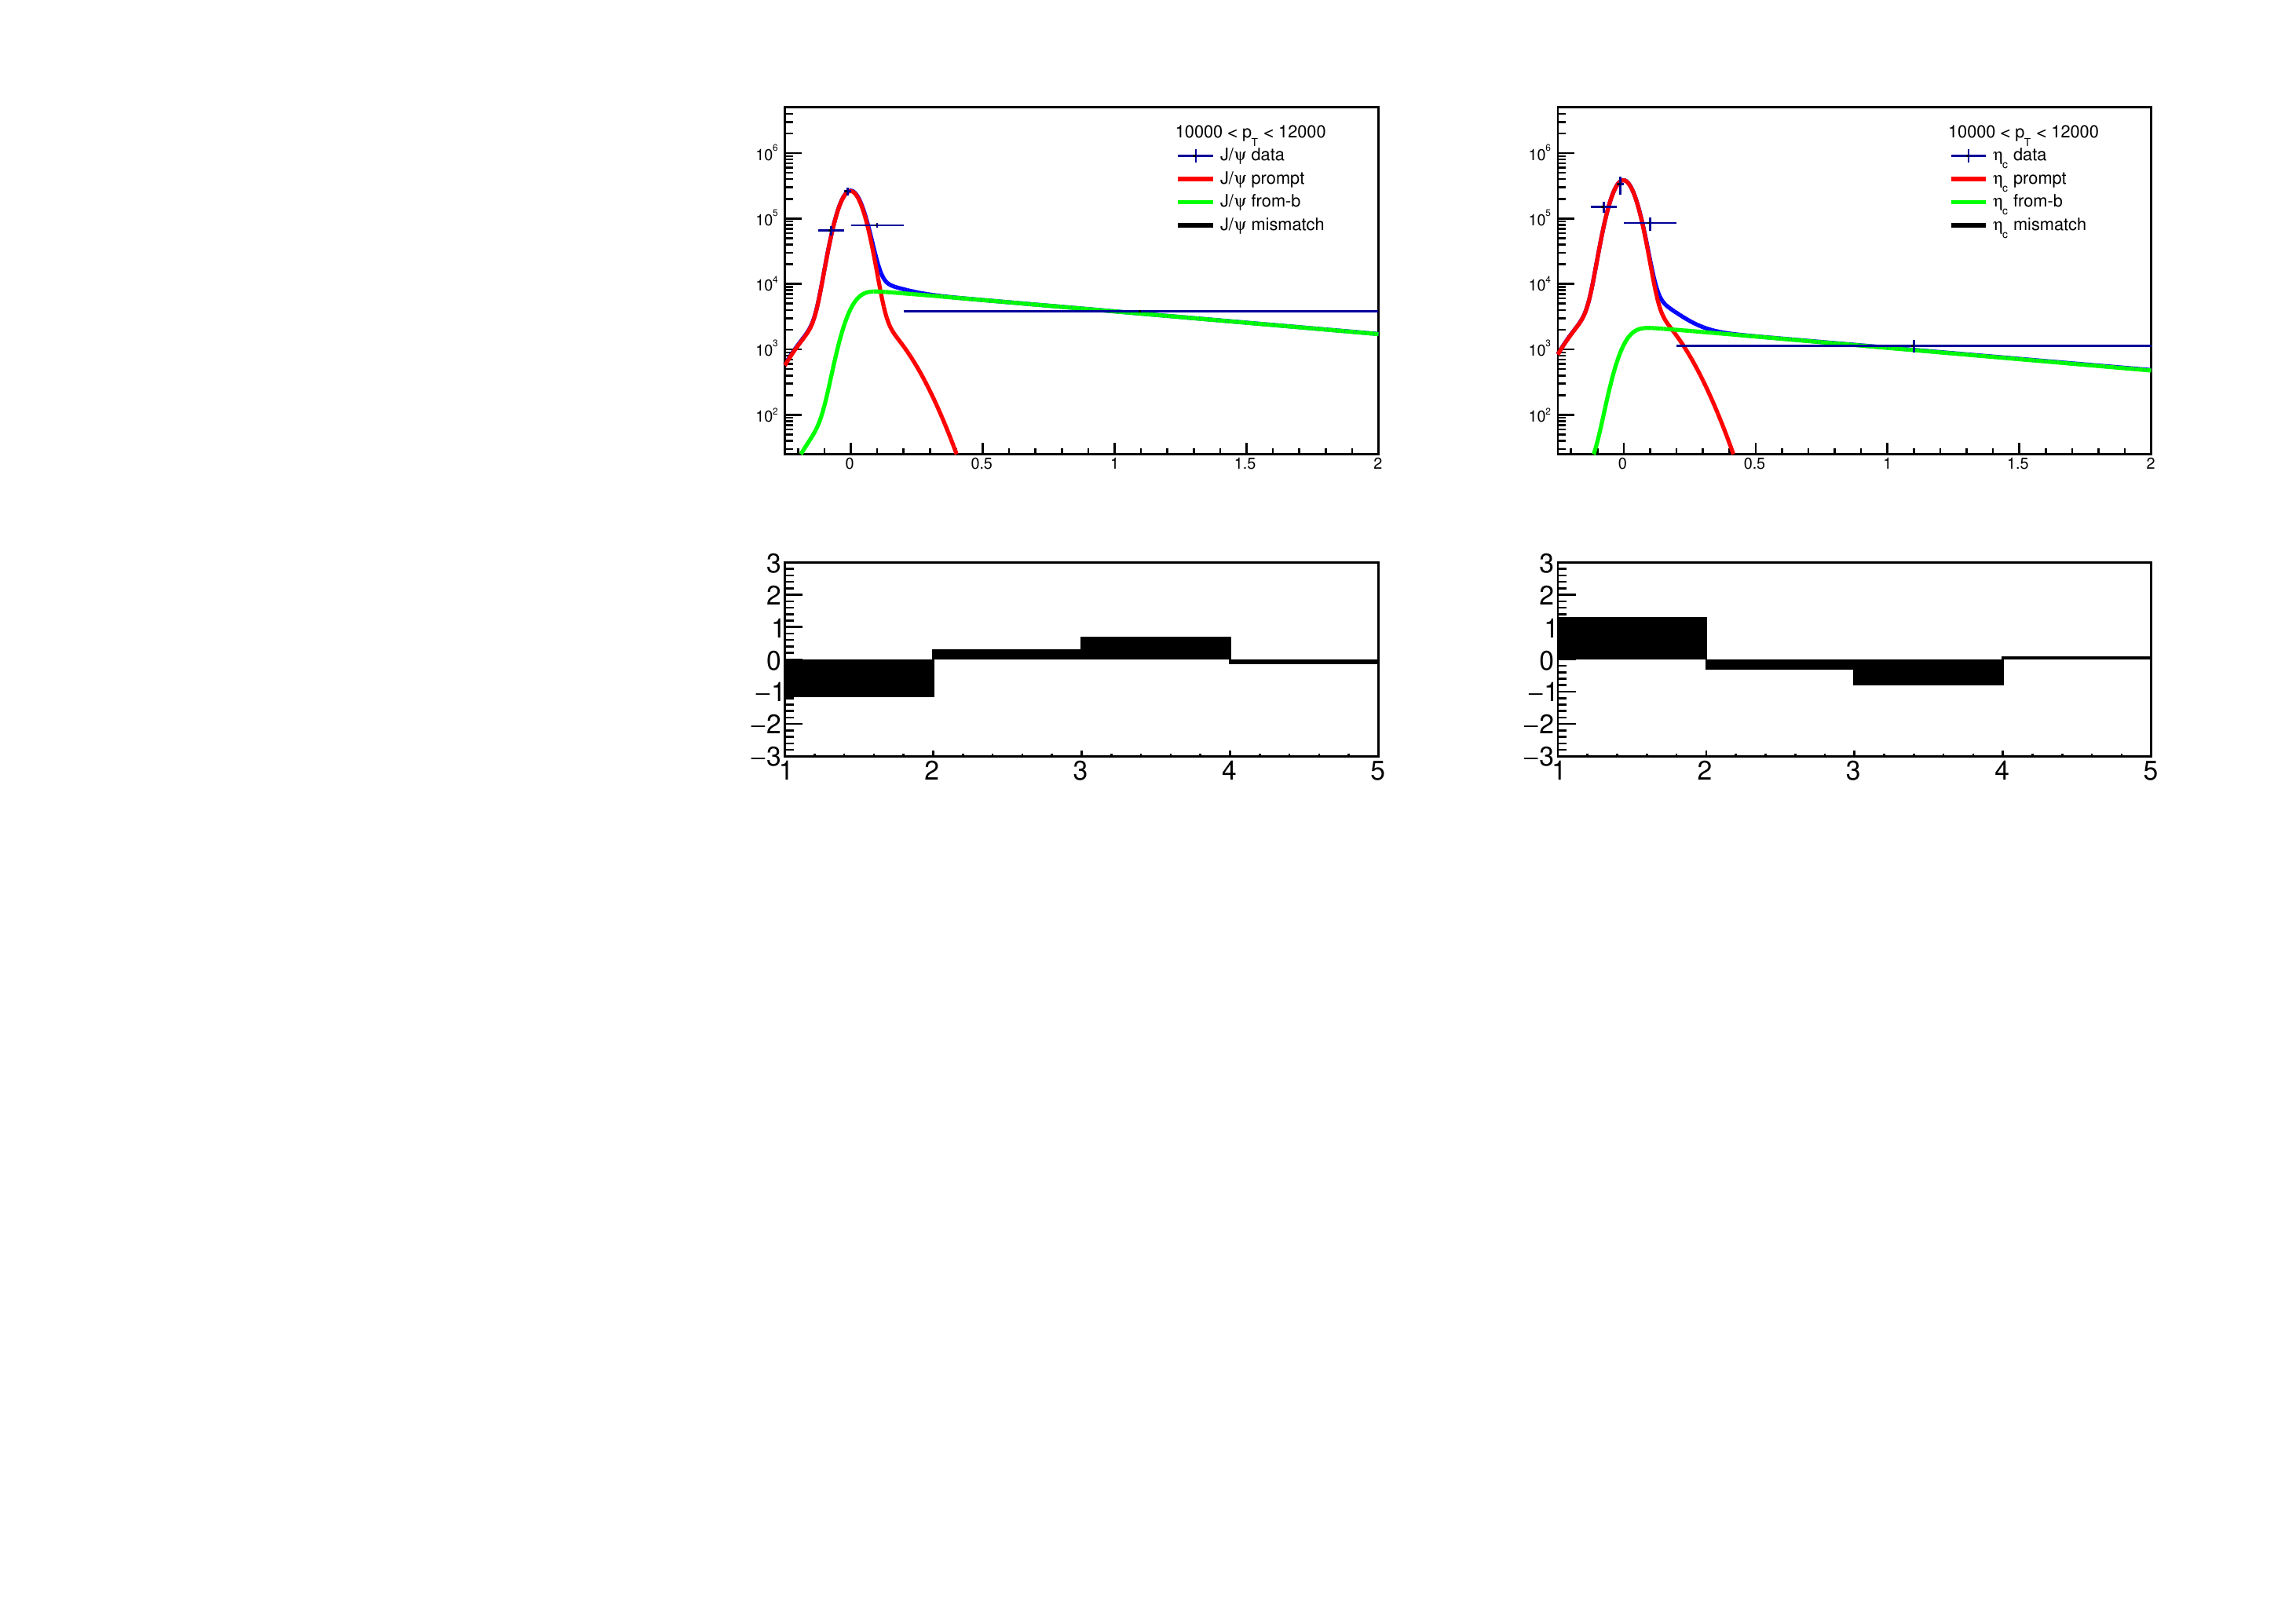}
\put(-46,-7){\scriptsize{$N(t_z)$}}
\put(-274,-7){\scriptsize{$N(t_z)$}}
\put(-192,185){\scriptsize{\lhcb preliminary}}
\put(-420,185){\scriptsize{\lhcb preliminary}}
\caption{The zoom of the $t_z$ distribution for \jpsi (left) and \etac (right) for $10.0 \gevc<\pt<12.0 \gevc$ and the result of simultaneous integral \chisq fit in all \pt bins. Red lines show prompt components, green lines show \etac and \jpsi from inclusive \bquark-decays, black lines show contributions from the events with wrongly associated PV. The corresponding pull distributions are shown below, where the $N(t_z)$ on the pull distributions denotes the $t_z$ bin number.} 
\label{fig:tzFitZoomPT3}
\end{figure}

\begin{figure}[ht]
\centering
\protect\protect\protect\includegraphics[width=0.9\textwidth]{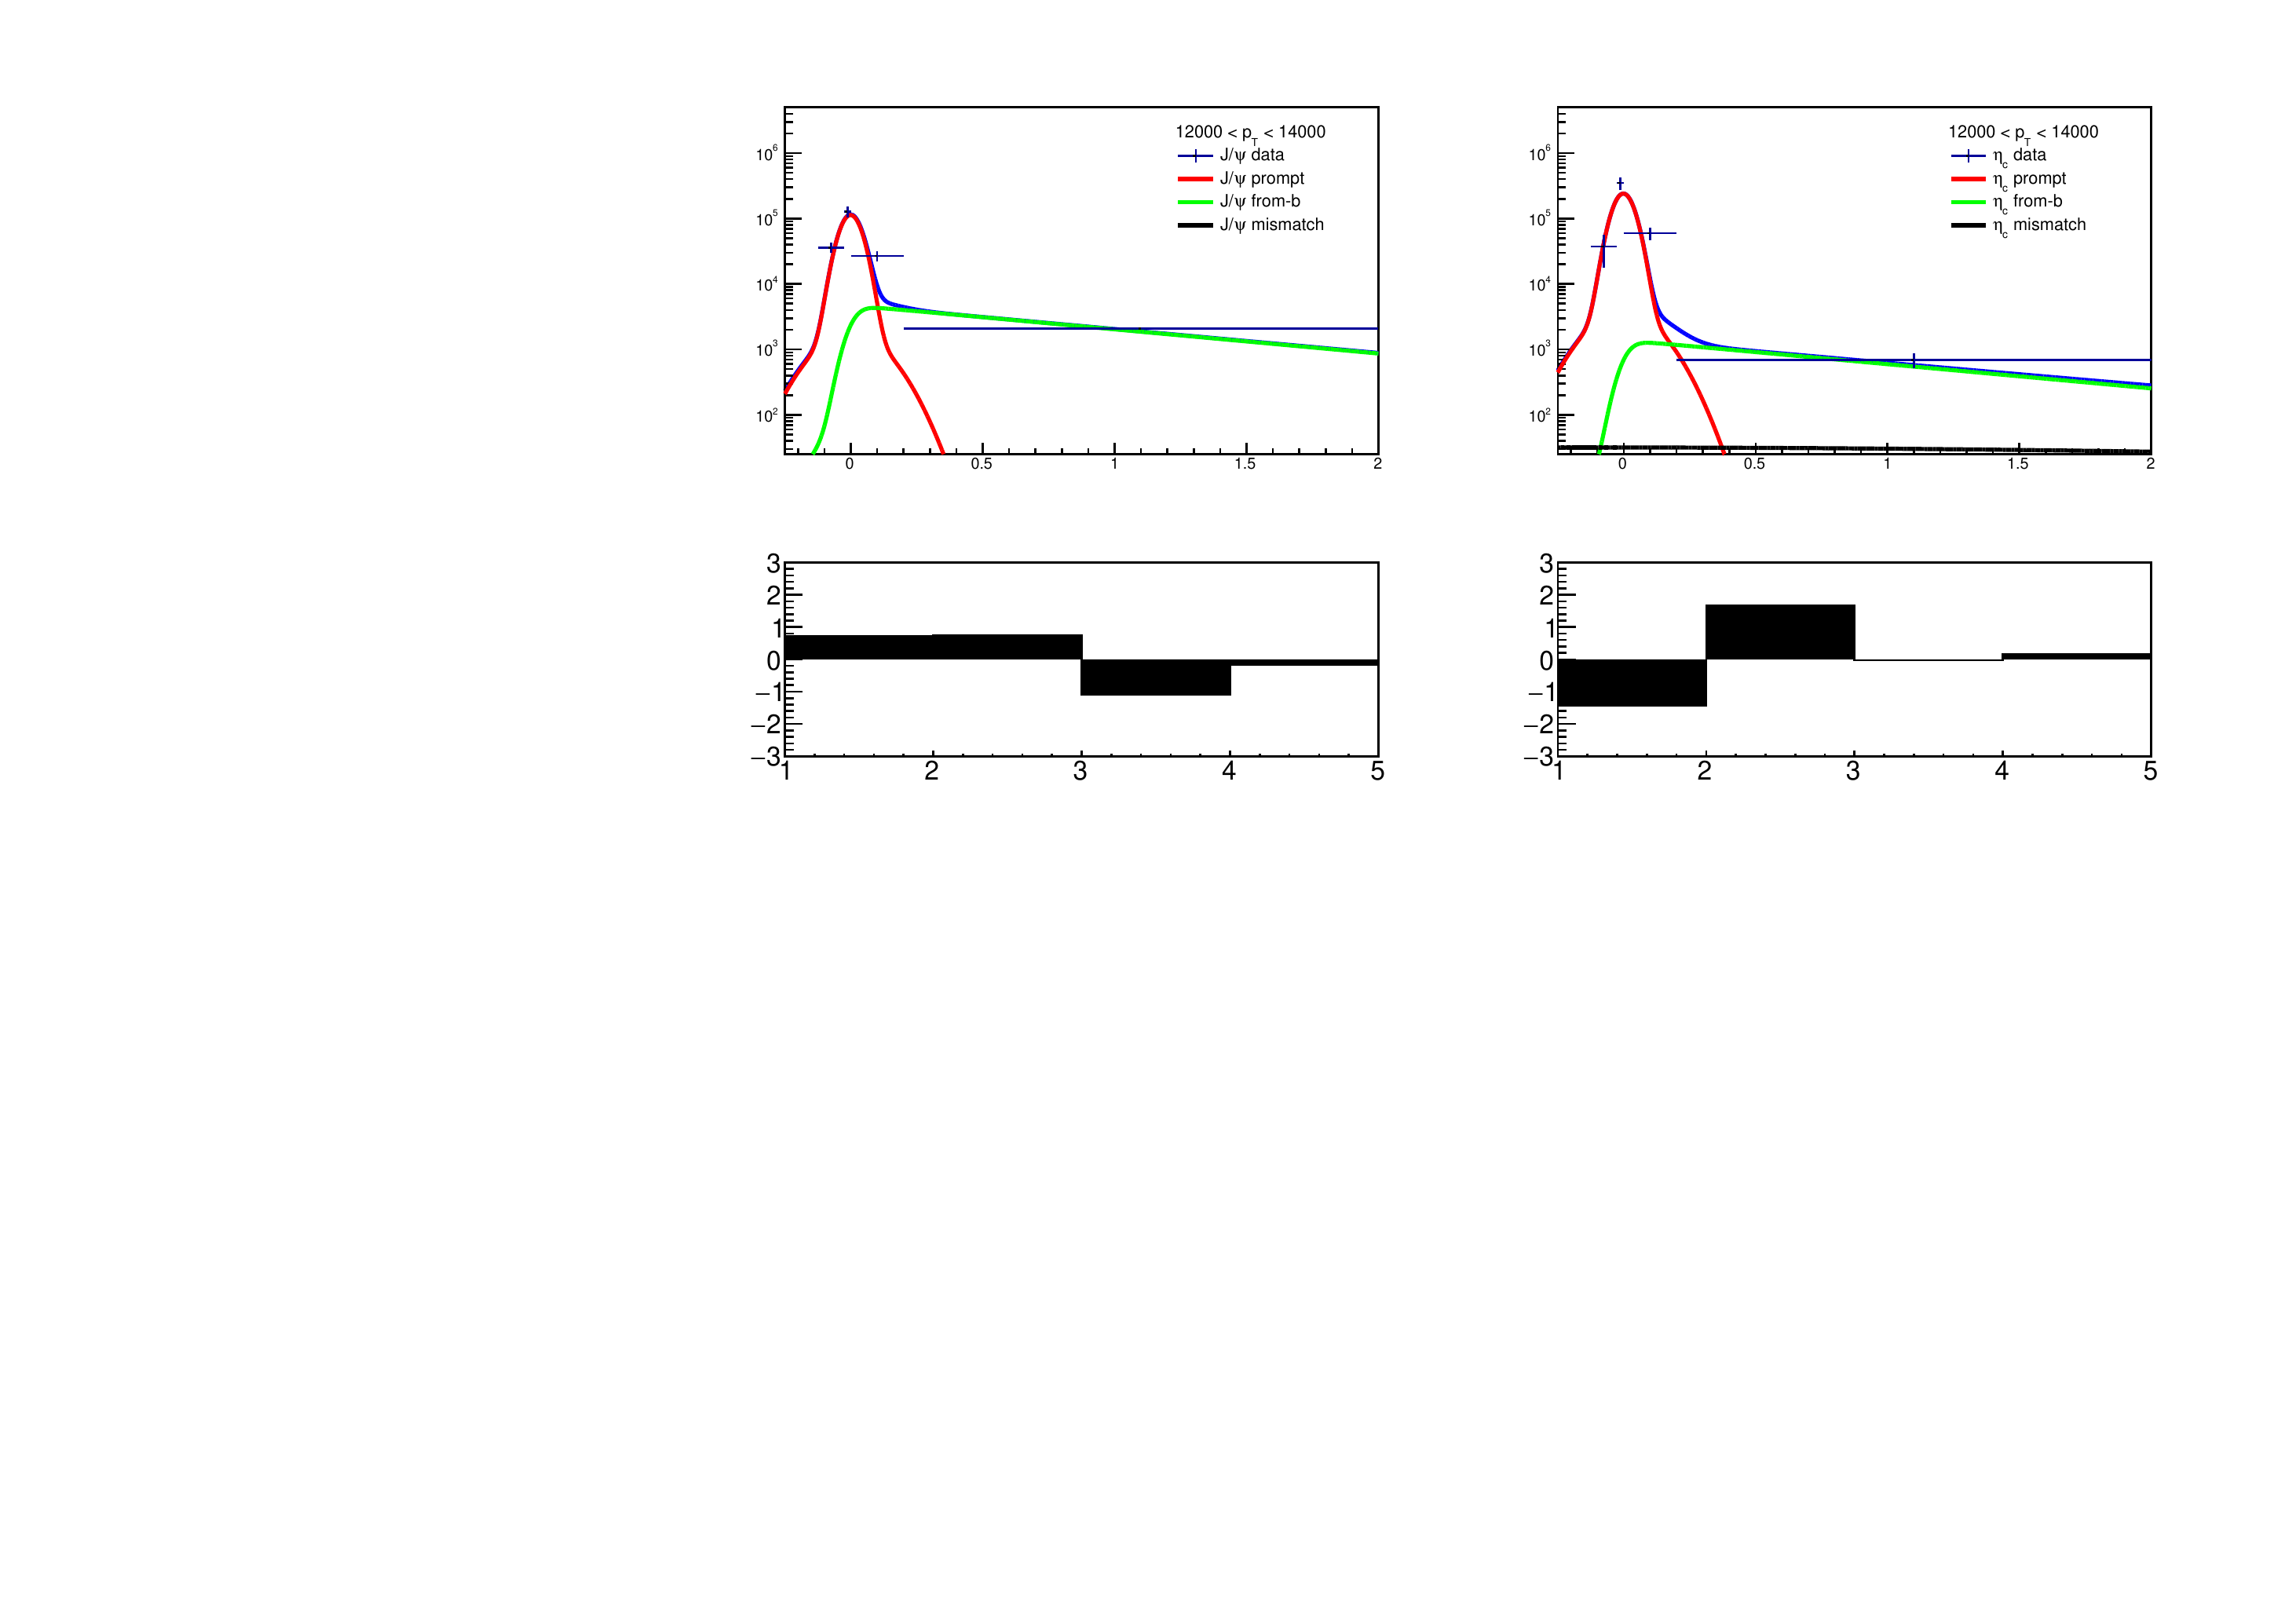}
\put(-46,-7){\scriptsize{$N(t_z)$}}
\put(-274,-7){\scriptsize{$N(t_z)$}}
\put(-192,185){\scriptsize{\lhcb preliminary}}
\put(-420,185){\scriptsize{\lhcb preliminary}}
\caption{The zoom of the $t_z$ distribution for \jpsi (left) and \etac (right) for $12.0 \gevc<\pt<14.0 \gevc$ and the result of simultaneous integral \chisq fit in all \pt bins. Red lines show prompt components, green lines show \etac and \jpsi from inclusive \bquark-decays, black lines show contributions from the events with wrongly associated PV. The corresponding pull distributions are shown below, where the $N(t_z)$ on the pull distributions denotes the $t_z$ bin number.} 
\label{fig:tzFitZoomPT4}
\end{figure}
\clearpage

\newpage
\section{Cross-check: possible interference impact on the \etac mass measurement}
\label{app:interference}
In this appendix we discuss possible impact of the interference of non-resonant \decay{\bquark}{\proton\antiproton X} S-wave decays and \decay{\bquark}{(\decay{\etac}{\proton\antiproton})X}. In this conservative estimate we describe the shape of the \etac peak together with background by the following expression:
\begin{equation}
	f_{[\decay{\bquark}{(\decay{\etac}{\proton\antiproton})X}]+[\decay{\bquark}{\proton\antiproton X}]+interf.} = |A_{RelBW(\etac)} + e^{i\cdot\phi}A_{non.res.}|^2,
\end{equation}
where $A_{RelBW(\etac)}$ is the Relativistic Breit-Wigner amplitude for \etac, $A_{non.res.}$ in the non-resonant amplitude of the \decay{\bquark}{\proton\antiproton X} decays, $\phi$ is the phase difference between the \etac and the non-resonant amplitudes.
The non-resonant amplitude is described by the empirical expression:
\begin{equation}
	A_{non.res.}=A+B\cdot e^{i\cdot \phi_B}\cdot M_{\ppbar} + C\cdot e^{i\cdot \phi_C}\cdot M_{\ppbar}^2,
\end{equation}
where $A$, $B$, $C$, $\phi_B$ and $\phi_C$ are real free fit parameters.

Distribution of invariant mass is shown on Fig.~\ref{fig:massTopoInterf}.
In general, fit yields a good description of $M_{\ppbar}$ distribution.
The fit gives the following value of the \jpsi and \etac mass difference to be $\Delta M _{\jpsi , \, \etac} = 113.87\pm0.64 \mev$. This result in agreement with the world average value $\Delta M _{\jpsi , \, \etac}^{PDG} = \etacMassDiffPDG$~\cite{PDG2017}.

\begin{figure}[h]
\centering
\protect\protect\protect\includegraphics[width=0.8\linewidth]{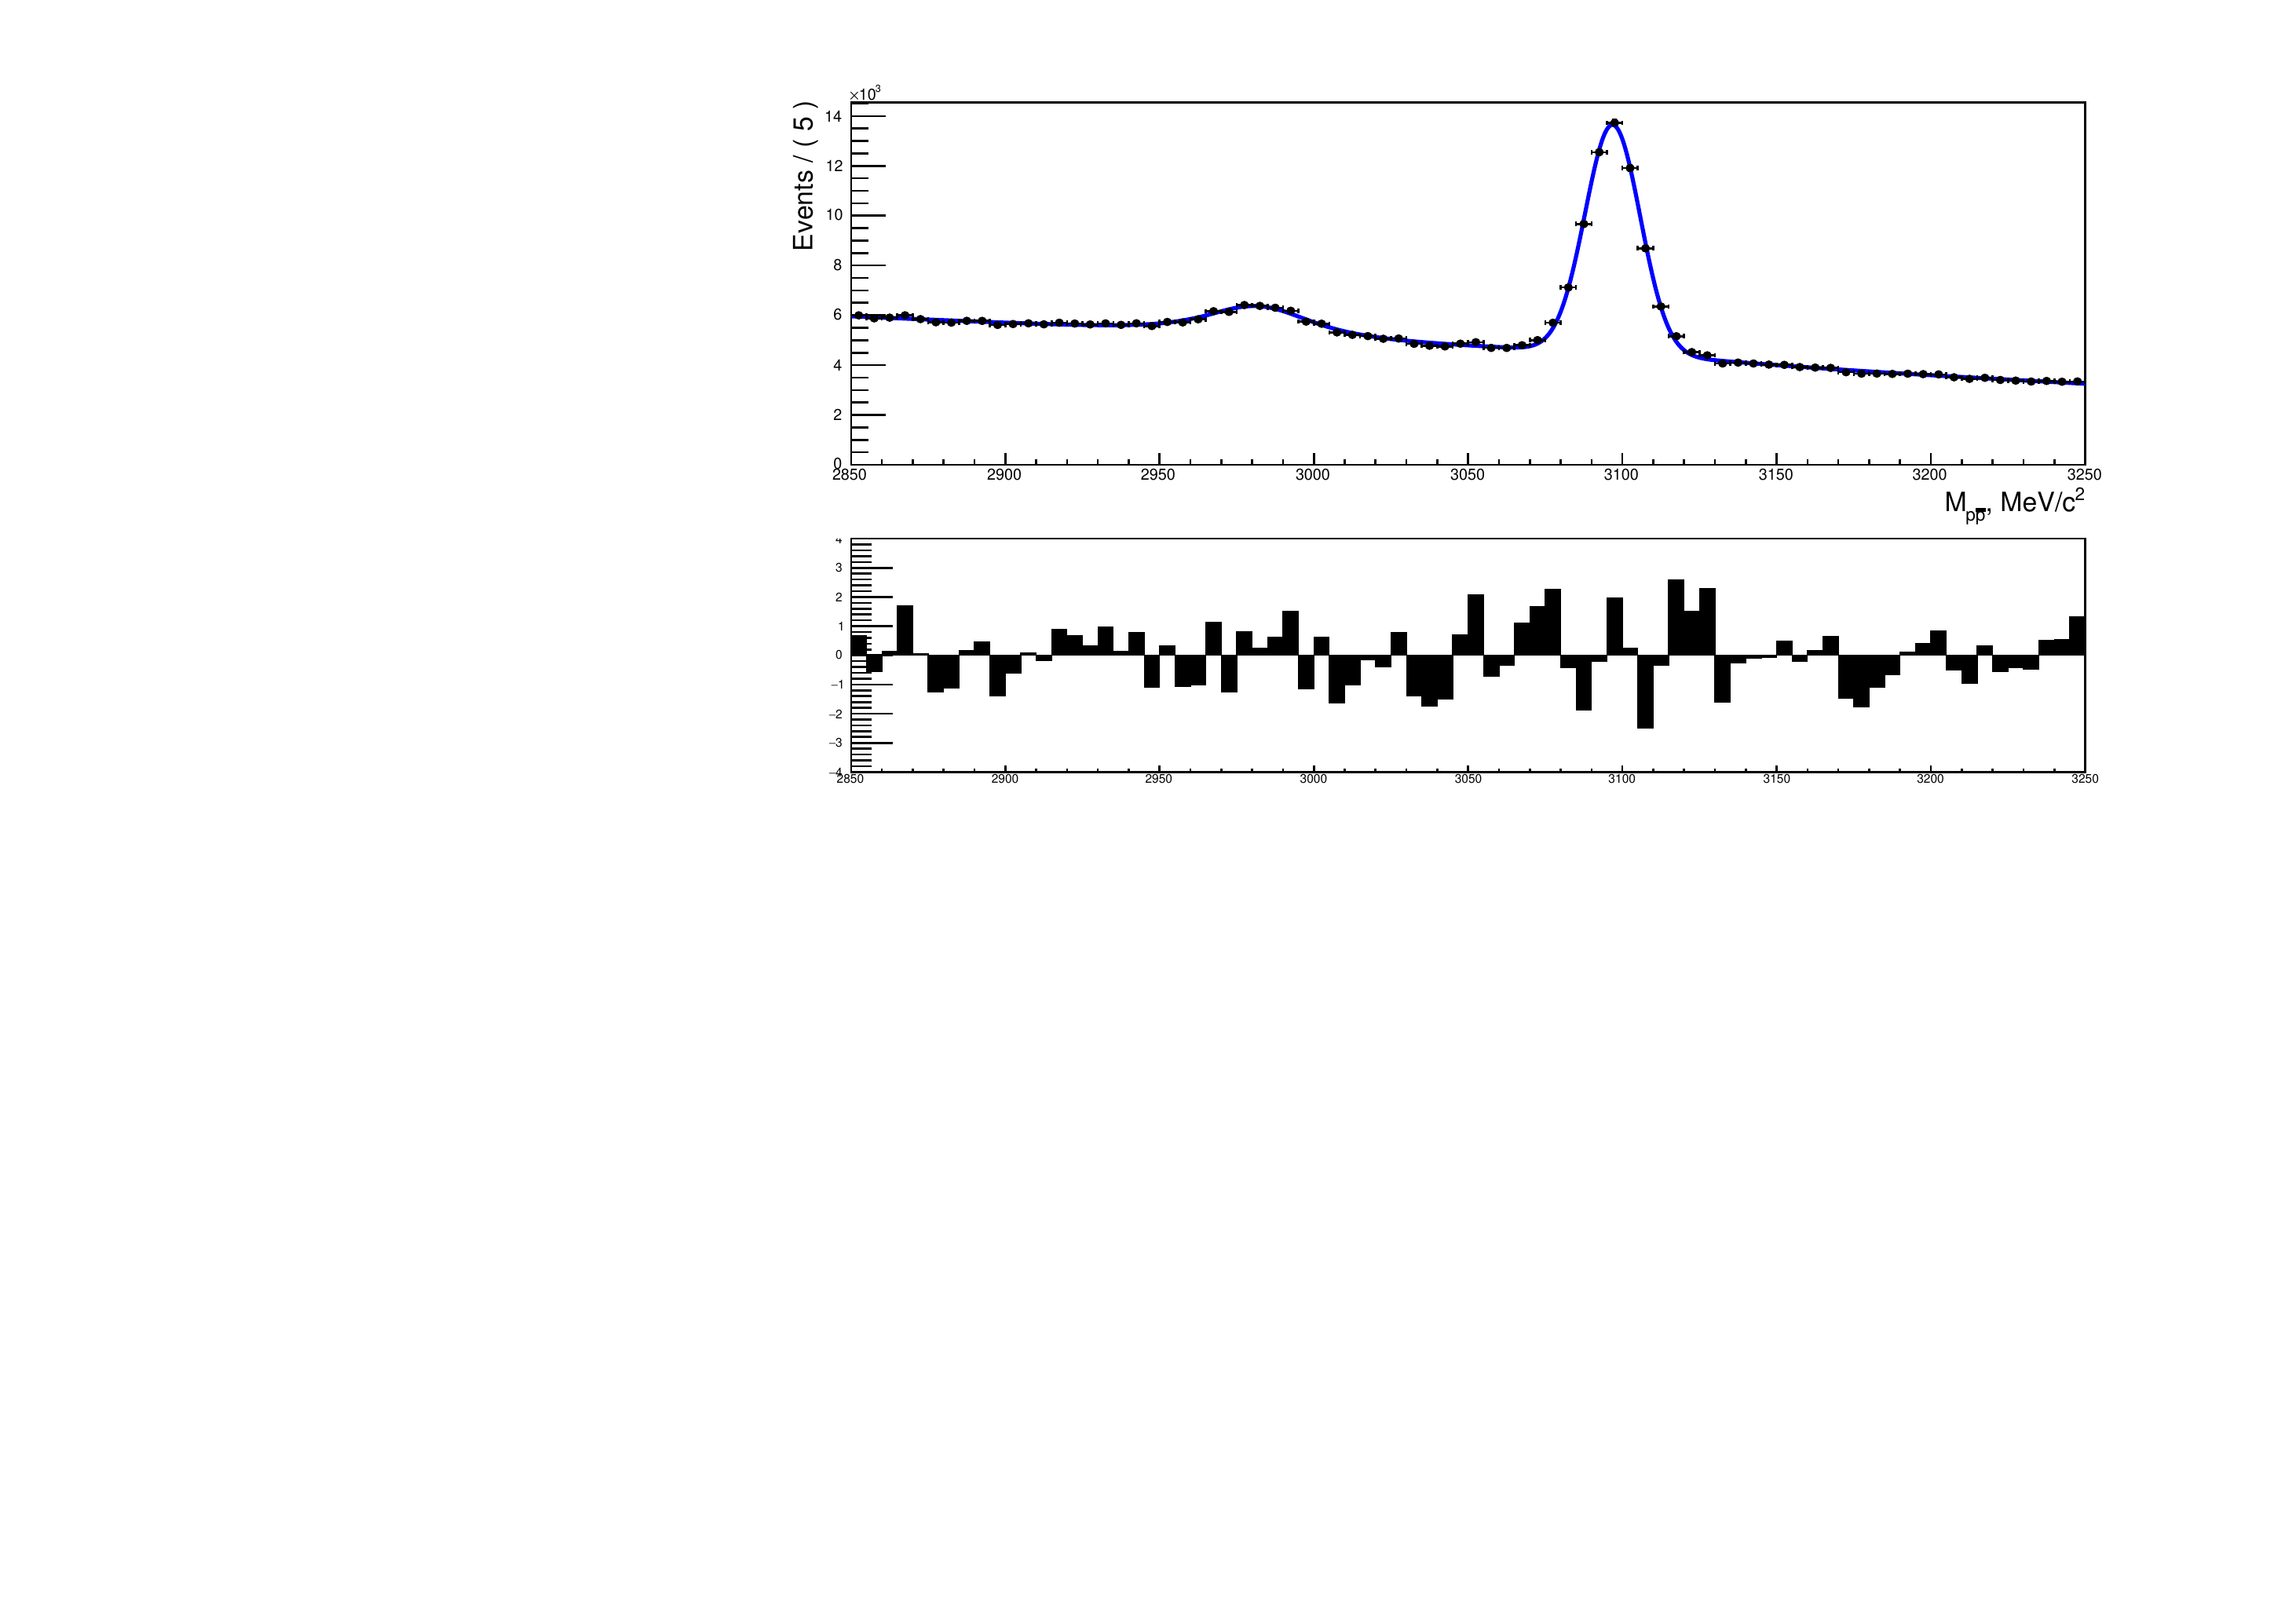}
\put(-310,150){\footnotesize{\lhcb preliminary}}
\caption{The distribution of $M_{\ppbar}$. The solid blues lines represent the fit result, which includes the possible interference contribution. The corresponding pull distributions are shown below each plot.} 
\label{fig:massTopoInterf}
\end{figure}
\clearpage

\newpage
\section{Cross-check: comparison of the $\tau_b$ parameter for \etac and \jpsi and its impact on the production measurement}
\label{app:taubEtacJpsi}

Values of $\tau_b$ parameter are expected to be the same for \etac and \jpsi. This is in agreement with the fact that simultaneous fit with common $\tau_b$ parameter for \etac and \jpsi well describes $t_z^{TRUE}$ distributions in the MC samples.

In general, \Bz, \Bs and $\Lambda_b$ lifetimes are close to 1.5 \ps within 2\% accuracy, which is better than the statistical precision of the $\tau_b$ parameter from the fit to the $t_z$ distribution in data. Only the \Bp meson has significantly different lifetime of 1.64 \ps. A systematic shift can then impact the results only in case if \Bp fraction contributing to the observed inclusive \bquark-decays to \etac is significantly different from that to \jpsi. These considerations allow to perform a very conservative cross-check described below. The upper limit of the possible impact corresponds to a difference between the $\tau_b$ for \etac and \jpsi of 5\%, estimated from the lifetimes of different \bquark-species and the corresponding fragmentation fractions. 

Also, the fit to data with $\tau_b$ as free fit parameters - two different parameters for \etac and \jpsi - is consistent with the same $\tau_b$ values for \etac and \jpsi and also with a 5\% difference, given a large uncertainty of the $\tau_b$ value for \etac: 
\begin{equation}
\begin{aligned}
\tau_b^{\jpsi}   &=  1.28 \pm  0.03 \ps \\
\tau_b^{\etac}   &=  1.19 \pm  0.12 \ps. 
\end{aligned}
\label{eq:differentTaubFit}
\end{equation}

In the cross-check, a fit to $t_z$ was performed using the $\tau_b$ values different by 5\% for the \etac and the \jpsi. The results on the yield ratios in the \pt bins are shown in Tab.~\ref{tab:taubXcheckPrompt} for  prompt production and in Tab.~\ref{tab:taubXcheckFromB} for production in \bquark-decays. They are consistent with the baseline fit well within statistical uncertainties. 

\begin{table}[ht]
\centering
\small
\begin{tabular}{c|c|c} 
\pt-range 						& Baseline fit  & Fit with 5\% difference between       \\
         					    &               & $\tau_b^{\etac}$ and $\tau_b^{\jpsi}$ \\ \hline
$6.5 \gevc < \pt < 8.0  \gevc$  & $1.08 \pm 0.21$ & $1.08 \pm 0.21$ \\
$8.0 \gevc < \pt < 10.0 \gevc$  & $1.29 \pm 0.18$ & $1.29 \pm 0.18$ \\
$10.0\gevc < \pt < 12.0 \gevc$  & $1.46 \pm 0.23$ & $1.47 \pm 0.23$ \\
$12.0\gevc < \pt < 14.0 \gevc$  & $2.13 \pm 0.40$ & $2.12 \pm 0.40$
\end{tabular} 
\caption{The comparison of the yield ratio $N_{\etac}^{prompt}/N_{\jpsi}^{prompt}$ of prompt charmonia in bins of \pt for baseline fit and for the fit assuming 5\% difference for $\tau_b^{\etac}$ and $\tau_b^{\jpsi}$.}
\label{tab:taubXcheckPrompt}
\end{table}

\begin{table}[ht]
\centering
\small
\begin{tabular}{c|c|c} 
\pt-range 						& Baseline fit    & Fit with 5\% difference between       \\
         					    &                 & $\tau_b^{\etac}$ and $\tau_b^{\jpsi}$ \\ \hline
$6.5 \gevc < \pt < 8.0  \gevc$  & $0.281 \pm 0.071$ & $0.263 \pm 0.068$ \\
$8.0 \gevc < \pt < 10.0 \gevc$  & $0.396 \pm 0.047$ & $0.383 \pm 0.046$ \\
$10.0\gevc < \pt < 12.0 \gevc$  & $0.277 \pm 0.052$ & $0.270 \pm 0.051$ \\
$12.0\gevc < \pt < 14.0 \gevc$  & $0.293 \pm 0.073$ & $0.289 \pm 0.073$
\end{tabular} 
\caption{The comparison of the yield ratio $N_{\etac}^{b-decays}/N_{\jpsi}^{b-decays}$ of charmonia from \bquark-decays in bins of \pt for baseline fit and for the fit assuming 5\% difference for $\tau_b^{\etac}$ and $\tau_b^{\jpsi}$.}
\label{tab:taubXcheckFromB}
\end{table}

\clearpage

\newpage
\section{Comparison of the separation cut efficiencies from data and MC}
\label{app:tzcutEff_dataVSmc}

A good agreement between data and MC in $t_z$ distribution is guaranteed by the fact that all parameters of $t_z$-resolution model and $\tau_b$ are in good agreement between data and MC. 
To extract the efficiency of $t_z<80 \fs$$(>80 \fs)$ requirement from data one can use and integrate the curve of the fit to $t_z$ from \tzfit. The comparison of the efficiency of this cut from data and MC is shown in the Tab.~\ref{tab:tzcutEffTab}. The values are well consistent within the uncertainty due to MC sample sizes.
\begin{table}[ht]
\centering
\small
\begin{tabular}{c|c|c} 
        						      & from \tzfit                            & MC                \\ \hline
$\eps^{\jpsi, prompt  }(t_z<80 \fs)$  & $0.955 \pm 0.003_{(stat. uncorrelated)}$ & $0.964 \pm 0.011$ \\
$\eps^{\jpsi, b-decays}(t_z>80 \fs)$  & $0.938 \pm 0.002_{(stat. uncorrelated)}$ & $0.936 \pm 0.016$
\end{tabular} 
\caption{Comparison of the $t_z<80 \fs$$(>80 \fs)$ requirement efficiency from data and MC for prompt charmonia and charmonia from \bquark-decays}
\label{tab:tzcutEffTab}
\end{table}

The requirement on proton $IP\,\chisq$ is also used in the analysis with \tzcut. Its efficiency enters to definition of $\eps^{P \to b}$ and $\eps^{b \to b}$.
The $IP\,\chisq$ variable is known to be well described by MC. The cross-talk described by $\eps^{P \to b}$ is small and the contamination of \bquark-decays sample by prompt \etac is about 1.5\% (about 0.4\% for \jpsi), which was estimated using known \etac prompt yield from \tzfit. The effect of this cross-talk is also checked by setting $\eps^{P \to b}\equiv 0$, which does not lead to change in $N^{prompt}_{\etac}/N^{prompt}_{\jpsi}$ and $N^{b-decays}_{\etac}/N^{b-decays}_{\jpsi}$ at 1\% level.

Since the contamination of \bquark-decays sample by prompt candidates is small, one can evaluate the value of $\eps^{b \to b}$ from data by comparing a signal yield in \bquark-decays sample and total number of signal from \bquark-decays obtained from \tzfit. The comparison between data and MC values is shown in Tab.~\ref{tab:tzcutEffb2bTab}.
\begin{table}[ht]
\centering
\small
\begin{tabular}{c|c|c} 
        		 & from \tzfit and \tzcut      & MC                \\ \hline
$\eps^{b \to b}$  & $0.699 \pm 0.076_{(stat)}$  & $0.692 \pm 0.013$ \\
\end{tabular} 
\caption{Comparison of the $\eps^{b \to b}$ requirement efficiency from data and MC.}
\label{tab:tzcutEffb2bTab}
\end{table}

From all above we conclude that all the considered issues are well within the actual estimate of the cross-talk uncertainty.
\clearpage
